# Supplementary material for: A Connect Sum Formula for the BPS Invariant of Knot Complements
Source: arXiv:2109.14021 ancillary file (2021-09-28)
Supplement: Supplementary file 1 [file README.pdf]

## Details of the recursions

This is a list of the coefficient functions in the recursion relations (6), (7) and (8), respectively, in [1].

$$\begin{aligned} t_0 = & q^2 - q^4 x + q^2 (-q^3 + q^4 - q^6 - q^7) x^2 + q^2 (q^5 - q^6 + q^8 + q^9) x^3 \\ & + q^2 (-q^7 + q^8 + q^9 - q^{11} + q^{13}) x^4 + q^2 (-q^{10} + q^{13} - q^{15}) x^5 \\ & + q^2 (q^{12} - q^{15} - q^{16} + q^{17}) x^6 + q^2 (q^{17} - q^{19}) x^7 \\ & + q^2 (-2q^{19} + q^{21}) x^8 + q^{23} x^9 + 2q^{28} x^{10} - 2q^{30} x^{11} - q^{35} x^{12} + q^{37} x^{13} \end{aligned}$$

$$\begin{aligned} t_1 = & -1 + q^2 x + (2q - q^3 - q^4 + q^6 + q^7) x^2 + (q^2 - 2q^3 + q^5 + q^6 - q^8 - q^9) x^3 \\ & + (-q^2 + q^4 + 2q^5 - q^6 - 3q^7 - 3q^8 + q^9 + 2q^{10} + q^{11} - q^{13}) x^4 \\ & + (-q^3 + 2q^4 - q^6 - 2q^7 + 2q^9 + 3q^{10} - q^{11} - 2q^{12} - q^{13} + q^{15}) x^5 \\ & + (-2q^6 + 2q^7 + 2q^8 + 2q^9 - 2q^{10} - 4q^{11} - 2q^{12} + 2q^{13} + 4q^{14} + q^{15} - q^{16} - q^{17}) x^6 \\ & + (-q^5 + 2q^8 - q^9 - 2q^{10} - 3q^{11} + 2q^{12} + 4q^{13} + 2q^{14} - q^{15} - 4q^{16} - q^{17} + q^{18} + q^{19}) x^7 \\ & + (-q^6 + q^7 - q^8 + 2q^{11} + 2q^{12} + 2q^{13} - 4q^{14} - 4q^{15} - q^{16} + 3q^{17} + 4q^{18} - q^{20} - q^{21}) x^8 \\ & + (q^8 - q^9 + q^{10} + q^{11} + q^{12} - 2q^{13} - 2q^{14} - 2q^{15} + 3q^{16} + 5q^{17} + q^{18} - 3q^{19} - 4q^{20} + q^{22} + q^{23}) x^9 \\ & + (q^9 - q^{10} + q^{13} - q^{14} + 2q^{15} + q^{16} - 4q^{18} - 4q^{19} + 3q^{21} + 3q^{22} - q^{24} - q^{25}) x^{10} \\ & + (-q^{11} + q^{12} - q^{15} + q^{16} - 2q^{17} - 2q^{18} + 4q^{20} + 3q^{21} - 3q^{23} - 3q^{24} + q^{26} + q^{27}) x^{11} \\ & + (q^{13} - q^{14} - q^{15} + q^{17} + q^{19} + q^{20} - 3q^{22} - 2q^{23} + 3q^{25} + 3q^{26} - q^{28} - q^{29}) x^{12} \\ & + (q^{16} - q^{19} - q^{21} + 2q^{24} + 2q^{25} - 3q^{27} - q^{28} + q^{30} + q^{31}) x^{13} \\ & + (-q^{18} + q^{21} + q^{22} - 2q^{26} - 2q^{27} + 3q^{29} + q^{30} - q^{32} - q^{33}) x^{14} \\ & + (-q^{23} + q^{25} + 2q^{28} - q^{31} - q^{32} + q^{34}) x^{15} + (2q^{25} - q^{27} - 2q^{30} + q^{33} + q^{34} - q^{36}) x^{16} \\ & + (-q^{27} - q^{35}) x^{17} + (-2q^{32} + q^{37}) x^{18} + 2q^{34} x^{19} + q^{39} x^{20} - q^{41} x^{21} \end{aligned}$$

$$\begin{aligned} t_2 = & -q^3 x^3 + q^5 x^4 + q^3 (2q - q^4 - q^5 + q^7) x^5 + q^3 (-2q^3 + q^6 + q^7 - q^9) x^6 \\ & + q^3 (-q^2 + 2q^5 + 2q^6 - 3q^8 - q^9 + q^{11} + q^{12}) x^7 + q^3 (2q^4 - 2q^7 - 2q^8 + q^9 + 3q^{10} + q^{11} - q^{13} - q^{14}) x^8 \\ & + q^3 (-2q^6 - q^7 + 3q^9 + 2q^{10} - q^{11} - 3q^{12} - 3q^{13} + q^{15} + q^{16}) x^9 \\ & + q^3 (-q^5 - q^7 + 2q^8 + 2q^9 - 2q^{10} - 4q^{11} - 2q^{12} + q^{13} + 3q^{14} + 2q^{15} - q^{16} - q^{17} - q^{18}) x^{10} \\ & + q^3 (q^7 + q^9 - 2q^{10} - 2q^{11} + 2q^{12} + 4q^{13} + 3q^{14} - q^{15} - 3q^{16} - 2q^{17} + q^{18} + q^{19} + q^{20}) x^{11} \\ & + q^3 (q^8 - q^9 - q^{10} + 2q^{12} + q^{13} - 2q^{15} - 2q^{16} + 2q^{17} + 2q^{18} + 2q^{19} - q^{20} - q^{21}) x^{12} \\ & + q^3 (-q^{10} + q^{11} + q^{12} - 2q^{13} - 2q^{14} - q^{15} + 4q^{17} + 2q^{18} - 2q^{19} - 2q^{20} - 2q^{21} + q^{22} + q^{23}) x^{13} \\ & + q^3 (q^{12} - q^{16} + q^{18} - q^{22}) x^{14} + q^3 (q^{14} - q^{18} + q^{20} - q^{24}) x^{15} \\ & + q^3 (-q^{16} + q^{17} + q^{18} - 2q^{19} - 2q^{20} - q^{21} + 4q^{23} + 2q^{24} - 2q^{25} - 2q^{26} - 2q^{27} + q^{28} + q^{29}) x^{16} \\ & + q^3 (q^{18} - q^{19} - q^{20} + 2q^{22} + q^{23} - 2q^{25} - 2q^{26} + 2q^{27} + 2q^{28} + 2q^{29} - q^{30} - q^{31}) x^{17} \end{aligned}$$

$$\begin{aligned}
& + q^3 (q^{21} + q^{23} - 2q^{24} - 2q^{25} + 2q^{26} + 4q^{27} + 3q^{28} - q^{29} - 3q^{30} - 2q^{31} + q^{32} + q^{33} + q^{34}) x^{18} \\
& + q^3 (-q^{23} - q^{25} + 2q^{26} + 2q^{27} - 2q^{28} - 4q^{29} - 2q^{30} + q^{31} + 3q^{32} + 2q^{33} - q^{34} - q^{35} - q^{36}) x^{19} \\
& + q^3 (-2q^{28} - q^{29} + 3q^{31} + 2q^{32} - q^{33} - 3q^{34} - 3q^{35} + q^{37} + q^{38}) x^{20} \\
& + q^3 (2q^{30} - 2q^{33} - 2q^{34} + q^{35} + 3q^{36} + q^{37} - q^{39} - q^{40}) x^{21} \\
& + q^3 (-q^{32} + 2q^{35} + 2q^{36} - 3q^{38} - q^{39} + q^{41} + q^{42}) x^{22} \\
& + q^3 (-2q^{37} + q^{40} + q^{41} - q^{43}) x^{23} + q^3 (2q^{39} - q^{42} - q^{43} + q^{45}) x^{24} \\
& + q^{47} x^{25} - q^{49} x^{26}
\end{aligned}$$

$$\begin{aligned}
t_3 = & -q^{15} x^8 + q^{17} x^9 + 2q^{16} x^{10} - q^{15} (2q^3 - q^8) x^{11} - q^{15} (q^2 + q^{10}) x^{12} \\
& - q^{15} (-2q^4 + q^6 + 2q^9 - q^{12} - q^{13} + q^{15}) x^{13} - q^{15} (q^6 - q^8 - 2q^{11} + q^{14} + q^{15} - q^{17}) x^{14} \\
& - q^{15} (q^5 - q^8 - q^9 + 2q^{13} + 2q^{14} - 3q^{16} - q^{17} + q^{19} + q^{20}) x^{15} \\
& - q^{15} (-q^7 + q^{10} + q^{12} - 2q^{15} - 2q^{16} + 3q^{18} + q^{19} - q^{21} - q^{22}) x^{16} \\
& - q^{15} (-q^8 + q^9 + q^{10} - q^{12} - q^{14} - q^{15} + 3q^{17} + 2q^{18} - 3q^{20} - 3q^{21} + q^{23} + q^{24}) x^{17} \\
& - q^{15} (q^{10} - q^{11} + q^{14} - q^{15} + 2q^{16} + 2q^{17} - 4q^{19} - 3q^{20} + 3q^{22} + 3q^{23} - q^{25} - q^{26}) x^{18} \\
& - q^{15} (-q^{12} + q^{13} - q^{16} + q^{17} - 2q^{18} - q^{19} + 4q^{21} + 4q^{22} - 3q^{24} - 3q^{25} + q^{27} + q^{28}) x^{19} \\
& - q^{15} (-q^{15} + q^{16} - q^{17} - q^{18} - q^{19} + 2q^{20} + 2q^{21} + 2q^{22} - 3q^{23} - 5q^{24} - q^{25} + 3q^{26} + 4q^{27} - q^{29} - q^{30}) x^{20} \\
& - q^{15} (q^{17} - q^{18} + q^{19} - 2q^{22} - 2q^{23} - 2q^{24} + 4q^{25} + 4q^{26} + q^{27} - 3q^{28} - 4q^{29} + q^{31} + q^{32}) x^{21} \\
& - q^{15} (q^{20} - 2q^{23} + q^{24} + 2q^{25} + 3q^{26} - 2q^{27} - 4q^{28} - 2q^{29} + q^{30} + 4q^{31} + q^{32} - q^{33} - q^{34}) x^{22} \\
& - q^{15} (2q^{25} - 2q^{26} - 2q^{27} - 2q^{28} + 2q^{29} + 4q^{30} + 2q^{31} - 2q^{32} - 4q^{33} - q^{34} + q^{35} + q^{36}) x^{23} \\
& - q^{15} (q^{26} - 2q^{27} + q^{29} + 2q^{30} - 2q^{32} - 3q^{33} + q^{34} + 2q^{35} + q^{36} - q^{38}) x^{24} \\
& - q^{15} (q^{29} - q^{31} - 2q^{32} + q^{33} + 3q^{34} + 3q^{35} - q^{36} - 2q^{37} - q^{38} + q^{40}) x^{25} \\
& - q^{15} (-q^{33} + 2q^{34} - q^{36} - q^{37} + q^{39} + q^{40}) x^{26} - q^{15} (-2q^{36} + q^{38} + q^{39} - q^{41} - q^{42}) x^{27} \\
& + q^{56} x^{28} - q^{58} x^{29}
\end{aligned}$$

$$\begin{aligned}
t_4 = & q^{43} x^{16} - q^{45} x^{17} - 2q^{44} x^{18} + 2q^{46} x^{19} + q^{45} x^{20} + q^{43} (-2q^4 + q^6) x^{21} \\
& + q^{43} (q^6 - q^8) x^{22} + q^{43} (q^5 - q^8 - q^9 + q^{10}) x^{23} + q^{43} (-q^7 + q^{10} - q^{12}) x^{24} \\
& + q^{43} (-q^8 + q^9 + q^{10} - q^{12} + q^{14}) x^{25} + q^{43} (q^{10} - q^{11} + q^{13} + q^{14}) x^{26} \\
& + q^{43} (-q^{12} + q^{13} - q^{15} - q^{16}) x^{27} - q^{58} x^{28} + q^{60} x^{29}
\end{aligned}$$

$$\begin{aligned}
h_0 = & -q^{302} [-1 + (1 + q + q^2 + q^3 + q^4 + q^5 + q^6) x \\
& - q (1 + q + 2q^2 + 2q^3 + 3q^4 + 3q^5 + 3q^6 + 2q^7 + 2q^8 + q^9 + q^{10}) x^2 \\
& + q^3 (1 + q + 2q^2 + 3q^3 + 4q^4 + 4q^5 + 5q^6 + 4q^7 + 4q^8 + 3q^9 + 2q^{10} + q^{11} + q^{12}) x^3 \\
& - q^6 (1 + q + 2q^2 + 3q^3 + 4q^4 + 4q^5 + 5q^6 + 4q^7 + 4q^8 + 3q^9 + 2q^{10} + q^{11} + q^{12}) x^4 \\
& + q^{10} (1 + q + 2q^2 + 2q^3 + 3q^4 + 3q^5 + 3q^6 + 2q^7 + 2q^8 + q^9 + q^{10}) x^5 \\
& - q^{15} (1 + q + q^2 + q^3 + q^4 + q^5 + q^6) x^6 + q^{21} x^7]^2 \times \\
& [-1 + q^3 x^2 + q^7 x^2 + q^5 x^3 - q^{10} x^4 - q^{13} x^6 - q^{23} (-1 + x) x^7 - q^{158} x^{44} \\
& - q^{168} (-1 + x) x^{47} + q^{172} (1 - 2x) x^{49} + q^{175} (1 - 2x) x^{49} + q^{171} x^{50} - q^{181} x^{50} + q^{174} (-1 + x) x^{51} \\
& + q^{186} (-1 + x) x^{51} + q^{179} x^{53} + 2q^{188} x^{53} + q^{189} x^{53} + q^{191} x^{54} - q^{187} (-1 + x) x^{54} \\
& - q^{190} x^{55} - q^{192} x^{56} - q^{198} x^{56} + q^{203} x^{58} - q^{196} x^{55} (1 + x) + q^{183} (-1 + x) x^{50} (1 + x)^2 \\
& + q^{185} x^{53} (2 + x) + q^{167} x^{46} (-1 + x - 2x^2) + q^{154} x^{44} (-2 + x^2) \\
& + q^{15} x^5 (-1 + x^2) + q^{182} x^{51} (-1 + x^2) - q^{173} x^{48} (-1 + 2x + x^2) \\
& - q^{31} x^{11} (-1 + x + 2x^2) + q^{26} x^8 (1 + x + 3x^2) + q^{160} x^{45} (1 + 2x - x^3) \\
& + q^{176} x^{50} (-1 + x^3) - q^{17} x^5 (2 + x^3) - q^{12} x^4 (1 + x + x^3) \\
& + q^{164} x^{47} (1 - x^2 + x^3) - q^{177} x^{50} (1 + x - x^2 + x^3) - q^{27} x^{10} (-1 + x^2 + x^3) \\
& + q^{180} x^{50} (-1 + x^2 + x^3) - q^{169} x^{48} (-1 + 3x^2 + x^3) + q^{165} x^{45} (-1 + x + x^3 - x^4) \\
& + q^{21} x^5 (-1 + x^4) - q^{161} x^{45} (-1 - x + x^2 + x^4) + q^{22} x^6 (-1 + 3x^2 + x^4) \\
& - q^{156} x^{43} (1 - 2x^2 - 2x^3 + x^4) + q^{19} x^6 (-1 + x^3 + x^4) + q^{170} x^{47} (1 + 3x - 2x^2 + x^3 + x^4) \\
& + q^{24} x^7 (2 - x + x^2 + x^3 + x^4) + q^{30} x^8 (1 + 2x + x^2 + x^3 + x^4) + q^{43} x^{14} (3 - x + 2x^2 + x^3 + x^4) \\
& + q^{25} x^5 (-1 - x + 2x^3 + x^4) + q^{39} x^{13} (-2 - x + 2x^2 + 2x^4) + q^{145} x^{41} (2 - x - 3x^2 + x^3 + 2x^4) \\
& + q^{28} x^7 (1 + 2x - x^5) + q^8 (x^3 - x^5) + q^{11} (x^3 - x^5) + q^{14} (x^3 - x^5) + q^{29} x^7 (1 + x + x^4 - x^5) \\
& + q^{20} x^5 (-2 + x^2 + x^5) + q^9 (x^2 + x^5) + q^{166} x^{46} (1 + x - x^3 + x^5) + q^{38} x^{11} (-1 - 5x - 3x^2 - x^3 + x^5) \\
& - q^{35} x^9 (1 - x - x^2 + x^3 + x^5) - q^{149} x^{41} (1 - x + 2x^2 + x^3 - 2x^4 + x^5) + q^{140} x^{39} (-1 + 3x - 4x^3 - x^4 + x^5) \\
& + q^{151} x^{41} (1 - 2x - x^2 - x^3 + 2x^4 + x^5) + q^{41} x^{11} (-1 - 2x + 2x^3 + 2x^4 + x^5) \\
& - q^{159} x^{44} (1 + x + x^2 - 3x^3 + 3x^4 + x^5) + q^{54} x^{14} (1 + x + x^2 - 2x^3 - 2x^4 - 2x^5 - 5x^6) \\
& + q^{105} x^{30} (-4 + x + x^2 + x^3 - 3x^4 - 5x^5 - 3x^6) - q^{153} x^{42} (1 + x + 2x^2 - x^4 + x^6) \\
& - q^{34} x^8 (-1 - 2x^2 + x^4 + x^6) + q^{37} x^{10} (-3 - 2x^2 - 2x^3 - 4x^5 + x^6) \\
& - q^{132} x^{36} (4 + x + x^2 + 2x^3 + x^4 - 4x^5 + x^6) + q^{36} x^8 (1 - x^2 - 2x^3 - x^4 - 2x^5 + x^6) \\
& + q^{107} x^{31} (-4 - 3x - 6x^2 + 3x^3 - 7x^4 + x^5 + x^6) - q^{155} x^{42} (1 + x^2 - x^4 + x^5 + x^6) \\
& + q^{142} x^{36} (-1 + x^3 + x^4 + 3x^5 + x^6) - q^{51} x^{15} (-2 + x + 3x^2 - 2x^3 + 4x^5 + x^6) \\
& + q^{143} x^{39} (1 + x + 4x^2 - 2x^4 + x^5 + 2x^6) - q^{136} x^{36} (1 + x - x^2 + 2x^3 + x^4 - x^5 + 3x^6) \\
& - q^{125} x^{34} (-3 + x + x^2 - 2x^3 + x^4 + 2x^5 + 3x^6) + q^{135} x^{37} (-1 - 4x + 3x^4 - x^5 + 4x^6) \\
& + q^{75} x^{20} (1 + x + x^2 - 7x^5 + 2x^6 - 4x^7) + q^{48} x^{12} (1 - x + 2x^2 + x^3 - 3x^4 - 4x^5 + 3x^6 - 2x^7) \\
& + q^{103} x^{27} (3 - 3x^3 + x^4 + 7x^6 - 2x^7) + q^{121} x^{33} (5 + x + x^2 + x^3 - 2x^4 - x^5 - x^7)
\end{aligned}$$

$$\begin{aligned}
& + q^{120}x^{33}(1+x^2+2x^3-x^4+5x^5-x^7) + q^{49}x^{13}(-1+2x+3x^2+4x^3+2x^4+x^5-3x^6-x^7) \\
& + q^{141}x^{37}(-1+2x+x^2+x^3+4x^4+2x^5+x^6-x^7) + q^{116}x^{32}(-1+6x+x^3+2x^5+3x^6-x^7) \\
& + q^{146}x^{39}(1+2x+x^2+x^3-x^4-2x^5+x^7) - q^{152}x^{41}(1+x^2+2x^3-x^4-2x^5+x^7) \\
& + q^{111}x^{30}(-4-3x-2x^2-2x^3-x^4-5x^6+x^7) - q^{56}x^{16}(1+3x^2-x^4+4x^5-3x^6+x^7) \\
& + q^{46}x^{12}(-1+x^2+5x^3+6x^5-x^6+x^7) - q^{16}(x^4+x^6+x^7) + q^{144}x^{38}(1+x^2-2x^4-5x^5+x^6+x^7) \\
& - q^{157}x^{41}(1+x^2+x^3+x^4-5x^5+x^6+x^7) - q^{32}x^7(-1+x^2+x^3+x^5+x^6+x^7) \\
& - q^{128}x^{35}(3+x+x^2+x^3+2x^4+2x^5+x^6+x^7) - q^{33}x^8(-1-2x+3x^3+2x^4+2x^5+x^6+x^7) \\
& + q^{148}x^{39}(1+x^3-3x^5+2x^6+x^7) - q^{50}x^{14}(-1+2x^2-2x^4+3x^6+x^7) \\
& + q^{112}x^{31}(-3+x^2+2x^4+3x^5+4x^6+x^7) - q^{134}x^{35}(1+3x+4x^4-5x^5+2x^7) \\
& + q^{109}x^{30}(-3-5x-x^2-5x^3+x^4+3x^5-5x^6+2x^7) + q^{42}x^{11}(-1-x-2x^3+x^4+x^5+2x^6+2x^7) \\
& + q^{60}x^{16}(2-3x^2+3x^3-x^4-2x^5+5x^6+2x^7) + q^{110}x^{31}(-1+x-2x^2-4x^4-2x^5+3x^7) \\
& + q^{40}x^{10}(-1-x+x^2-x^3-x^4+x^5-x^6+3x^7) - q^{124}x^{34}(1-2x+x^2+4x^3+2x^4-2x^5+x^6+3x^7) \\
& - q^{74}x^{21}(-4+3x+x^2+x^3+3x^4-3x^5-x^6+4x^7) - q^{130}x^{34}(-1-x+x^2+4x^3+5x^4+3x^5+6x^7) \\
& + q^{94}x^{25}(-3-3x-4x^2-4x^3+2x^5-4x^6+6x^7) + q^{100}x^{27}(3-x^3+2x^4+x^5+x^6-3x^8) \\
& + q^{47}x^{12}(-1+x+2x^2+3x^3+x^4+2x^5+x^6-x^7-3x^8) \\
& + q^{123}x^{33}(1+3x-4x^2+3x^3+x^4+x^5+x^7-2x^8) \\
& + q^{70}x^{19}(1-3x+x^2+x^3-2x^4+3x^5-2x^6-5x^7-x^8) \\
& + q^{127}x^{33}(1+2x+x^2-2x^3-3x^4-6x^5+2x^6-2x^7-x^8) \\
& + q^{44}x^{11}(-1-x-2x^2+x^3+x^5+x^6+x^7-x^8) + q^{150}x^{39}(1+x^3-4x^4-2x^5+3x^6+x^7-x^8) \\
& - q^{66}x^{18}(1-2x-5x^2-3x^4+x^8) + q^{52}x^{14}(1+4x-x^3-4x^4-5x^5-2x^6+x^8) \\
& + q^{147}x^{38}(1+x+x^3+x^4-3x^5+2x^6+x^8) + q^{137}x^{36}(-2-x+3x^3+3x^4+5x^5-2x^7+x^8) \\
& + q^{138}x^{36}(-1-x-x^2+x^4+2x^5-x^6-x^7+x^8) + q^{139}x^{37}(-1+x+x^2+x^4+3x^5-2x^6+x^7+x^8) \\
& - q^{133}x^{34}(-1+x^2-3x^4+x^5-3x^6+2x^7+x^8) + q^{115}x^{31}(-1+3x-5x^2-x^3-3x^5-x^6+2x^7+x^8) \\
& + q^{55}x^{15}(1-x-x^2+x^3+2x^4-3x^5-x^6+2x^7+x^8) + q^{61}x^{17}(-2-x+2x^3+x^4+2x^5+3x^7+x^8) \\
& + q^{114}x^{31}(-3-2x+x^2+4x^3+6x^4+x^5+x^6+4x^7+x^8) \\
& + q^{117}x^{31}(-3-x-x^2+4x^3+x^5-x^6+5x^7+x^8) \\
& + q^{65}x^{17}(1-x+x^3+2x^4-x^5+7x^6+2x^8) - q^{119}x^{32}(1-2x-3x^2-5x^3+x^4+x^6-3x^7+2x^8) \\
& + q^{102}x^{28}(3+3x^2+4x^3-x^4+3x^5-2x^7+2x^8) - q^{126}x^{33}(-2-2x+2x^3+x^4+x^5+x^7+2x^8) \\
& + q^{63}x^{17}(-1-3x+x^2+x^3-3x^5+5x^6+x^7+2x^8) \\
& + q^{118}x^{31}(-1+4x+4x^2+x^3+3x^4+4x^5+3x^7+2x^8) + q^{59}x^{15}(1-x-4x^2+x^3-x^4+x^6+3x^7+2x^8) \\
& + q^{113}x^{30}(-5-x-x^3-5x^4+2x^5-4x^6-x^7+3x^8) + q^{86}x^{23}(3-x-x^2+3x^3-2x^4-9x^5+3x^7+4x^8) \\
& + q^{108}x^{27}(1-3x^3+4x^4-4x^5+2x^6+3x^7-3x^9) \\
& + q^{104}x^{27}(1+4x+2x^3-2x^4-3x^5+x^6+3x^7-5x^8-2x^9) \\
& + q^{53}x^{13}(1+x+x^2+2x^3-5x^4-3x^7-2x^8-2x^9) \\
& + q^{97}x^{26}(-4+3x-2x^2+4x^4+8x^5+4x^6+5x^7-3x^8-x^9)
\end{aligned}$$

$$\begin{aligned}
& + q^{129} x^{33} (1 + x^4 - 5x^5 + x^6 + 4x^7 - 2x^8 - x^9) \\
& + q^{45} x^{10} (-1 + x^3 + 2x^4 + 2x^5 + 3x^6 + 2x^7 + 2x^8 - x^9) \\
& + q^{62} x^{16} (1 - x + 2x^3 + x^4 + 5x^6 + 5x^7 + 3x^8 - x^9) \\
& + q^{90} x^{24} (-3 - 4x + 2x^2 + 2x^3 - 4x^4 - 5x^6 + x^9) \\
& - q^{69} x^{18} (2 + x - x^2 + 2x^3 + 4x^4 + 3x^6 + 5x^7 + x^9) \\
& + q^{67} x^{17} (-1 - x - 3x^2 + 5x^3 - x^4 - 3x^6 - 3x^8 + x^9) \\
& + q^{57} x^{14} (-1 - x^2 - 4x^3 - 5x^4 - 2x^5 - 5x^6 + x^7 - x^8 + x^9) \\
& + q^{131} x^{34} (1 - 2x - x^3 - 2x^4 + 2x^6 - 2x^7 + x^8 + x^9) \\
& - q^{71} x^{19} (1 - 3x^2 + 2x^3 + 2x^4 + 4x^5 + x^7 + x^8 + x^9) \\
& + q^{106} x^{28} (5 - 2x^2 + 2x^3 - 2x^4 - 5x^5 + 4x^6 + x^7 + x^8 + x^9) \\
& + q^{58} x^{15} (1 - x - 3x^2 + 2x^4 + x^5 - x^6 - x^7 + 3x^8 + x^9) \\
& + q^{79} x^{21} (1 + x - x^2 - 4x^3 + 6x^4 - x^5 + x^6 - 3x^7 + 2x^9) \\
& + q^{64} x^{16} (1 - x^2 + 4x^3 + 6x^4 + x^5 + 4x^6 - x^7 + 2x^9) \\
& - q^{122} x^{31} (1 + x - 3x^2 - 2x^3 - 4x^4 - 6x^5 - 5x^8 + 2x^9) \\
& - q^{91} x^{24} (2 + 2x + x^3 - 4x^4 + x^6 + 3x^7 - 5x^8 + 2x^9) \\
& + q^{77} x^{19} (-1 + 2x^3 - 5x^4 - x^6 + 3x^7 + 3x^8 + 2x^9) \\
& - q^{72} x^{19} (1 - 4x - x^2 + x^3 + 6x^4 + 3x^5 + x^6 + x^7 + 4x^8 + 2x^9) \\
& + q^{95} x^{24} (-1 - x + x^2 + 5x^3 - 3x^4 - 6x^7 - 3x^8 + 3x^9) \\
& + q^{80} x^{19} (-1 + x^2 - 4x^4 + x^5 - 2x^6 + 2x^7 + 4x^8 + 3x^9) \\
& - q^{76} x^{19} (1 + x - x^2 - x^3 + 3x^4 - x^5 + x^6 + 4x^7 + 4x^9) \\
& + q^{96} x^{24} (-1 + x^2 + x^3 + 3x^4 - 4x^7 - 2x^8 - 3x^{10}) \\
& - q^{99} x^{25} (1 - x^2 - 2x^3 - 8x^5 + x^7 + x^{10}) \\
& - q^{88} x^{22} (-2 + x + 3x^2 + 6x^3 - x^4 + 4x^5 + x^9 + x^{10}) \\
& + q^{85} x^{21} (1 + 3x - x^2 + x^4 + 2x^5 + 5x^7 + x^9 + x^{10}) \\
& + q^{87} x^{22} (1 - 2x^2 + 5x^3 + 4x^4 + 4x^5 - 2x^6 - 3x^8 + 3x^9 + x^{10}) \\
& + q^{83} x^{21} (1 + 4x + x^2 - x^3 + 2x^4 + 3x^5 - 8x^6 + 5x^7 + 4x^9 + x^{10}) \\
& + q^{82} x^{21} (1 - 2x^2 - 4x^3 + 2x^4 + 4x^6 + 3x^7 + 2x^{10}) \\
& - q^{92} x^{23} (-1 + 2x + x^2 + 2x^4 + 8x^5 + 5x^7 - x^9 + 2x^{10}) \\
& - q^{68} x^{17} (-1 - 2x^3 - 4x^4 + x^5 - 4x^6 - 2x^7 + x^9 + 2x^{10}) \\
& - q^{73} x^{17} (-1 + x^2 + x^3 + x^4 + 6x^5 + 3x^7 - 3x^8 + 6x^9 + 3x^{10}) \\
& + q^{81} x^{20} (-1 + x + x^2 + 4x^3 + 5x^5 + x^6 + 6x^7 + 4x^{10}) \\
& + q^{89} x^{22} (1 + 2x + x^2 + x^3 - x^4 - x^5 - 3x^8 + 4x^9 + x^{10} - x^{11}) \\
& + q^{78} x^{19} (-1 - 2x + 2x^3 - x^4 + 5x^5 + 5x^6 + x^7 - x^9 + x^{11}) \\
& + q^{84} x^{20} (-1 + x^2 - 3x^4 - x^5 - x^6 - 3x^7 + x^8 - 2x^{10} + x^{11}) \\
& + q^{98} x^{24} (-1 - 2x + x^2 + 3x^3 + 4x^4 - 4x^6 + 3x^7 - 3x^8 + 2x^9 - x^{10} + x^{11})
\end{aligned}$$

$$\begin{aligned}
& -q^{101}x^{25}(1-x-x^2-3x^3-4x^5+4x^6+2x^7+3x^8+2x^{10}+x^{11}) \\
& +q^{93}x^{22}(1-5x^3+2x^4+4x^5+x^6+9x^8-x^9+x^{10}-2x^{11}-x^{12}) \\
& +q^{162}(x^{44}+2x^{47})+q^{163}(x^{46}-x^{48})+q^{178}(x^{48}-2x^{51})+q^{193}(x^{53}-x^{55})]
\end{aligned}$$

$$\begin{aligned}
h_1 = & -q^{298}[-1+(1+q+q^2+q^3+q^5+q^6)x-q(1+q+2q^2+q^3+2q^4+2q^5+2q^6+q^7+q^8+q^{10})x^2 \\
& +q^3(1+q+q^2+2q^3+2q^4+2q^5+2q^6+q^7+q^8+q^9)x^3 \\
& +q^6(-1-q^2-q^3-q^4-q^6+q^7+q^9+q^{10}+q^{11}+q^{13})x^4 \\
& -q^{13}(1+q+q^2+2q^3+2q^4+2q^5+2q^6+q^7+q^8+q^9)x^5 \\
& +q^{14}(1+q^2+q^3+2q^4+2q^5+2q^6+q^7+2q^8+q^9+q^{10})x^6 \\
& -q^{19}(1+q+q^3+q^4+q^5+q^6)x^7+q^{25}x^8]^2 \times \\
& [1-qx^2-2q^2x^3+q^3x^5+q^{175}x^{54}-q^{170}x^{56}+2q^{173}x^{56}-q^{177}x^{57}+q^{180}x^{59}+q^{168}x^{54}(-3+x-4x^2) \\
& -q^{169}x^{55}(3+x^2)+q^{172}x^{55}(2+3x^2)+q^{162}x^{51}(1-2x-5x^3)+q^{166}x^{52}(-1+x+3x^3) \\
& +q^{158}x^{50}(-1+3x-x^2+7x^3)-q^{171}x^{53}(2+x^4)+q^6x^4(4+x^4)+q^5x^3(2+x^2+x^4) \\
& +q^{167}x^{52}(3+2x^2+x^4)-q^{163}x^{51}(4+3x^2+x^4)-q^{164}x^{52}(1-4x+2x^2-5x^3+2x^4) \\
& +q^{160}x^{51}(3-5x+5x^2-5x^3+5x^4)+q^{156}x^{49}(1-5x+6x^2-10x^3+5x^4-7x^5) \\
& +q^{161}x^{50}(2+x^2-7x^3+3x^4-3x^5)+q^{154}x^{49}(2-4x+x^2-9x^3+2x^4-x^5)+q^4x(-2-x^4+x^5) \\
& +q^{159}x^{49}(-1+4x-2x^2+4x^3+2x^5)+q^{165}x^{51}(-1+5x^3+2x^5)+q^{157}x^{49}(-3-3x^2+8x^3-6x^4+4x^5) \\
& +q^{152}x^{48}(-1+7x-8x^2+14x^3-8x^4+9x^5)+q^8x^2(3-x+x^2+2x^4-2x^5+x^6) \\
& +q^{150}x^{47}(1-2x+8x^2-4x^3+11x^4-6x^5+2x^6)-q^{12}x^3(4-2x+x^2+5x^4-4x^5+4x^6) \\
& -q^{10}x^4(-1+6x-2x^2+x^3+2x^5+x^7)+q^{15}x^4(-1+2x-4x^2+x^3-5x^4+3x^5-5x^6+x^7) \\
& +q^{155}x^{47}(1+2x-3x^2+5x^3-6x^4+x^5-3x^6+3x^7)-q^7(x^2+2x^6+x^8) \\
& +q^{148}x^{45}(-1+2x^2-8x^3+10x^4-18x^5+11x^6-11x^7+x^8) \\
& +q^{19}x^5(1-3x+6x^2-5x^3+7x^4-7x^5+8x^6-3x^7+x^8) \\
& +q^{16}x^4(6-3x+3x^2-x^3+9x^4-6x^5+7x^6-x^7+2x^8) \\
& +q^{153}x^{45}(1+4x^3-x^4+4x^5-9x^6+9x^7-5x^8+x^9) \\
& -q^{149}x^{44}(2+4x^3-4x^4+7x^5-10x^6+13x^7-5x^8+2x^9) \\
& +q^{11}(x^3+2x^5+4x^7-2x^8+2x^9) \\
& +q^{14}x^3(-1-3x^2+8x^3-5x^4+x^5-x^6+4x^7-x^8+2x^9) \\
& -q^{146}x^{43}(1+x^2+x^3-3x^4+9x^5-8x^6+12x^7-9x^8+4x^9) \\
& +q^{145}x^{43}(3-x+3x^3-8x^4+10x^5-13x^6+17x^7-9x^8+4x^9) \\
& +q^{17}x^4(-3+x-6x^2+5x^3-9x^4+4x^5-6x^6+3x^7-6x^8+3x^9-2x^{10}) \\
& +q^{22}x^5(-3+x-8x^2+14x^3-14x^4+4x^5-7x^6+10x^7-9x^8+4x^9-2x^{10}) \\
& -q^{20}x^5(6-4x+5x^2-x^3+14x^4-11x^5+11x^6-3x^7+3x^8+x^{10}) \\
& +q^{13}x^3(2+4x^2-4x^3+4x^4-2x^5+3x^6-2x^7+4x^8+x^{10})
\end{aligned}$$

$$\begin{aligned}
& + q^{18}x^4(2 + 5x^2 - 13x^3 + 9x^4 - 2x^5 + 4x^6 - 6x^7 + 4x^8 - 3x^9 + x^{10}) \\
& - q^9(x^2 + 3x^4 - 3x^5 + 2x^6 + 2x^8 + 2x^{10}) \\
& + q^{26}x^6(4 - 3x + 10x^2 - 15x^3 + 21x^4 - 9x^5 + 14x^6 - 12x^7 + 14x^8 - 8x^9 + 3x^{10}) \\
& - q^{23}x^6(1 - 5x + 11x^2 - 9x^3 + 9x^4 - 10x^5 + 11x^6 - 9x^7 + 2x^8 - 2x^9 + x^{11}) \\
& - q^{21}x^5(-5 + 2x - 7x^2 + 6x^3 - 13x^4 + 7x^5 - 12x^6 + 4x^7 - 10x^8 + 5x^9 - 3x^{10} + x^{11}) \\
& - q^{151}x^{42}(1 + x^4 + 3x^5 - 2x^6 + 8x^7 - 8x^8 + 6x^9 - 5x^{10} + 4x^{11}) \\
& + q^{142}x^{40}(1 + 2x^2 - x^3 + x^5 - 4x^6 + 11x^7 - 11x^8 + 17x^9 - 13x^{10} + 5x^{11}) \\
& + q^{147}x^{41}(2 + x^4 + 4x^5 - x^6 + 10x^7 - 10x^8 + 10x^9 - 7x^{10} + 5x^{11}) \\
& + q^{131}x^{37}(6 - 5x + 4x^2 - 3x^3 + x^4 + 2x^5 - 9x^6 + 7x^7 - 23x^8 + 28x^9 - 26x^{10} + 15x^{11} - 9x^{12}) \\
& + q^{133}x^{37}(3 - x - 6x^3 + 9x^4 - 2x^5 + x^6 + 15x^7 - 22x^8 + 30x^9 - 27x^{10} + 20x^{11} - 7x^{12}) \\
& + q^{118}x^{34}(5 - 9x + 11x^2 - 17x^3 + 9x^4 - 5x^6 + 22x^7 - 35x^8 + 44x^9 - 39x^{10} + 26x^{11} - 7x^{12}) \\
& + q^{126}x^{36}(3 - 7x + 6x^2 - 10x^3 + 4x^4 + x^5 - 6x^6 + 19x^7 - 31x^8 + 34x^9 - 31x^{10} + 16x^{11} - 6x^{12}) \\
& + q^{141}x^{39}(1 - 4x^3 + 2x^4 - 2x^6 + 11x^7 - 13x^8 + 20x^9 - 21x^{10} + 12x^{11} - 5x^{12}) \\
& + q^{139}x^{39}(4 + 2x^2 + 2x^4 + 3x^5 - 5x^6 + 8x^7 - 15x^8 + 17x^9 - 15x^{10} + 9x^{11} - 4x^{12}) \\
& + q^{29}x^6(-2 + 6x - 5x^2 + 7x^3 - 10x^4 + 25x^5 - 17x^6 + 23x^7 - 11x^8 + 19x^9 - 9x^{10} + 6x^{11} - 3x^{12}) \\
& + q^{134}x^{38}(1 - 2x + 5x^2 - 3x^3 + x^4 + x^5 - 6x^6 + 14x^7 - 22x^8 + 23x^9 - 20x^{10} + 9x^{11} - 3x^{12}) \\
& - q^{24}x^6(-6 + 6x - 8x^2 + 4x^3 - 18x^4 + 13x^5 - 17x^6 + 5x^7 - 5x^8 + 2x^9 - 2x^{10} + x^{12}) \\
& + q^{143}x^{40}(-3 - x^2 - x^4 - 5x^5 + 2x^6 - 10x^7 + 12x^8 - 13x^9 + 10x^{10} - 7x^{11} + x^{12}) \\
& + q^{138}x^{39}(-1 + x - 3x^2 + 2x^3 - x^5 + 4x^6 - 14x^7 + 15x^8 - 19x^9 + 17x^{10} - 7x^{11} + x^{12}) \\
& + q^{30}x^7(-5 + 5x - 12x^2 + 18x^3 - 25x^4 + 15x^5 - 19x^6 + 15x^7 - 22x^8 + 11x^9 - 6x^{10} - x^{11} + x^{12}) \\
& + q^{25}x^5(1 - 6x + 3x^2 - 7x^3 + 8x^4 - 19x^5 + 12x^6 - 17x^7 + 7x^8 - 15x^9 + 7x^{10} - 5x^{11} + 2x^{12}) \\
& + q^{28}x^7(-6 + 7x - 11x^2 + 8x^3 - 21x^4 + 17x^5 - 23x^6 + 10x^7 - 8x^8 + 2x^9 - 3x^{10} + x^{11} + 2x^{12}) \\
& - q^{144}x^{40}(-1 + x^3 - 2x^4 + 2x^5 + 3x^6 - 9x^7 + 14x^8 - 21x^9 + 16x^{10} - 12x^{11} + 3x^{12}) \\
& + q^{140}x^{39}(-2 + x + 2x^3 - 3x^4 + 3x^5 + 3x^6 - 11x^7 + 20x^8 - 25x^9 + 22x^{10} - 14x^{11} + 5x^{12}) \\
& + q^{130}x^{37}(-2 + 3x - 6x^2 + 6x^3 - 2x^4 + 2x^5 + 6x^6 - 17x^7 + 25x^8 - 28x^9 + 25x^{10} - 11x^{11} + 5x^{12}) \\
& + q^{137}x^{38}(-2 + 6x^3 - 5x^4 + x^5 + x^6 - 14x^7 + 17x^8 - 24x^9 + 24x^{10} - 16x^{11} + 6x^{12}) \\
& + q^{135}x^{38}(-6 + 2x - 3x^2 + x^3 - x^4 - x^5 + 7x^6 - 7x^7 + 20x^8 - 22x^9 + 21x^{10} - 12x^{11} + 6x^{12}) \\
& + q^{122}x^{35}(-4 + 8x - 8x^2 + 12x^3 - 6x^4 - x^5 + 6x^6 - 20x^7 + 34x^8 - 39x^9 + 35x^{10} - 21x^{11} + 7x^{12}) \\
& + q^{114}x^{33}(-6 + 11x - 14x^2 + 18x^3 - 12x^4 + 2x^5 + 2x^6 - 25x^7 + 38x^8 - 48x^9 + 42x^{10} - 31x^{11} + 8x^{12}) \\
& - q^{110}x^{32}(-7 + 14x - 19x^2 + 16x^3 - 17x^4 + x^5 + 3x^6 - 27x^7 + 39x^8 - 53x^9 + 49x^{10} - 34x^{11} + 11x^{12}) \\
& + q^{27}x^7(1 - 9x + 14x^2 - 13x^3 + 10x^4 - 15x^5 + 16x^6 - 14x^7 + 4x^8 - 6x^9 + x^{11} + x^{13}) \\
& - q^{106}x^{31}(8 - 14x + 23x^2 - 15x^3 + 22x^4 - 4x^5 - 4x^6 + 28x^7 - 40x^8 + 55x^9 - 56x^{10} + 35x^{11} - 12x^{12} + x^{13}) \\
& + q^{33}x^7(3 - 7x + 6x^2 - 8x^3 + 12x^4 - 30x^5 + 24x^6 - 30x^7 + 14x^8 - 22x^9 + 13x^{10} - 9x^{11} + 4x^{12} + x^{13}) \\
& - q^{31}x^8(1 - 13x + 16x^2 - 20x^3 + 11x^4 - 20x^5 + 20x^6 - 21x^7 + 9x^8 - 9x^9 + x^{10} + x^{11} - 3x^{12} + 2x^{13}) \\
& - q^{129}x^{36}(4 - 2x + x^2 - 6x^3 + 13x^4 - 5x^5 + 3x^6 + 13x^7 - 25x^8 + 37x^9 - 31x^{10} + 25x^{11} - 10x^{12} + 3x^{13})
\end{aligned}$$

$$\begin{aligned}
& + q^{125}x^{35} (6 - 5x + 2x^2 - 6x^3 + 16x^4 - 9x^5 + 4x^6 + 13x^7 - 27x^8 + 42x^9 - 38x^{10} + 31x^{11} - 12x^{12} + 5x^{13}) \\
& - q^{136}x^{37} (1 - 3x + 2x^2 + 3x^4 - 5x^5 + 4x^6 + 4x^7 - 11x^8 + 23x^9 - 32x^{10} + 28x^{11} - 19x^{12} + 7x^{13}) \\
& - q^{121}x^{34} (7 - 9x + 3x^2 - 6x^3 + 22x^4 - 13x^5 + 7x^6 + 12x^7 - 31x^8 + 45x^9 - 44x^{10} + 37x^{11} - 16x^{12} + 7x^{13}) \\
& + q^{132}x^{36} (2 - 5x + 3x^2 + 5x^4 - 6x^5 + 7x^6 + 5x^7 - 12x^8 + 25x^9 - 37x^{10} + 34x^{11} - 23x^{12} + 9x^{13}) \\
& + q^{117}x^{33} (8 - 12x + 6x^2 - 6x^3 + 23x^4 - 17x^5 + 7x^6 + 10x^7 - 32x^8 + 48x^9 - 50x^{10} + 41x^{11} - 21x^{12} + 9x^{13}) \\
& - q^{128}x^{35} (3 - 6x + 6x^2 + 7x^4 - 9x^5 + 11x^6 + 2x^7 - 14x^8 + 30x^9 - 42x^{10} + 37x^{11} - 29x^{12} + 11x^{13}) \\
& + q^{109}x^{31} (10 - 17x + 11x^2 - 9x^3 + 27x^4 - 24x^5 + 14x^6 + 9x^7 - 34x^8 + 49x^9 - 60x^{10} + 46x^{11} - 29x^{12} \\
& + 11x^{13}) \\
& - q^{113}x^{32} (9 - 14x + 7x^2 - 9x^3 + 24x^4 - 22x^5 + 11x^6 + 10x^7 - 33x^8 + 48x^9 - 55x^{10} + 44x^{11} - 26x^{12} \\
& + 11x^{13}) \\
& + q^{127}x^{35} (1 - 6x + 7x^2 - 6x^3 + 6x^4 - 2x^5 - 2x^6 + 11x^7 - 7x^8 + 26x^9 - 32x^{10} + 32x^{11} - 19x^{12} + 11x^{13}) \\
& - q^{123}x^{34} (1 - 6x + 9x^2 - 7x^3 + 10x^4 - 3x^5 + x^6 + 10x^7 - 11x^8 + 28x^9 - 36x^{10} + 37x^{11} - 23x^{12} + 12x^{13}) \\
& - q^{105}x^{30} (11 - 16x + 15x^2 - 10x^3 + 27x^4 - 29x^5 + 16x^6 + 10x^7 - 33x^8 + 54x^9 - 63x^{10} + 49x^{11} - 32x^{12} \\
& + 13x^{13}) \\
& + q^{119}x^{33} (1 - 6x + 14x^2 - 9x^3 + 13x^4 - 6x^5 - x^6 + 6x^7 - 14x^8 + 32x^9 - 42x^{10} + 42x^{11} - 26x^{12} \\
& + 15x^{13}) \\
& + q^{108}x^{30} (5 - 15x + 16x^2 - 10x^3 + 13x^4 - 26x^5 + 20x^6 - 10x^7 - 20x^8 + 40x^9 - 70x^{10} + 66x^{11} \\
& - 53x^{12} + 20x^{13} - 7x^{14}) \\
& + q^{36}x^8 (1 - 6x + 9x^2 - 15x^3 + 18x^4 - 28x^5 + 25x^6 - 32x^7 + 22x^8 - 16x^9 + 7x^{10} - 5x^{11} - 2x^{12} \\
& + 4x^{13} - 5x^{14}) \\
& + q^{116}x^{32} (5 - 11x + 17x^2 - 4x^3 + 11x^4 - 19x^5 + 19x^6 - 6x^7 - 19x^8 + 37x^9 - 61x^{10} + 56x^{11} \\
& - 45x^{12} + 17x^{13} - 5x^{14}) \\
& + q^{103}x^{29} (1 - 8x + 13x^2 - 25x^3 + 17x^4 - 18x^5 + 3x^6 + 6x^7 - 21x^8 + 32x^9 - 61x^{10} + 69x^{11} \\
& - 41x^{12} + 23x^{13} - 5x^{14}) \\
& + q^{111}x^{31} (1 - 9x + 14x^2 - 15x^3 + 18x^4 - 13x^5 + x^6 + 7x^7 - 21x^8 + 33x^9 - 53x^{10} + 58x^{11} \\
& - 34x^{12} + 19x^{13} - 3x^{14}) \\
& + q^{35}x^9 (1 - 17x + 19x^2 - 22x^3 + 14x^4 - 26x^5 + 24x^6 - 31x^7 + 13x^8 - 12x^9 + 2x^{10} + x^{11} - 5x^{12} \\
& + 3x^{13} - 2x^{14}) \\
& + q^{34}x^8 (5 - 7x + 15x^2 - 19x^3 + 29x^4 - 22x^5 + 24x^6 - 23x^7 + 27x^8 - 14x^9 + 9x^{10} + x^{11} - x^{14}) \\
& - q^{124}x^{34} (-4 + 6x - 10x^2 + x^3 - 9x^4 + 11x^5 - 12x^6 + x^7 + 14x^8 - 32x^9 + 51x^{10} - 42x^{11} + 33x^{12} \\
& - 14x^{13} + x^{14}) \\
& + q^{115}x^{32} (-1 + 6x - 14x^2 + 12x^3 - 15x^4 + 10x^5 + x^6 - 7x^7 + 16x^8 - 33x^9 + 48x^{10} - 51x^{11} + 29x^{12} \\
& - 17x^{13} + 2x^{14}) \\
& + q^{32}x^7 (-1 + 6x - 8x^2 + 14x^3 - 12x^4 + 26x^5 - 22x^6 + 27x^7 - 16x^8 + 11x^9 - 5x^{10} + 4x^{11} - 3x^{13} + 2x^{14}) \\
& + q^{37}x^8 (-4 + 8x - 5x^2 + 9x^3 - 15x^4 + 37x^5 - 29x^6 + 33x^7 - 19x^8 + 26x^9 - 16x^{10} + 12x^{11} - 3x^{12}
\end{aligned}$$



$$\begin{aligned}
& -x^{13} + 2x^{14}) \\
& + q^{38}x^9 (-5 + 9x - 16x^2 + 19x^3 - 33x^4 + 26x^5 - 31x^6 + 26x^7 - 32x^8 + 21x^9 - 9x^{10} - x^{11} + 2x^{12} \\
& - 2x^{13} + 3x^{14}) \\
& + q^{107}x^{30} (-1 + 8x - 15x^2 + 19x^3 - 17x^4 + 15x^5 - x^6 - 5x^7 + 23x^8 - 33x^9 + 58x^{10} - 64x^{11} + 39x^{12} \\
& - 21x^{13} + 4x^{14}) \\
& + q^{120}x^{33} (-5 + 8x - 12x^2 + 2x^3 - 10x^4 + 15x^5 - 17x^6 + 4x^7 + 16x^8 - 34x^9 + 56x^{10} - 50x^{11} + 37x^{12} \\
& - 16x^{13} + 4x^{14}) \\
& + q^{39}x^{10} (-2 + 20x - 22x^2 + 20x^3 - 17x^4 + 31x^5 - 29x^6 + 36x^7 - 18x^8 + 18x^9 - x^{10} - 2x^{11} + 7x^{12} \\
& - 7x^{13} + 4x^{14}) \\
& + q^{99}x^{28} (-1 + 8x - 12x^2 + 28x^3 - 18x^4 + 20x^5 - 7x^6 - 7x^7 + 20x^8 - 34x^9 + 59x^{10} - 69x^{11} + 43x^{12} \\
& - 25x^{13} + 6x^{14}) \\
& + q^{112}x^{31} (-5 + 13x - 18x^2 + 6x^3 - 12x^4 + 24x^5 - 20x^6 + 10x^7 + 20x^8 - 39x^9 + 68x^{10} - 62x^{11} + 49x^{12} \\
& - 19x^{13} + 6x^{14}) \\
& + q^{104}x^{29} (-5 + 18x - 16x^2 + 14x^3 - 14x^4 + 26x^5 - 23x^6 + 14x^7 + 20x^8 - 42x^9 + 73x^{10} - 68x^{11} + 56x^{12} \\
& - 23x^{13} + 7x^{14}) \\
& + q^{95}x^{26} (-2 + 2x - 9x^2 + 17x^3 - 32x^4 + 20x^5 - 19x^6 + 12x^7 + 6x^8 - 17x^9 + 37x^{10} - 60x^{11} + 69x^{12} \\
& - 45x^{13} + 26x^{14} - 6x^{15}) \\
& + q^{98}x^{27} (-4 + x - 7x^2 + 19x^3 - 28x^4 + 16x^5 - 30x^6 + 12x^7 + 5x^8 - 26x^9 + 43x^{10} - 61x^{11} + 64x^{12} \\
& - 34x^{13} + 14x^{14} - x^{15}) \\
& + q^{102}x^{28} (2 + 9x^2 - 16x^3 + 25x^4 - 17x^5 + 26x^6 - 9x^7 - 4x^8 + 28x^9 - 42x^{10} + 60x^{11} - 60x^{12} \\
& + 36x^{13} - 13x^{14} + x^{15}) \\
& - q^{40}x^9 (1 - 7x + 9x^2 - 18x^3 + 22x^4 - 29x^5 + 30x^6 - 36x^7 + 27x^8 - 19x^9 + 9x^{10} - 9x^{11} - 4x^{12} \\
& + 8x^{13} - 8x^{14} + x^{15}) \\
& + q^{43}x^{11} (3 - 22x + 24x^2 - 18x^3 + 20x^4 - 34x^5 + 34x^6 - 39x^7 + 23x^8 - 17x^9 + x^{10} + 2x^{11} - 9x^{12} \\
& + 10x^{13} - 6x^{14} + x^{15}) \\
& - q^{47}x^{12} (3 - 22x + 27x^2 - 16x^3 + 21x^4 - 38x^5 + 37x^6 - 40x^7 + 29x^8 - 15x^9 + x^{10} + 3x^{11} - 13x^{12} \\
& + 15x^{13} - 9x^{14} + 2x^{15}) \\
& + q^{42}x^{10} (5 - 10x + 17x^2 - 21x^3 + 34x^4 - 32x^5 + 35x^6 - 28x^7 + 40x^8 - 23x^9 + 12x^{10} - 4x^{12} + 2x^{13} \\
& - 5x^{14} + 2x^{15}) \\
& + q^{44}x^{10} (1 - 7x + 10x^2 - 19x^3 + 23x^4 - 32x^5 + 33x^6 - 40x^7 + 31x^8 - 21x^9 + 14x^{10} - 7x^{11} - 7x^{12} \\
& + 11x^{13} - 13x^{14} + 4x^{15}) \\
& - q^{46}x^{11} (5 - 11x + 18x^2 - 21x^3 + 37x^4 - 33x^5 + 36x^6 - 32x^7 + 44x^8 - 24x^9 + 16x^{10} + 3x^{11} - 7x^{12} \\
& + 6x^{13} - 8x^{14} + 4x^{15}) \\
& + q^{51}x^{13} (3 - 22x + 29x^2 - 16x^3 + 22x^4 - 38x^5 + 38x^6 - 41x^7 + 31x^8 - 15x^9 - 2x^{10} + 4x^{11} - 17x^{12} \\
& + 20x^{13} - 14x^{14} + 5x^{15})
\end{aligned}$$

$$\begin{aligned}
& -q^{97}x^{26}(2+12x^2-16x^3+25x^4-11x^5+29x^6-33x^7+20x^8+12x^9-31x^{10}+59x^{11}-69x^{12} \\
& +57x^{13}-36x^{14}+13x^{15}) \\
& +q^{101}x^{27}(1+12x^2-16x^3+20x^4-11x^5+26x^6-31x^7+17x^8+14x^9-32x^{10}+55x^{11}-66x^{12} \\
& +55x^{13}-34x^{14}+13x^{15}) \\
& +q^{67}x^{17}(1-17x+19x^2-19x^3+13x^4-33x^5+34x^6-43x^7+27x^8-21x^9-3x^{10}+14x^{11}-32x^{12} \\
& +48x^{13}-47x^{14}+25x^{15}-10x^{16}) \\
& +q^{58}x^{14}(5-10x+18x^2-23x^3+35x^4-27x^5+36x^6-38x^7+52x^8-28x^9+21x^{10}+10x^{11}-19x^{12} \\
& +26x^{13}-22x^{14}+17x^{15}-5x^{16}) \\
& +q^{59}x^{15}(2-19x+25x^2-20x^3+17x^4-38x^5+39x^6-40x^7+33x^8-15x^9+10x^{11}-23x^{12}+34x^{13} \\
& -30x^{14}+13x^{15}-4x^{16}) \\
& +q^{52}x^{12}(1-7x+9x^2-16x^3+25x^4-35x^5+36x^6-49x^7+29x^8-27x^9+18x^{10}-4x^{11}-10x^{12} \\
& +22x^{13}-24x^{14}+16x^{15}-4x^{16}) \\
& +q^{41}x^9(5-9x+4x^2-10x^3+18x^4-43x^5+32x^6-35x^7+24x^8-30x^9+18x^{10}-15x^{11}+4x^{12} \\
& +x^{13}-7x^{14}-2x^{16}) \\
& +q^{50}x^{12}(5-11x+19x^2-21x^3+38x^4-29x^5+38x^6-35x^7+48x^8-26x^9+17x^{10}+4x^{11}-10x^{12} \\
& +11x^{13}-10x^{14}+8x^{15}-x^{16}) \\
& +q^{94}x^{25}(-1+6x-3x^2+9x^3-21x^4+31x^5-19x^6+33x^7-18x^8-6x^9+25x^{10}-45x^{11}+60x^{12} \\
& -67x^{13}+32x^{14}-14x^{15}+x^{16}) \\
& +q^{54}x^{13}(-5+10x-19x^2+22x^3-36x^4+28x^5-39x^6+37x^7-51x^8+26x^9-19x^{10}-6x^{11}+15x^{12} \\
& -18x^{13}+19x^{14}-12x^{15}+x^{16}) \\
& +q^{55}x^{14}(-3+21x-27x^2+18x^3-20x^4+37x^5-42x^6+41x^7-33x^8+14x^9+5x^{10}-6x^{11}+19x^{12} \\
& -26x^{13}+23x^{14}-8x^{15}+x^{16}) \\
& +q^{48}x^{11}(-1+7x-10x^2+17x^3-25x^4+34x^5-35x^6+46x^7-30x^8+25x^9-17x^{10}+4x^{11}+7x^{12} \\
& -15x^{13}+20x^{14}-9x^{15}+2x^{16}) \\
& +q^{45}x^{10}(-5+10x-3x^2+10x^3-22x^4+46x^5-33x^6+40x^7-25x^8+34x^9-21x^{10}+19x^{11}-2x^{12} \\
& -5x^{13}+12x^{14}-4x^{15}+4x^{16}) \\
& +q^{63}x^{16}(-1+18x-22x^2+20x^3-16x^4+36x^5-36x^6+44x^7-29x^8+18x^9+x^{10}-15x^{11}+26x^{12} \\
& -42x^{13}+37x^{14}-19x^{15}+7x^{16}) \\
& +q^{71}x^{18}(-1+16x-16x^2+14x^3-11x^4+32x^5-33x^6+42x^7-27x^8+20x^9+3x^{10}-11x^{11}+38x^{12} \\
& -49x^{13}+55x^{14}-30x^{15}+14x^{16}) \\
& +q^{61}x^{14}(-5+9x-6x^2+8x^3-18x^4+36x^5-35x^6+46x^7-30x^8+33x^9-27x^{10}+25x^{11}+7x^{12} \\
& -19x^{13}+35x^{14}-31x^{15}+19x^{16}-8x^{17}) \\
& +q^{53}x^{12}(-5+11x-4x^2+9x^3-21x^4+45x^5-37x^6+43x^7-28x^8+35x^9-25x^{10}+29x^{11}+5x^{12} \\
& -9x^{13}+27x^{14}-14x^{15}+10x^{16}-4x^{17}) \\
& +q^{84}x^{21}(-6+x-7x^2+4x^3-17x^4+26x^5-37x^6+21x^7-26x^8+25x^9-5x^{10}-25x^{11}+50x^{12}
\end{aligned}$$

$$\begin{aligned}
& -68x^{13} + 69x^{14} - 51x^{15} + 24x^{16} - 3x^{17}) \\
& + q^{75}x^{19} (1 - 14x + 13x^2 - 11x^3 + 10x^4 - 30x^5 + 30x^6 - 40x^7 + 24x^8 - 19x^9 - 3x^{10} + 12x^{11} - 42x^{12} \\
& + 49x^{13} - 58x^{14} + 35x^{15} - 18x^{16} + x^{17}) \\
& - q^{62}x^{15} (5 - 9x + 15x^2 - 24x^3 + 32x^4 - 26x^5 + 34x^6 - 41x^7 + 50x^8 - 31x^9 + 22x^{10} + 11x^{11} - 27x^{12} \\
& + 32x^{13} - 27x^{14} + 27x^{15} - 9x^{16} + x^{17}) \\
& - q^{79}x^{20} (1 - 10x + 12x^2 - 8x^3 + 9x^4 - 31x^5 + 30x^6 - 38x^7 + 23x^8 - 19x^9 - 6x^{10} + 13x^{11} - 44x^{12} \\
& + 51x^{13} - 60x^{14} + 39x^{15} - 21x^{16} + 2x^{17}) \\
& + q^{80}x^{20} (6 - 2x + 9x^2 - 5x^3 + 19x^4 - 29x^5 + 35x^6 - 22x^7 + 26x^8 - 23x^9 + 6x^{10} + 25x^{11} - 48x^{12} \\
& + 65x^{13} - 66x^{14} + 46x^{15} - 21x^{16} + 2x^{17}) \\
& + q^{60}x^{14} (1 - 7x + 8x^2 - 13x^3 + 20x^4 - 33x^5 + 37x^6 - 48x^7 + 33x^8 - 22x^9 + 23x^{10} - 5x^{11} - 16x^{12} \\
& + 26x^{13} - 39x^{14} + 31x^{15} - 14x^{16} + 2x^{17}) \\
& - q^{56}x^{13} (1 - 7x + 9x^2 - 15x^3 + 22x^4 - 34x^5 + 37x^6 - 49x^7 + 30x^8 - 25x^9 + 21x^{10} - 6x^{11} - 13x^{12} \\
& + 25x^{13} - 29x^{14} + 24x^{15} - 8x^{16} + 2x^{17}) \\
& + q^{49}x^{11} (5 - 11x + 3x^2 - 10x^3 + 22x^4 - 45x^5 + 36x^6 - 42x^7 + 26x^8 - 37x^9 + 22x^{10} - 26x^{11} - x^{12} \\
& + 7x^{13} - 17x^{14} + 9x^{15} - 6x^{16} + 2x^{17}) \\
& + q^{83}x^{21} (1 - 7x + 10x^2 - 4x^3 + 8x^4 - 27x^5 + 30x^6 - 33x^7 + 23x^8 - 21x^9 - 8x^{10} + 13x^{11} - 44x^{12} \\
& + 53x^{13} - 62x^{14} + 43x^{15} - 23x^{16} + 3x^{17}) \\
& - q^{64}x^{15} (1 - 6x + 7x^2 - 11x^3 + 17x^4 - 28x^5 + 35x^6 - 47x^7 + 34x^8 - 22x^9 + 23x^{10} - 4x^{11} - 15x^{12} \\
& + 29x^{13} - 47x^{14} + 40x^{15} - 21x^{16} + 3x^{17}) \\
& - q^{70}x^{17} (5 - 7x + 11x^2 - 20x^3 + 25x^4 - 24x^5 + 31x^6 - 38x^7 + 42x^8 - 38x^9 + 28x^{10} + 9x^{11} - 35x^{12} \\
& + 40x^{13} - 44x^{14} + 35x^{15} - 19x^{16} + 3x^{17}) \\
& + q^{66}x^{16} (5 - 8x + 13x^2 - 22x^3 + 29x^4 - 24x^5 + 33x^6 - 40x^7 + 45x^8 - 36x^9 + 24x^{10} + 9x^{11} - 32x^{12} \\
& + 35x^{13} - 36x^{14} + 30x^{15} - 13x^{16} + 3x^{17}) \\
& + q^{88}x^{22} (4 + 5x^2 - 4x^3 + 17x^4 - 24x^5 + 36x^6 - 16x^7 + 27x^8 - 25x^9 + 9x^{10} + 19x^{11} - 53x^{12} \\
& + 73x^{13} - 72x^{14} + 55x^{15} - 26x^{16} + 4x^{17}) \\
& - q^{87}x^{22} (1 - 4x + 6x^2 - 4x^3 + 8x^4 - 23x^5 + 33x^6 - 28x^7 + 23x^8 - 16x^9 - 9x^{10} + 15x^{11} - 42x^{12} \\
& + 56x^{13} - 65x^{14} + 47x^{15} - 24x^{16} + 4x^{17}) \\
& - q^{92}x^{23} (3 + 3x^2 - 4x^3 + 18x^4 - 18x^5 + 32x^6 - 15x^7 + 27x^8 - 26x^9 + 9x^{10} + 21x^{11} - 51x^{12} \\
& + 73x^{13} - 71x^{14} + 60x^{15} - 26x^{16} + 5x^{17}) \\
& + q^{74}x^{18} (5 - 5x + 9x^2 - 19x^3 + 20x^4 - 21x^5 + 29x^6 - 40x^7 + 37x^8 - 38x^9 + 30x^{10} + 7x^{11} - 31x^{12} \\
& + 44x^{13} - 49x^{14} + 42x^{15} - 23x^{16} + 5x^{17}) \\
& + q^{68}x^{16} (1 - 6x + 6x^2 - 11x^3 + 14x^4 - 24x^5 + 32x^6 - 43x^7 + 34x^8 - 22x^9 + 19x^{10} - 5x^{11} - 19x^{12} \\
& + 33x^{13} - 52x^{14} + 46x^{15} - 30x^{16} + 6x^{17}) \\
& + q^{91}x^{23} (1 - x + 4x^2 - 3x^3 + 6x^4 - 19x^5 + 35x^6 - 25x^7 + 20x^8 - 13x^9 - 8x^{10} + 18x^{11} - 39x^{12} \\
& + 59x^{13} - 68x^{14} + 47x^{15} - 25x^{16} + 6x^{17})
\end{aligned}$$

$$\begin{aligned}
& + q^{57}x^{13} (5 - 10x + 5x^2 - 8x^3 + 21x^4 - 42x^5 + 34x^6 - 45x^7 + 29x^8 - 34x^9 + 29x^{10} - 27x^{11} - 7x^{12} \\
& + 13x^{13} - 32x^{14} + 21x^{15} - 15x^{16} + 6x^{17}) \\
& - q^{78}x^{19} (4 - 3x + 8x^2 - 17x^3 + 17x^4 - 18x^5 + 29x^6 - 39x^7 + 35x^8 - 36x^9 + 29x^{10} + 3x^{11} - 31x^{12} \\
& + 47x^{13} - 53x^{14} + 49x^{15} - 28x^{16} + 7x^{17}) \\
& + q^{96}x^{24} (2 - 5x^3 + 18x^4 - 15x^5 + 27x^6 - 15x^7 + 28x^8 - 24x^9 + 11x^{10} + 20x^{11} - 47x^{12} + 76x^{13} \\
& - 71x^{14} + 61x^{15} - 25x^{16} + 7x^{17}) \\
& - q^{100}x^{25} (1 - 5x^3 + 17x^4 - 17x^5 + 21x^6 - 15x^7 + 28x^8 - 22x^9 + 14x^{10} + 21x^{11} - 44x^{12} + 76x^{13} \\
& - 71x^{14} + 58x^{15} - 24x^{16} + 7x^{17}) \\
& + q^{93}x^{23} (1 + 3x^2 - 2x^3 + 13x^4 - 16x^5 + 30x^6 - 11x^7 + 31x^8 - 35x^9 + 20x^{10} + 12x^{11} - 27x^{12} \\
& + 61x^{13} - 72x^{14} + 59x^{15} - 34x^{16} + 13x^{17}) \\
& - q^{89}x^{22} (2 + 4x^2 - 3x^3 + 16x^4 - 17x^5 + 34x^6 - 12x^7 + 30x^8 - 36x^9 + 20x^{10} + 12x^{11} - 27x^{12} \\
& + 60x^{13} - 68x^{14} + 62x^{15} - 32x^{16} + 13x^{17}) \\
& + q^{73}x^{17} (4 - 6x + 3x^2 - 6x^3 + 12x^4 - 25x^5 + 29x^6 - 38x^7 + 28x^8 - 27x^9 + 32x^{10} - 21x^{11} - 8x^{12} \\
& + 32x^{13} - 45x^{14} + 51x^{15} - 44x^{16} + 18x^{17} - 6x^{18}) \\
& + q^{65}x^{15} (5 - 8x + 6x^2 - 7x^3 + 15x^4 - 32x^5 + 33x^6 - 43x^7 + 31x^8 - 31x^9 + 29x^{10} - 25x^{11} - 8x^{12} \\
& + 24x^{13} - 36x^{14} + 37x^{15} - 27x^{16} + 12x^{17} - 2x^{18}) \\
& + q^{76}x^{18} (1 - 6x + 3x^2 - 11x^3 + 8x^4 - 20x^5 + 30x^6 - 38x^7 + 29x^8 - 23x^9 + 21x^{10} - 4x^{11} - 26x^{12} \\
& + 42x^{13} - 62x^{14} + 62x^{15} - 42x^{16} + 15x^{17} - 2x^{18}) \\
& + q^{82}x^{20} (3 - 2x + 5x^2 - 15x^3 + 14x^4 - 14x^5 + 27x^6 - 36x^7 + 33x^8 - 33x^9 + 26x^{10} + 4x^{11} - 29x^{12} \\
& + 45x^{13} - 56x^{14} + 58x^{15} - 28x^{16} + 9x^{17} - x^{18}) \\
& + q^{90}x^{22} (1 + 2x^2 - 9x^3 + 5x^4 - 10x^5 + 24x^6 - 32x^7 + 26x^8 - 33x^9 + 23x^{10} + 4x^{11} - 25x^{12} + 47x^{13} \\
& - 60x^{14} + 65x^{15} - 30x^{16} + 15x^{17} - x^{18}) \\
& + q^{86}x^{21} (-2 + x - 3x^2 + 14x^3 - 10x^4 + 11x^5 - 27x^6 + 33x^7 - 31x^8 + 34x^9 - 26x^{10} - 4x^{11} + 27x^{12} \\
& - 47x^{13} + 60x^{14} - 64x^{15} + 28x^{16} - 13x^{17} + x^{18}) \\
& + q^{72}x^{17} (-1 + 6x - 4x^2 + 11x^3 - 11x^4 + 22x^5 - 30x^6 + 39x^7 - 34x^8 + 21x^9 - 17x^{10} + 6x^{11} + 23x^{12} \\
& - 36x^{13} + 57x^{14} - 53x^{15} + 38x^{16} - 10x^{17} + 2x^{18}) \\
& + q^{69}x^{16} (-5 + 7x - 4x^2 + 6x^3 - 14x^4 + 28x^5 - 32x^6 + 43x^7 - 31x^8 + 29x^9 - 29x^{10} + 22x^{11} + 7x^{12} \\
& - 29x^{13} + 40x^{14} - 44x^{15} + 35x^{16} - 15x^{17} + 4x^{18}) \\
& + q^{77}x^{18} (-3 + 6x - 2x^2 + 6x^3 - 10x^4 + 23x^5 - 26x^6 + 37x^7 - 25x^8 + 27x^9 - 32x^{10} + 18x^{11} + 10x^{12} \\
& - 29x^{13} + 52x^{14} - 56x^{15} + 55x^{16} - 21x^{17} + 8x^{18}) \\
& + q^{85}x^{20} (-1 + 3x + 6x^3 - 5x^4 + 18x^5 - 21x^6 + 37x^7 - 17x^8 + 28x^9 - 34x^{10} + 20x^{11} + 10x^{12} - 28x^{13} \\
& + 62x^{14} - 65x^{15} + 62x^{16} - 29x^{17} + 12x^{18}) \\
& - q^{81}x^{19} (-2 + 5x + 6x^3 - 8x^4 + 19x^5 - 24x^6 + 37x^7 - 23x^8 + 29x^9 - 32x^{10} + 20x^{11} + 9x^{12} - 27x^{13} \\
& + 60x^{14} - 62x^{15} + 61x^{16} - 25x^{17} + 12x^{18}) \\
& - q^{176} (x^{56} + 2x^{58})]
\end{aligned}$$

$$\begin{aligned}
h_2 = & q^{299} x^3 [-1 + (1 + q + q^2 + q^3 + q^4 + q^5 + q^6) x \\
& - q (1 + q + 2q^2 + 2q^3 + 3q^4 + 3q^5 + 3q^6 + 2q^7 + 2q^8 + q^9 + q^{10}) x^2 \\
& + q^3 (1 + q + 2q^2 + 3q^3 + 4q^4 + 4q^5 + 5q^6 + 4q^7 + 4q^8 + 3q^9 + 2q^{10} + q^{11} + q^{12}) x^3 \\
& - q^6 (1 + q + 2q^2 + 3q^3 + 4q^4 + 4q^5 + 5q^6 + 4q^7 + 4q^8 + 3q^9 + 2q^{10} + q^{11} + q^{12}) x^4 \\
& + q^{10} (1 + q + 2q^2 + 2q^3 + 3q^4 + 3q^5 + 3q^6 + 2q^7 + 2q^8 + q^9 + q^{10}) x^5 \\
& - q^{15} (1 + q + q^2 + q^3 + q^4 + q^5 + q^6) x^6 + q^{21} x^7]^2 \times \\
& [-1 + qx^2 + q^2 x^3 - q^8 x^4 - q^3 x^5 + q^4 x^5 - q^6 x^5 + 2q^{212} x^{71} + q^{213} x^{71} + q^{215} x^{72} \\
& - q^{211} (-1 + x) x^{72} - q^{214} x^{73} - q^{216} x^{74} - q^{222} x^{74} + q^{227} x^{76} - q^{220} x^{73} (1 + x) \\
& + q^{209} x^{71} (2 + x) + q^{210} x^{69} (-1 + 2x) - 2q^{191} x^{64} (1 - x + x^2) - 2q^{202} x^{66} (-1 + x^3) \\
& + q^{204} x^{68} (-1 + x^2 + x^3) + q^{207} x^{68} (-2 - x + x^2 + x^3) + q^{203} x^{67} (-1 + x^4) \\
& + q^{206} x^{67} (-1 - x^2 + x^4) - q^{192} x^{62} (1 - 3x^3 + x^4) + q^{193} x^{64} (1 + x^2 - 3x^4 - x^5) \\
& - q^{182} x^{57} (1 - x^2 + x^5) + q^{178} x^{59} (-1 + x + x^2 - 2x^3 + x^5) + q^{13} x^6 (-1 - x^4 + x^5) \\
& + q^{12} x^5 (-2 + x^2 + x^4 + x^5) - q^{11} x^3 (-1 + x^2 + x^4 + x^5) - q^{197} x^{63} (1 - x^3 + 3x^4 + x^5) \\
& + q^{196} x^{62} (-1 + x^4 + x^5 - 2x^6) + q^7 (x^2 - x^6) + q^{189} x^{61} (1 - x - 4x^2 + x^3 + x^5 - x^6) \\
& + q^{180} x^{59} (1 - x - 2x^2 + x^3 + x^4 + 2x^5 - x^6) + q^{10} x^4 (-1 + x^6) \\
& - q^{187} x^{60} (-2 + 2x^2 - 2x^4 + x^6) + q^{190} x^{63} (-1 + 3x + x^2 - x^4 + x^6) \\
& - q^{166} x^{54} (1 + x - x^3 - x^4 - 2x^5 + x^6) + q^{188} x^{62} (-2 + x^3 - x^5 + x^6) \\
& - q^{201} x^{65} (-1 + x^3 + x^4 - x^5 + x^6) + q^{194} x^{63} (-1 + 2x^2 + 4x^3 - 3x^4 + x^5 + x^6) \\
& + q^5 (x^3 - x^7) - q^{18} x^8 (1 - x - 2x^2 - x^3 + x^4 + x^7) + q^{23} x^{10} (-2 + x - 2x^3 - x^4 + x^5 + x^7) \\
& - q^{173} x^{57} (-1 + 2x^2 - 3x^3 + 3x^4 - 3x^6 + x^7) + q^{17} x^6 (1 + 2x^2 + x^3 + x^4 - x^6 + x^7) \\
& + q^{26} x^7 (1 + 2x - 2x^3 - x^4 - 4x^5 - x^6 + x^7) - q^{181} x^{59} (1 - 2x + 2x^2 + x^3 + x^4 - 6x^5 + x^6 + x^7) \\
& - q^{24} x^9 (-1 - 2x + x^3 + x^5 + x^6 + x^7) - q^{19} x^6 (1 - x^4 + 2x^6 + x^7) \\
& + q^{172} x^{57} (1 + 2x^2 + x^3 - 3x^5 + 2x^6 + x^7) + q^{167} x^{56} (-1 + 2x + 2x^2 + 3x^3 - x^4 - 2x^5 + x^6 + 2x^7) \\
& + q^{154} x^{51} (1 + x + 4x^2 - x^3 - 5x^4 - 5x^5 - 2x^6 + x^7 - 6x^8) \\
& + q^{158} x^{52} (1 + x - 4x^2 - x^3 + x^4 - 3x^5 + 4x^6 - 2x^8) \\
& + q^{185} x^{59} (1 + x + x^4 + x^5 - x^6 - x^8) + q^{22} x^7 (1 + 2x - x^2 + x^4 + x^5 - x^6 - x^8) \\
& + q^{176} x^{58} (1 + 2x^2 - 2x^3 - 4x^4 + x^5 + 2x^6 - x^8) + q^{20} x^5 (-2 + x^4 + x^5 + x^6 + x^7 - x^8) \\
& + q^{200} x^{63} (-1 + 2x^2 - x^5 + x^8) + q^{195} x^{60} (1 + x^5 + x^8) - q^{16} x^4 (1 + 2x^2 + x^3 - 2x^6 + x^8) \\
& + q^{170} x^{56} (-1 + 2x + 3x^2 + 2x^3 - 2x^5 - 2x^6 + x^8) + q^{198} x^{62} (-1 - x^7 + x^8) \\
& - q^{15} (x^5 - x^7 + x^8) + q^{31} x^{10} (-2 - x - x^2 - 3x^3 + 4x^5 - x^6 - x^7 + x^8) \\
& - q^{184} x^{58} (1 - x^2 + 2x^4 - 2x^5 - 2x^6 + x^7 + x^8) - 2q^{48} x^{19} (2 - 2x + x^2 - x^4 + x^6 + x^7 + x^8) \\
& + q^{175} x^{56} (-1 + x + 2x^3 - 4x^4 - x^5 - x^6 + 2x^7 + x^8) - q^{183} x^{59} (-1 + x^2 + x^3 + 2x^4 + x^5 - 4x^6 + 3x^7 + x^8) \\
& + q^{169} x^{55} (-2 + x^3 + 2x^4 - 2x^5 - 3x^6 + x^7 + 2x^8) + q^{177} x^{57} (1 + x^2 - 2x^4 - x^5 + x^7 - x^9)
\end{aligned}$$

$$\begin{aligned}
& + q^{165} x^{53} (-1 - 2x^2 + x^4 + 2x^5 + 5x^6 + 2x^7 + x^8 - x^9) \\
& + q^{171} x^{55} (1 + x - x^2 + x^3 + 3x^4 - 3x^6 + 3x^7 + x^9) \\
& - q^{156} x^{51} (-1 - 2x + 4x^3 + x^4 + 2x^5 + 2x^6 - 4x^8 + x^9) \\
& + q^{162} x^{53} (1 - x - 2x^2 - x^3 + 2x^4 + 2x^5 + x^6 - 2x^7 - x^8 + x^9) \\
& - q^{179} x^{57} (1 - x + 4x^3 + 3x^5 - x^6 - x^7 + x^8 + x^9) - q^{21} x^5 (1 - 3x^2 - x^4 - x^5 + x^6 + x^7 + x^8 + x^9) \\
& - q^{157} x^{51} (1 - 2x - 2x^2 + 2x^3 + 4x^4 - 3x^5 - 5x^7 + 3x^8 + x^9) \\
& + q^{142} x^{48} (-1 - 3x + 4x^2 + 4x^3 + x^4 + 3x^5 + 4x^6 + x^7 + 3x^8 + 2x^9) \\
& + q^{160} x^{50} (1 + x^3 - 2x^4 - 5x^5 - 2x^7 - 2x^8 + x^9 - 4x^{10}) \\
& + q^{149} x^{48} (-1 + x^2 + x^3 + 4x^4 + 3x^5 - x^6 - 3x^9 - 3x^{10}) \\
& + q^{127} x^{42} (-1 - x^2 + 4x^3 + x^4 - 2x^5 - 2x^6 + x^7 + 3x^8 + 7x^9 - 3x^{10}) \\
& + q^{28} x^{10} (-1 - 2x + x^5 + x^7 - x^{10}) + q^9 (x^2 - x^8 + x^{10}) \\
& - q^{145} x^{48} (3 + x + 2x^2 - 3x^3 - 2x^4 - 2x^5 - 2x^6 + x^7 + x^8 + x^{10}) \\
& - q^{174} x^{55} (1 - x^3 + x^4 + x^5 + 5x^6 + 2x^7 - 3x^8 - x^9 + x^{10}) \\
& + q^{40} x^{15} (4 - 6x^2 + x^4 - x^5 + 2x^7 + x^8 - x^9 + x^{10}) + q^{27} x^8 (1 + x - x^2 - 2x^3 - x^4 - x^7 + x^9 + x^{10}) \\
& + q^{168} x^{53} (1 + x^4 + 4x^5 - 4x^7 - 6x^8 + x^9 + x^{10}) - q^{33} x^9 (1 + x^2 + x^3 - x^5 + x^6 - 3x^7 - 2x^8 + 3x^{10}) \\
& + q^{137} x^{46} (1 - x - 8x^2 - 3x^3 - 2x^5 - 5x^6 + x^7 - 4x^8 - x^9 + 3x^{10}) \\
& + q^{151} x^{48} (-2 + x^2 + x^4 + 3x^5 - 4x^6 - 7x^7 - 7x^8 + 3x^9 - 2x^{10} - x^{11}) \\
& + q^{153} x^{49} (-1 + 3x^2 + 3x^3 - 2x^4 + x^5 + 2x^6 - 5x^7 + 2x^8 + 4x^9 - 2x^{10} - x^{11}) \\
& + q^{30} x^8 (1 + x^2 + x^3 - 3x^4 - 2x^5 + x^6 + 3x^7 + x^8 + x^9 + x^{10} - x^{11}) \\
& + q^{161} x^{51} (1 - 2x^3 - 3x^4 - 2x^5 + 5x^6 + 3x^7 + 5x^8 - 2x^{10} + x^{11}) \\
& + q^{164} x^{51} (1 - x^2 - x^4 - 2x^5 + 7x^7 - x^8 - 4x^9 - x^{10} + x^{11}) \\
& + q^{122} x^{42} (-5 - x + x^2 + 5x^4 + x^5 - 10x^6 + 4x^7 - 2x^8 + 2x^9 - x^{10} + x^{11}) \\
& + q^{131} x^{44} (3 - x + 2x^2 + 5x^3 - 2x^4 - 7x^5 - 3x^6 - 6x^7 + 2x^8 - 8x^9 + x^{10} + x^{11}) \\
& + q^{163} x^{52} (1 + x - 3x^3 + 4x^5 + 3x^6 + x^7 + 4x^8 - 2x^9 + x^{10} + x^{11}) \\
& + q^{29} x^7 (1 + 3x^3 + x^4 - x^5 - 2x^6 + x^7 + 2x^8 + x^9 + x^{10} + x^{11}) \\
& - q^{152} x^{49} (1 + 2x - x^3 + x^4 + 3x^6 + 2x^7 + x^8 + 3x^9 + x^{10} + x^{11}) \\
& + q^{138} x^{46} (-1 + x^2 - 4x^3 - 6x^4 + 2x^5 + 4x^6 + 5x^7 + 2x^8 + 2x^9 + 4x^{10} + x^{11}) \\
& + q^{136} x^{45} (1 + 3x - x^3 - 2x^4 + 2x^7 + x^8 + 3x^9 + 4x^{10} + x^{11}) \\
& + q^{141} x^{46} (1 + x - 5x^3 - 5x^4 - 4x^5 + 7x^6 - 2x^7 + x^8 - x^9 + 5x^{10} + x^{11}) \\
& - q^{132} x^{43} (1 - 2x^2 + x^3 - x^4 + 3x^5 - 6x^6 + 6x^7 - 2x^8 - 2x^9 + 3x^{11}) \\
& - q^{43} x^{13} (1 - 2x^2 - x^3 + 2x^4 + x^5 - x^6 + x^7 - 3x^9 + x^{10} + 3x^{11}) \\
& - q^{129} x^{43} (1 + x - 5x^2 - x^3 - x^4 + x^5 - 2x^6 - 3x^7 - 4x^8 + 4x^9 + 5x^{10} + 3x^{11}) \\
& + q^{118} x^{39} (2 + 2x - 3x^2 + 2x^3 - 4x^4 - 7x^5 - 5x^6 - 4x^7 - 2x^8 - x^9 - 4x^{10} + 7x^{11}) \\
& + q^{34} x^8 (1 - x^2 + x^3 + x^6 + x^7 + x^8 - 2x^{10} - x^{11} - 4x^{12}) \\
& + q^{99} x^{33} (1 + 4x - 7x^3 - 4x^4 + 2x^5 - 3x^6 + x^7 + x^8 - 3x^9 - 8x^{10} + 2x^{11} - 4x^{12})
\end{aligned}$$

$$\begin{aligned}
& + q^{124}x^{41}(-1-2x-x^2-2x^3+4x^4+6x^5+x^6-3x^7+2x^8+5x^9+x^{10}-3x^{12}) \\
& + q^{42}x^{13}(1+x+x^2+x^4-4x^5-x^6+2x^7+3x^8+x^9+2x^{10}-x^{12}) \\
& + q^{144}x^{46}(1-x-4x^4+5x^5+4x^6+3x^7+x^8+5x^{10}-x^{12}) \\
& + q^{44}x^{14}(1+x+x^2-2x^3-x^4-2x^6+x^7+6x^8-2x^{11}-x^{12}) \\
& + q^{140}x^{45}(1+2x-4x^3-2x^4+6x^6+x^8+2x^{10}+3x^{11}-x^{12}) \\
& + q^{135}x^{43}(-1+6x^2-x^3-2x^4-3x^5-4x^6-7x^7-2x^8-x^9-x^{10}-5x^{11}+x^{12}) \\
& - q^{38}x^{11}(1+x+x^2-2x^3-x^4+x^5+x^6+x^8-3x^{11}+x^{12}) \\
& + q^{35}x^{10}(-1-x^3+2x^4+x^5-2x^{10}-x^{11}+x^{12}) \\
& + q^{53}x^{18}(-1-x+2x^3+2x^4-5x^5-4x^6+x^7-2x^8+2x^9+x^{10}-x^{11}+x^{12}) \\
& + q^{109}x^{37}(-2-x+x^2+2x^3-x^4+2x^5+3x^6+x^7+5x^8+7x^9+x^{11}+x^{12}) \\
& + q^{155}x^{49}(-1-x+2x^3-2x^4-2x^6-3x^7+2x^8+3x^9-2x^{10}+x^{11}+x^{12}) \\
& + q^{106}x^{37}(-1+6x^2-x^3-x^4-8x^5-3x^7+3x^8+3x^9+2x^{12}) \\
& + q^{52}x^{17}(-1-x^4-x^6+5x^9+2x^{12}) + q^{37}x^{10}(-2+x^4+4x^5+2x^6-x^7+2x^8-3x^{10}+2x^{12}) \\
& + q^{133}x^{43}(1-x+x^2+2x^3+3x^4-5x^5-6x^6-5x^8+2x^{10}-5x^{11}+2x^{12}) \\
& - q^{147}x^{47}(1+x^2+x^3-x^4-7x^5+5x^6-2x^8-2x^9-x^{11}+2x^{12}) \\
& - q^{59}x^{20}(1-3x^2+5x^3+4x^5+x^7+x^8-2x^9-2x^{10}+x^{11}+2x^{12}) \\
& + q^{55}x^{17}(-1-x+x^2+2x^3+2x^5+2x^6-5x^7-x^8+x^9+3x^{11}+2x^{12}) \\
& + q^{98}x^{33}(2+2x+x^4-4x^5+8x^6-2x^7-10x^9-3x^{10}+4x^{11}+x^{12}-4x^{13}) \\
& + q^{148}x^{46}(1-2x^2+x^3+3x^4+x^6+8x^7-2x^8-5x^9-2x^{10}+2x^{11}-x^{12}-3x^{13}) \\
& + q^{128}x^{41}(1-3x^2+x^3+3x^4+5x^5+2x^6+x^7-3x^8-3x^9+2x^{10}+3x^{11}-5x^{12}-2x^{13}) \\
& + q^{143}x^{45}(2+3x^3-x^5+x^6+x^7+5x^8-2x^9-x^{10}-x^{11}+3x^{12}-2x^{13}) \\
& + q^{146}x^{45}(1-2x^4-5x^5+2x^6+3x^7+5x^8+7x^9+6x^{12}-2x^{13}) \\
& + q^{117}x^{39}(2+x+x^2-3x^3-14x^4+x^5+6x^6+2x^7-2x^8+9x^9-x^{10}+2x^{11}-2x^{12}-x^{13}) \\
& + q^{14}(x^3-x^5+2x^8+x^9+x^{12}-x^{13}) - q^{123}x^{40}(-3-x+x^2+4x^3-x^5-x^6+x^7-11x^8+x^9+x^{13}) \\
& + q^{114}x^{38}(-1+2x+3x^3-2x^4-6x^5+3x^6+3x^7-4x^8-2x^9-6x^{10}+x^{13}) \\
& - q^{104}x^{34}(-1+2x^2+2x^3+x^4-4x^5-6x^6+6x^7-3x^8-5x^{10}-7x^{11}-3x^{12}+x^{13}) \\
& + q^{108}x^{36}(-3+2x^2+2x^3+5x^5+x^6-5x^7+x^8+x^9+x^{10}-2x^{11}-2x^{12}+x^{13}) \\
& + q^{41}x^{11}(-1-x-x^2+x^3+2x^4-4x^6+2x^7+x^8-x^{10}-x^{11}-x^{12}+x^{13}) \\
& + q^{25}x^5(-1-x+2x^3+x^4+2x^5-3x^7-x^8+x^9-x^{10}+x^{11}+x^{12}+x^{13}) \\
& - q^{112}x^{37}(2+x-3x^2-6x^3+4x^5+9x^6+3x^8+x^9+x^{10}+x^{11}+x^{12}+x^{13}) \\
& + q^{130}x^{42}(-3-2x^2-2x^3+9x^4-2x^6+3x^7-x^8-4x^9+4x^{10}+x^{11}+x^{12}+x^{13}) \\
& - q^{125}x^{41}(-1+x+2x^2+x^3-x^4-3x^5-5x^6-2x^7+3x^8+3x^{10}+2x^{12}+x^{13}) \\
& + q^{67}x^{22}(3-3x-2x^2-x^3+5x^4-2x^6-4x^7+3x^8-x^9+7x^{10}+2x^{12}+x^{13}) \\
& + q^{126}x^{41}(-1+x-3x^2+x^3+3x^5-x^6+3x^7+x^8-3x^9+4x^{10}-x^{11}-2x^{12}+2x^{13}) \\
& - q^{150}x^{46}(-1+x^3-x^5-2x^6+x^7+x^8+4x^9+x^{12}+2x^{13})
\end{aligned}$$

$$\begin{aligned}
& + q^{134}x^{43}(-3 - x^2 + x^3 - x^4 + 3x^5 - 4x^6 + 3x^7 - x^8 - x^9 - 4x^{10} - 2x^{11} + 3x^{13}) \\
& - q^{120}x^{39}(-1 - 2x^2 + 2x^3 + 4x^4 - 2x^5 - 3x^6 - 2x^7 + 2x^8 + x^9 + 5x^{10} + 2x^{11} + 3x^{13}) \\
& + q^{119}x^{38}(1 - x + x^3 - 5x^4 + x^6 + 9x^7 + x^8 + 2x^9 + x^{10} - 4x^{11} - 3x^{12} + 3x^{13}) \\
& + q^{159}x^{48}(-1 - x^3 + 2x^5 - x^6 - 2x^7 - 5x^8 + x^{10} + 3x^{11} - 2x^{12} + 4x^{13}) \\
& - q^{100}x^{33}(-2 + x^3 + 7x^4 - 2x^5 + 2x^6 + 2x^7 + 2x^8 - 8x^9 + x^{10} + 2x^{11} + 2x^{12} + 4x^{13}) \\
& + q^{77}x^{26}(-3 + x + 4x^2 + x^3 - 4x^4 + 4x^6 - 2x^8 - 5x^9 - 3x^{10} + x^{11} - 2x^{12} - 2x^{13} - 2x^{14}) \\
& + q^{57}x^{17}(1 - 2x^2 + x^3 + 2x^4 - x^5 - x^6 + x^7 - 2x^8 + x^9 + 2x^{10} + 3x^{11} + x^{12} - 2x^{13} - 2x^{14}) \\
& + q^{72}x^{23}(1 + x - x^2 - x^3 + 4x^4 - x^5 - 5x^6 + x^7 + 6x^8 - 3x^9 - 3x^{10} + x^{11} - 4x^{12} + 5x^{13} - 2x^{14}) \\
& + q^{94}x^{31}(-2 + x + x^2 + x^3 - 4x^5 - 3x^6 - 4x^7 + 5x^8 + 5x^9 - 7x^{10} + 3x^{11} - 2x^{12} - 5x^{13} - x^{14}) \\
& + q^{121}x^{39}(1 + 2x - 2x^2 + x^3 + x^4 - 9x^5 + x^6 + 3x^7 + x^9 + 8x^{10} + 5x^{11} + 5x^{12} - 3x^{13} - x^{14}) \\
& + q^{58}x^{19}(-1 - 3x + 2x^2 + x^3 - 6x^5 + x^6 + 2x^7 + 2x^8 - 5x^9 + 5x^{10} - 4x^{11} - 2x^{13} - x^{14}) \\
& + q^{62}x^{20}(2 + x + 4x^2 + x^3 - x^4 + 3x^5 + 4x^6 - 2x^8 - 2x^9 - 2x^{10} - 2x^{12} + x^{14}) \\
& + q^{102}x^{34}(3 - 6x^2 - x^3 + x^4 - 3x^5 + 2x^6 - x^7 + 4x^8 + 3x^9 + 2x^{10} + x^{11} - x^{12} + x^{14}) \\
& + q^{46}x^{12}(1 + x^3 + x^4 - 3x^5 - 2x^6 - x^9 + 2x^{10} + 2x^{11} + x^{13} + x^{14}) \\
& + q^{39}x^{11}(-1 + 2x^2 + 2x^3 + x^4 - x^5 + x^6 - 3x^7 - 2x^9 + x^{10} + 2x^{12} + x^{13} + x^{14}) \\
& + q^{139}x^{43}(-1 - x + 3x^3 + 3x^4 + x^5 - x^6 + 5x^7 - 6x^8 - 3x^9 + x^{10} - 4x^{11} - x^{12} + 2x^{13} + x^{14}) \\
& + q^{111}x^{36}(-1 - x - x^2 - x^3 + 6x^5 - x^6 + 4x^8 + 7x^9 - 2x^{10} - 3x^{11} - 3x^{12} + 3x^{13} + x^{14}) \\
& - q^{115}x^{37}(2 - 3x^2 - 3x^3 + 6x^4 + x^5 + 2x^6 + 3x^7 - 5x^9 - x^{10} + 3x^{11} + 3x^{12} - 5x^{13} + 2x^{14}) \\
& + q^{49}x^{14}(1 + 2x - 2x^3 + x^4 + 2x^5 - 2x^6 + x^7 - x^8 - x^9 - 2x^{10} - 5x^{11} + x^{12} - 2x^{13} + 2x^{14}) \\
& + q^{51}x^{15}(-1 - 2x^2 - 3x^3 + 4x^5 + x^6 - 3x^7 + x^8 - x^9 - 3x^{10} + x^{11} + x^{12} - x^{13} + 2x^{14}) \\
& + q^{89}x^{29}(-1 + x^2 + 3x^3 + 3x^4 - 2x^5 + x^6 - 4x^7 + x^8 + 2x^{10} - 4x^{11} + 9x^{12} + x^{13} + 2x^{14}) \\
& + q^{101}x^{32}(-1 + x^2 - 5x^4 - 4x^5 - 2x^6 + x^7 + 2x^8 - 6x^9 + 2x^{10} - 3x^{11} + 5x^{12} + 3x^{13} + 2x^{14}) \\
& + q^{64}x^{21}(-1 + x - 4x^3 - x^4 + 4x^5 + 3x^6 + 3x^7 - 2x^8 - 3x^9 - 7x^{10} - x^{11} - x^{12} + 3x^{14}) \\
& - q^{97}x^{31}(1 - 2x^2 - x^3 - x^4 + 5x^6 + 5x^8 + 9x^9 + 3x^{10} + 6x^{11} - 6x^{12} + 6x^{13} + 3x^{14}) \\
& - q^{60}x^{17}(1 + x^2 + x^5 + x^6 + 2x^8 - 4x^{10} + 5x^{12} - x^{13} + 4x^{14}) \\
& + q^{105}x^{34}(1 - 4x^2 - 3x^3 + 2x^4 - 2x^5 - x^6 + 7x^7 - 2x^8 + 5x^9 + 9x^{11} - x^{12} + x^{13} + 4x^{14}) \\
& + q^{45}x^{10}(-1 - x^3 + x^5 + x^6 + 2x^7 - 4x^8 + 3x^9 + 5x^{10} - x^{11} - 3x^{12} + x^{13} - 3x^{15}) \\
& + q^{56}x^{17}(1 - x + 4x^3 + 2x^4 - 3x^5 - 2x^6 - x^7 + 4x^8 + 3x^9 - 3x^{10} + 8x^{11} + x^{13} - 2x^{15}) \\
& + q^{96}x^{31}(-1 + x + 6x^3 + x^5 + 5x^6 + 3x^7 - 6x^8 - 3x^{10} - 2x^{11} + 2x^{12} - x^{13} - 5x^{14} - 2x^{15}) \\
& + q^{90}x^{29}(1 - 2x^2 - 3x^3 - x^5 - 8x^7 + 7x^8 + 10x^9 - 2x^{10} + x^{11} + x^{12} + x^{13} - x^{15}) \\
& + q^{47}x^{13}(1 - x^5 + x^6 + 3x^8 + 2x^9 - 2x^{10} - 5x^{11} + 2x^{12} - 3x^{13} + x^{14} - x^{15}) \\
& + q^{76}x^{25}(-1 + 2x + x^2 - 2x^3 - x^4 + x^5 + 3x^6 + 2x^7 + 3x^8 - x^9 - x^{10} - 3x^{12} - x^{13} + x^{15}) \\
& - q^{32}x^7(-1 + x^4 + x^5 + x^6 + x^7 - 2x^8 + x^9 - x^{11} + x^{12} + x^{13} + x^{15}) \\
& + q^{36}x^8(1 - x^3 - x^4 - x^5 - x^8 - 2x^9 + 2x^{12} + x^{13} + x^{15}) \\
& - q^{93}x^{30}(3 + 2x - x^2 - 3x^3 - 7x^4 + 4x^6 + 5x^7 + x^8 - 2x^9 + 5x^{10} + 4x^{11} + x^{12} + 4x^{13} + x^{15})
\end{aligned}$$



$$\begin{aligned}
& + q^{78} x^{24} (-1 + 3x^3 + x^4 - 3x^5 + x^6 + 3x^7 + 2x^8 - 4x^9 + 7x^{10} - 2x^{11} - 6x^{12} - 3x^{13} - 4x^{14} + x^{15}) \\
& - q^{113} x^{36} (1 - 3x^2 + x^3 - 3x^4 - x^5 - x^6 - 4x^7 + x^8 + x^9 - 5x^{10} + x^{11} + 4x^{12} - 5x^{13} - x^{14} + x^{15}) \\
& + q^{50} x^{13} (1 - 2x^4 - x^5 + x^6 - x^7 + 3x^8 + x^9 - x^{10} - 2x^{13} + x^{14} + x^{15}) \\
& - q^{95} x^{31} (-1 + 3x - 6x^2 - 5x^3 - 2x^5 - 3x^6 + 3x^7 - x^8 + x^9 + 3x^{10} + 5x^{11} + x^{12} + 2x^{13} + x^{14} + x^{15}) \\
& - q^{74} x^{24} (2 - x + x^2 + x^3 + 6x^6 + 4x^7 - 2x^8 - 2x^9 + 6x^{10} + 3x^{12} + 2x^{14} + x^{15}) \\
& + q^{79} x^{26} (1 - x^2 + 6x^3 + x^4 - 3x^5 - x^6 + 3x^7 - x^8 - x^9 + x^{11} - 3x^{12} - 3x^{13} + 2x^{14} + x^{15}) \\
& + q^{107} x^{34} (1 - x^2 - 6x^3 - 3x^4 + 3x^5 + 8x^6 - x^8 + 2x^9 + 6x^{10} - 9x^{11} + 4x^{12} - x^{13} + 4x^{14} + x^{15}) \\
& + q^{103} x^{33} (2 - x^3 + x^4 - 3x^5 + 4x^6 + 3x^8 - 5x^9 + 6x^{10} + x^{12} - 4x^{13} + 2x^{15}) \\
& - q^{116} x^{36} (1 - 2x^3 - x^4 - 5x^5 + 2x^6 + x^7 + 4x^8 + 5x^9 + 8x^{10} + 2x^{11} + 8x^{12} - x^{13} - x^{14} + 2x^{15}) \\
& + q^{88} x^{28} (3 + x - 2x^2 - 3x^3 + 6x^5 + 5x^6 + 5x^8 + 5x^9 + 7x^{10} + 7x^{11} + 7x^{12} - 3x^{13} + x^{14} + 2x^{15}) \\
& + q^{65} x^{19} (-1 + x - 3x^3 + x^4 - 2x^5 - 3x^8 - 3x^{11} + x^{13} + x^{14} + 2x^{15}) \\
& + q^{66} x^{21} (1 + x^3 - x^5 + 2x^6 - 4x^7 - x^8 - 2x^9 + 2x^{10} - 4x^{11} + 2x^{12} - x^{13} + 2x^{14} + 2x^{15}) \\
& + q^{110} x^{34} (1 - x^2 - 2x^3 + 2x^4 + 3x^5 + 5x^6 + 3x^7 + x^8 - x^9 - 2x^{11} - 9x^{12} + 4x^{14} + 4x^{15}) \\
& + q^{75} x^{23} (1 - x - 6x^2 + x^3 + 3x^4 + 3x^5 - 6x^6 + 2x^7 + 4x^8 + 2x^9 + 3x^{11} - 3x^{12} + 2x^{13} - 5x^{15} - 2x^{16}) \\
& + q^{92} x^{29} (-1 - 2x^2 - 2x^3 + x^4 + x^6 + 2x^7 - 2x^8 + x^9 + 7x^{10} - 4x^{11} + 4x^{12} + 4x^{13} - x^{15} - 2x^{16}) \\
& + q^{69} x^{21} (1 - x^2 + x^3 - 5x^4 + 9x^6 - 2x^7 - 3x^8 - 3x^{10} + x^{12} + 3x^{13} + 2x^{14} + 2x^{15} - 2x^{16}) \\
& + q^{54} x^{15} (1 - x^2 - 2x^3 + x^4 + 4x^5 + x^6 + x^8 + x^9 - x^{10} - x^{11} + 4x^{12} - x^{16}) \\
& + q^{73} x^{22} (2 - 3x^2 - x^3 + x^4 - x^5 - x^6 + x^8 + 3x^9 - x^{10} + x^{11} + 5x^{12} + 2x^{13} + x^{14} - 4x^{15} - x^{16}) \\
& - q^{80} x^{25} (1 - 3x^2 - 4x^3 + 4x^4 + 5x^5 + 3x^6 - 4x^7 - 2x^8 + 4x^9 - x^{11} - 2x^{13} + 5x^{14} - 3x^{15} + x^{16}) \\
& + q^{63} x^{19} (1 + x^2 + 2x^4 - x^5 + x^7 + 5x^8 + 2x^9 - x^{10} + x^{11} + x^{12} - 2x^{13} + 2x^{14} + 2x^{16}) \\
& + q^{61} x^{18} (-1 + x - x^2 + x^3 - x^4 - 3x^5 - x^6 + 2x^7 + 3x^8 - 2x^9 - 2x^{10} + 3x^{11} - 3x^{13} - 3x^{15} + 2x^{16}) \\
& + q^{83} x^{25} (-2 + x^3 - x^4 - 2x^5 - 2x^6 + 2x^7 - 3x^8 + 2x^9 - 4x^{10} + 5x^{11} - 4x^{12} + x^{13} + 2x^{14} + x^{15} + 2x^{16}) \\
& + q^{87} x^{27} (1 - x^2 + x^4 - 3x^5 + 4x^6 + 2x^7 - x^8 - 4x^9 + 3x^{10} + 3x^{11} - 3x^{12} - 3x^{13} + 3x^{14} + x^{15} + 2x^{16}) \\
& + q^{71} x^{21} (1 + x - x^3 + x^4 + 2x^5 - x^6 + x^8 - x^9 + 3x^{10} + 3x^{11} + 6x^{12} + 4x^{13} + 2x^{14} - x^{16} - 3x^{17}) \\
& + q^{91} x^{27} (1 - 2x^3 - 3x^4 + x^5 - x^6 - x^8 + x^9 - 5x^{10} + 8x^{11} - 2x^{13} - 4x^{14} - 2x^{15} - 2x^{16} + x^{17}) \\
& + q^{85} x^{26} (1 - x + x^2 + 2x^3 - 3x^4 + 3x^6 + 4x^7 - 2x^8 - 2x^9 - x^{10} + 2x^{11} - 2x^{12} + 2x^{13} + x^{14} + 4x^{16} + x^{17}) \\
& + q^{70} x^{20} (-1 + 2x^2 - 3x^4 + 2x^5 + 2x^6 + x^7 + x^8 - x^9 + 2x^{10} - 4x^{11} + 7x^{13} - 4x^{14} + 6x^{15} - 2x^{16} + 2x^{17}) \\
& + q^{84} x^{24} (-1 + x^3 - x^4 - 2x^5 - 2x^7 - 3x^8 - 6x^9 + 9x^{10} - 9x^{12} + 7x^{13} + x^{14} + 6x^{16} + 3x^{17}) \\
& + q^{68} x^{19} (-1 + x^2 - x^5 - 2x^6 - 2x^9 + x^{10} - 2x^{11} - 5x^{12} - 3x^{13} + 6x^{15} + x^{16} + x^{17} - x^{18}) \\
& - q^{86} x^{25} (1 - 3x^2 + x^5 + 3x^6 - x^7 + x^8 + x^9 + x^{10} - 3x^{11} - 5x^{13} + 3x^{14} - 3x^{15} - 5x^{16} - 4x^{17} + x^{18}) \\
& + q^{82} x^{24} (-1 + 2x^4 + 3x^5 - 4x^6 - 5x^7 - 3x^8 + 5x^9 - 7x^{10} - 3x^{11} + x^{12} + x^{14} - x^{15} - 2x^{16} + 3x^{17} + x^{18}) \\
& + q^{81} x^{22} (1 + x^5 + x^6 - x^7 + x^8 + 3x^9 - 2x^{10} + 4x^{11} - 4x^{13} - 9x^{14} - x^{15} - 4x^{16} + x^{17} - 2x^{18} + x^{19}) \\
& + q^{186} (x^{62} + 3x^{65}) + q^{199} (x^{64} + x^{67} - 3x^{68}) + q^{205} (x^{65} - 2x^{68}) \\
& + q^{217} (x^{71} - x^{73})]
\end{aligned}$$

$$\begin{aligned}
h_3 = & q^{327} x^{15} [-1 + (1 + q + q^2 + q^3 + q^4 + q^5 + q^6) x \\
& - q (1 + q + 2q^2 + 2q^3 + 3q^4 + 3q^5 + 3q^6 + 2q^7 + 2q^8 + q^9 + q^{10}) x^2 \\
& + q^3 (1 + q + 2q^2 + 3q^3 + 4q^4 + 4q^5 + 5q^6 + 4q^7 + 4q^8 + 3q^9 + 2q^{10} + q^{11} + q^{12}) x^3 \\
& - q^6 (1 + q + 2q^2 + 3q^3 + 4q^4 + 4q^5 + 5q^6 + 4q^7 + 4q^8 + 3q^9 + 2q^{10} + q^{11} + q^{12}) x^4 \\
& + q^{10} (1 + q + 2q^2 + 2q^3 + 3q^4 + 3q^5 + 3q^6 + 2q^7 + 2q^8 + q^9 + q^{10}) x^5 \\
& - q^{15} (1 + q + q^2 + q^3 + q^4 + q^5 + q^6) x^6 + q^{21} x^7]^2 \times \\
& [1 - qx^2 - 2q^2x^3 - q^{183}x^{59} - q^{179}x^{60} + q^{184}x^{61} + q^{196}x^{62} + q^{189}x^{63} - q^{191}x^{64} \\
& - q^{197}x^{64} - q^{190}x^{65} - q^{192}x^{65} - q^{198}x^{65} + q^{201}x^{67} + q^7x^6 (2 + x - 2x^2) \\
& - q^{188}x^{62} (-2 + x^2) + q^{178}x^{59} (-1 - x + x^2) + q^4x^4 (1 - x + x^2) \\
& + q^3x^2 (-1 + x^3) + q^{186}x^{59} (-1 + x^3) + q^{187}x^{60} (-1 + x + x^3) \\
& + q^{168}x^{54} (-1 + x^2 - 2x^4) + q^5x^3 (-1 + 3x^2 + x^4) + q^{181}x^{59} (1 + 2x^2 + x^3 + x^4) \\
& - q^{173}x^{56} (-2 + x^2 + 2x^3 + 3x^4) + q^{171}x^{55} (1 + x + 3x^2 - 4x^3 - 2x^5) \\
& + q^{180}x^{57} (-1 - x - 2x^2 + x^5) + q^{177}x^{57} (1 - 2x^3 + x^5) - q^{175}x^{57} (-1 + 2x^2 - 2x^4 + x^5) \\
& - q^{170}x^{55} (-1 - 2x + x^2 + x^4 + x^5) - q^{11}x^5 (-3 + x^2 + x^3 + x^5 + x^6) + q^{21}x^9 (-2 + x + x^2 - x^3 - 2x^7) \\
& + q^{10}x^4 (1 + x + 2x^2 - x^4 - x^7) - q^{24}x^9 (4 + x - 5x^2 + 2x^5 + x^7) + q^{13}x^6 (1 + x - 4x^2 - x^5 + 2x^7) \\
& + q^{176}x^{55} (1 + x^2 + x^3 - x^4 + x^5 + 3x^7) + q^9x^2 (-1 + x^3 + x^6 - x^7 - 3x^8) \\
& + q^{154}x^{46} (-1 + 2x^2 + x^3 + x^4 + x^5 - 2x^6 - x^8) + q^{169}x^{53} (-1 + x^2 + 2x^3 + x^8) \\
& + q^{166}x^{52} (-1 - x - x^2 - x^3 - 2x^5 - 4x^7 + x^8) + q^6 (x^5 - x^7 + x^8) \\
& - q^{158}x^{49} (-1 + 2x - 2x^2 + x^4 - 5x^6 + x^7 + x^8) - q^{160}x^{51} (-1 + 3x + 2x^2 + 3x^3 + x^4 - 2x^5 + 2x^6 + 2x^8) \\
& + q^{12}x^4 (1 - 2x^3 - x^4 - x^5 + x^7 + 2x^8) + q^{17}x^5 (2 + x^2 - x^3 + x^4 - x^5 - x^6 + 2x^7 + 2x^8) \\
& + q^{16}x^6 (2 - x^3 + 3x^4 + x^5 + x^6 + x^7 - x^9) + q^{18}x^7 (-2 - 2x^2 + 2x^4 + 3x^5 + 2x^6 + x^7 - x^9) \\
& + q^{20}x^7 (-1 - 2x + x^2 + x^3 + x^4 + 2x^5 - 2x^7 - 2x^8 - x^9) \\
& + q^{167}x^{51} (-1 - x^2 + x^3 + 2x^4 + 3x^5 + x^6 + x^7 - 2x^8 - x^9) \\
& + q^{174}x^{53} (1 - x^4 - 2x^5 + x^9) - q^8 (x^3 + x^7 + x^9) + q^{15}x^5 (1 - 3x^4 - x^5 + 2x^6 + x^7 + x^9) \\
& - q^{31}x^{12} (1 + x - 3x^2 + 2x^3 + 2x^4 + x^5 - 5x^6 - 3x^8 + x^9) \\
& - q^{19}x^6 (-1 + x + 4x^2 + 2x^4 + x^6 - 2x^7 - 2x^8 + 2x^9) \\
& - q^{143}x^{44} (2 + 2x + 3x^2 - 2x^4 + x^5 - 4x^6 + 5x^7 - 2x^8 + 4x^9) \\
& + q^{22}x^6 (1 - 2x^2 + 4x^4 + 3x^5 + 2x^6 + 2x^7 - x^9 - 4x^{10}) \\
& + q^{155}x^{48} (1 + x^2 + 2x^3 - 2x^4 - 2x^5 - 3x^6 + 4x^7 + x^8 - x^{10}) \\
& - q^{161}x^{48} (-1 + x^4 + x^5 + x^6 - 3x^7 + x^8 - x^9 + x^{10}) \\
& + q^{164}x^{50} (-1 - x^3 + 2x^4 + 3x^5 + 2x^7 + x^8 - x^9 + x^{10}) \\
& + q^{14}x^3 (-1 - 3x^4 - 2x^5 - x^6 + 2x^{10}) \\
& - q^{138}x^{42} (-2 - 2x - 2x^2 + 5x^3 + 6x^5 + x^6 - 5x^7 + 3x^8 - 3x^9 + 3x^{10}) \\
& + q^{23}x^7 (1 - x + 2x^3 - x^4 + 3x^5 + x^7 - 3x^{10} + x^{11})
\end{aligned}$$

$$\begin{aligned}
& -q^{163}x^{48}(-1+2x^4+x^5-x^7-3x^8-4x^9+x^{10}+x^{11}) \\
& +q^{151}x^{45}(-1+2x^2+2x^3+2x^5-3x^6-5x^7-4x^8+2x^{10}+x^{11}) \\
& +q^{147}x^{45}(-3-2x-2x^2-x^3+6x^4+x^5-x^6-3x^7-2x^8+3x^{10}+x^{11}) \\
& +q^{120}x^{37}(1-x-4x^2-2x^3-x^4-2x^5+x^6+x^7-8x^8-6x^9+5x^{10}+x^{11}) \\
& +q^{153}x^{45}(-1+2x^4+2x^5-x^7-4x^8+2x^9+2x^{11}) \\
& +q^{25}x^5(1-x^3-2x^5+2x^6-x^8+x^9-2x^{10}+2x^{11}) \\
& +q^{140}x^{43}(3-x-2x^2-3x^3-7x^4-x^5+x^6+3x^7-x^8+x^{10}+2x^{11}) \\
& +q^{172}x^{50}(-1+x^4-4x^9+x^{10}+2x^{11}) \\
& +q^{149}x^{44}(-2-2x+3x^4+4x^6+2x^7-2x^8-3x^9+4x^{10}+2x^{11}) \\
& -q^{150}x^{46}(1-x^2-3x^3-2x^4-3x^5+2x^6+2x^7+x^9-2x^{10}+3x^{11}) \\
& +q^{110}x^{33}(-2-5x+3x^2+2x^3+3x^4+4x^5-x^6+x^7+8x^9+x^{10}-7x^{11}-3x^{12}) \\
& +q^{130}x^{40}(-2+3x+6x^2+3x^3+6x^4-2x^5-3x^6-2x^7+3x^8+2x^9-x^{10}+2x^{11}-2x^{12}) \\
& -q^{32}x^{11}(-3-3x+3x^2+3x^3-2x^4+5x^5+4x^6+2x^7-4x^8-3x^{10}+x^{12}) \\
& +q^{29}x^9(1-x+5x^3-2x^5+x^7-x^8+3x^9-x^{10}+x^{12}) \\
& +q^{162}x^{47}(1-2x^7+3x^9+x^{10}-3x^{11}+x^{12}) \\
& +q^{159}x^{47}(1+x-x^4-2x^6+5x^9-x^{11}+x^{12}) \\
& +q^{134}x^{39}(-2-x+2x^3+3x^4-x^6-6x^7-3x^8-x^9+5x^{10}-x^{11}+x^{12}) \\
& -q^{152}x^{45}(2+x+x^3-x^4-4x^5-x^6-x^7+2x^8-3x^{10}+x^{11}+x^{12}) \\
& -q^{156}x^{46}(1-2x-x^3-3x^4+x^6+2x^7-2x^8+x^9-x^{10}+x^{11}+x^{12}) \\
& -q^{165}x^{48}(-1+x^3+2x^5+x^6+x^8+x^9+2x^{10}+x^{11}+x^{12}) \\
& -q^{133}x^{40}(2-5x-x^3-2x^4+x^5+x^6+2x^7-3x^8-3x^{10}+6x^{11}+x^{12}) \\
& +q^{27}x^8(-2-2x+3x^3-x^4-3x^7-x^8-x^9+2x^{12}) \\
& +q^{43}x^{13}(-1-2x-2x^2+2x^3+5x^4+4x^5+3x^6+3x^7-3x^8-5x^{10}-x^{11}+2x^{12}) \\
& +q^{136}x^{42}(6+2x+2x^2+2x^3-3x^4-8x^5+2x^6+4x^7+3x^8-2x^9-2x^{10}+2x^{11}+2x^{12}) \\
& +q^{26}x^7(-1-x^2+x^3-x^4+4x^5+4x^6-4x^7-4x^8-4x^9-2x^{10}+3x^{12}) \\
& +q^{117}x^{36}(3+4x-5x^4-5x^5-4x^6-x^8-6x^9+2x^{10}+x^{11}+3x^{12}) \\
& +q^{157}x^{45}(-1+x^5-x^6-2x^7-4x^8+2x^9+3x^{10}+3x^{11}+3x^{12}) \\
& +q^{119}x^{36}(3+4x+x^2-2x^3-5x^4-4x^5-3x^6+4x^7+2x^8-3x^9+6x^{10}-x^{11}+4x^{12}) \\
& +q^{36}x^{10}(1+x-4x^4-3x^5-4x^6-2x^8+7x^9+x^{10}+2x^{11}-2x^{12}-3x^{13}) \\
& +q^{131}x^{39}(-2-2x-2x^2+2x^3+6x^4+4x^5+7x^6-4x^7+x^8+2x^9+2x^{10}-4x^{11}-4x^{12}-2x^{13}) \\
& +q^{34}x^{10}(1+2x+x^2+2x^3-4x^4-5x^5-x^6+3x^7+3x^9+x^{10}+x^{11}-3x^{12}-x^{13}) \\
& +q^{41}x^{12}(1+2x-x^2+x^3+2x^4+3x^5+5x^6+3x^8-x^9-3x^{10}-4x^{11}+x^{12}-x^{13}) \\
& +q^{145}x^{43}(1+x-x^2+x^4-4x^5+2x^7-3x^8-5x^9+3x^{10}+2x^{11}+x^{12}-x^{13}) \\
& +q^{144}x^{42}(2-x^2-2x^3-2x^4-x^6+2x^7+4x^8+3x^9-x^{10}+x^{13}) \\
& -q^{128}x^{37}(-1+6x^2+x^3-x^4-5x^5-3x^7+3x^8+5x^9-3x^{12}+x^{13})
\end{aligned}$$

$$\begin{aligned}
& + q^{37}x^{12}(-1 - 3x - 3x^3 + x^4 + 3x^5 + 2x^6 - x^7 + 5x^8 - 2x^9 + x^{10} - x^{11} - 3x^{12} + x^{13}) \\
& - q^{146}x^{43}(-1 + 2x + x^2 + x^3 + 2x^4 + x^5 - x^6 - 4x^7 - 2x^8 + 3x^9 + 2x^{10} - 2x^{12} + x^{13}) \\
& + q^{28}x^7(-1 + x + 3x^4 + 3x^5 + 3x^7 - x^8 - 6x^9 + 3x^{10} - 2x^{11} + x^{12} + x^{13}) \\
& - q^{148}x^{43}(-1 + x^2 + x^3 - x^6 - 2x^7 - 2x^8 + 3x^9 - 3x^{10} + x^{11} + x^{12} + x^{13}) \\
& - q^{125}x^{38}(-1 + 4x + x^2 - x^3 + 5x^4 - 6x^6 - 2x^7 + 5x^8 - 2x^9 - 4x^{10} + 2x^{11} + 2x^{12} + x^{13}) \\
& - q^{51}x^{17}(-2 - 2x + x^2 + 6x^3 + 4x^4 + 8x^5 + 2x^6 - 6x^7 - 3x^8 - 5x^{10} + x^{11} - 3x^{12} + 2x^{13}) \\
& + q^{142}x^{41}(1 + 2x + x^2 - x^4 - 2x^5 - 3x^6 - 4x^7 + 3x^8 + 5x^9 + x^{10} - 2x^{11} + x^{12} + 2x^{13}) \\
& + q^{141}x^{42}(3 + 2x - x^2 + 2x^3 + x^4 - 5x^5 + 7x^7 - 4x^9 - 3x^{10} - 2x^{11} + 2x^{12} + 2x^{13}) \\
& - q^{35}x^{10}(-1 - 2x - 3x^2 + 2x^4 + 3x^5 + x^6 + x^7 - 3x^8 - x^9 + 4x^{13}) \\
& + q^{49}x^{13}(1 - x - 3x^2 + x^3 + 2x^4 + 3x^5 + 2x^6 - 2x^7 - 2x^8 - 3x^9 - 4x^{10} - 2x^{11} + x^{12} + 4x^{13}) \\
& + q^{118}x^{34}(-1 - x + 5x^2 + 2x^3 - 2x^4 + x^5 - 3x^6 - x^7 - x^8 + 8x^9 + x^{10} - 3x^{11} - 3x^{12} + 5x^{13}) \\
& + q^{135}x^{39}(-1 + x^3 + x^4 - 4x^5 + x^6 + x^7 - x^8 + x^9 + 2x^{10} - 3x^{12} + x^{14}) \\
& - q^{30}x^8(1 - 3x^2 + x^3 - 2x^5 + 2x^6 + 3x^7 + 3x^8 + x^9 - 3x^{11} - x^{12} + x^{14}) \\
& + q^{39}x^{10}(-1 - 2x^3 - 2x^4 - 2x^5 + 3x^6 - 3x^7 + 5x^8 + 5x^{10} - 3x^{11} + 2x^{12} - x^{13} + x^{14}) \\
& + q^{46}x^{14}(-1 - 2x - 3x^2 + 2x^3 + 2x^4 + 3x^5 - x^6 - x^7 - x^8 + x^9 - 7x^{10} - x^{11} + 2x^{12} - x^{13} + x^{14}) \\
& - q^{33}x^8(1 + x + x^2 - x^3 - 2x^5 + 2x^6 + x^7 - 3x^8 + 3x^9 - x^{11} - 4x^{12} + x^{13} + x^{14}) \\
& - q^{100}x^{30}(-6 - 8x + 4x^2 + 3x^3 + 8x^4 + 3x^5 + 10x^7 + 4x^9 - 2x^{11} - x^{12} + x^{13} + x^{14}) \\
& + q^{38}x^{11}(2 + 2x - x^2 - 2x^3 - 2x^4 - 5x^5 + 2x^6 + 2x^7 + 4x^8 - x^9 + 4x^{10} - x^{11} + x^{12} + 2x^{14}) \\
& + q^{137}x^{40}(-2 - x + 4x^2 - x^3 + x^4 + 4x^5 - 7x^6 + x^7 + x^8 + x^9 + 2x^{10} - 5x^{11} - 4x^{12} - 2x^{13} + 2x^{14}) \\
& + q^{42}x^{12}(1 - x - 2x^2 - x^3 - x^4 + 2x^6 + 6x^7 + 2x^8 + 2x^9 - 5x^{10} - 2x^{11} - x^{13} + 2x^{14}) \\
& - q^{126}x^{37}(-1 + x + 6x^2 + x^3 - x^4 - 5x^5 - x^6 - 6x^7 + 4x^8 + 4x^9 + 6x^{10} + x^{13} + 2x^{14}) \\
& + q^{44}x^{13}(1 - x - 2x^2 + 2x^3 + 4x^4 + x^5 + 2x^6 + 2x^7 + 6x^8 - 3x^9 - 2x^{10} - 2x^{11} + 5x^{12} + 4x^{13} + 2x^{14}) \\
& + q^{40}x^{12}(1 - 4x^2 - 5x^3 - 3x^4 + x^5 + 5x^7 + 2x^8 + 2x^9 - 6x^{10} - 2x^{11} - 4x^{12} + 3x^{14}) \\
& + q^{66}x^{20}(-2 + x + x^2 - 4x^5 - 4x^6 - 13x^7 - 2x^8 - 4x^9 + 3x^{11} + 7x^{12} - x^{13} + 4x^{14}) \\
& + q^{48}x^{14}(-2 + x^3 + 7x^4 + x^5 - 2x^6 - x^7 - 6x^8 - 2x^9 - 4x^{10} + 3x^{11} + 3x^{13} + 2x^{14} - 3x^{15}) \\
& + q^{122}x^{35}(1 - x^3 + x^4 + x^5 - 5x^6 + 3x^7 - 2x^8 + 6x^9 - x^{10} - 9x^{11} + 3x^{12} + x^{13} + 3x^{14} - 3x^{15}) \\
& + q^{50}x^{14}(-1 - x + 2x^2 + 4x^3 - x^4 + x^5 + x^6 - 5x^7 - 3x^8 + 4x^9 + x^{10} + 4x^{12} + 5x^{13} + 4x^{14} - x^{15}) \\
& - q^{123}x^{36}(-4 - 2x + x^2 + 2x^3 + 6x^4 + 5x^5 + 2x^6 - 2x^8 + x^{10} - 2x^{11} - 7x^{12} + x^{15}) \\
& + q^{104}x^{31}(3 + 2x - 2x^2 - x^3 - 3x^4 - 5x^5 - 4x^6 + 3x^9 - 4x^{13} + x^{15}) \\
& + q^{139}x^{39}(-1 + x^2 + 2x^4 + 2x^5 - 3x^6 - 2x^8 - 3x^9 + 2x^{10} + x^{11} - x^{12} - x^{13} + x^{15}) \\
& + q^{56}x^{17}(1 + 2x^2 + x^3 - 4x^4 + 2x^5 + 2x^6 + 3x^7 + 2x^8 + 9x^9 + 2x^{10} + x^{11} - 2x^{12} - 4x^{14} + x^{15}) \\
& + q^{53}x^{16}(2 + 4x + x^2 - x^3 - 3x^4 - 5x^5 - x^6 + 2x^7 + x^8 + 6x^{10} - x^{11} - 4x^{12} - x^{14} + x^{15}) \\
& + q^{116}x^{34}(-5 + 3x - 2x^2 + 6x^3 - x^4 + 3x^5 + 5x^6 - 3x^7 + x^8 + 4x^9 + 2x^{10} - 6x^{11} - x^{12} - x^{14} + x^{15}) \\
& + q^{109}x^{32}(-1 - x - 2x^2 - 4x^3 + 4x^6 + 3x^7 + x^8 - 3x^9 + 2x^{10} + 2x^{11} + x^{12} - 6x^{13} + x^{14} + x^{15}) \\
& - q^{129}x^{36}(-1 - x + x^3 + 3x^4 + 2x^5 - 3x^7 - 6x^9 + x^{10} + 2x^{11} - 6x^{12} + 2x^{13} + x^{14} + x^{15})
\end{aligned}$$

$$\begin{aligned}
& + q^{115} x^{33} (-1 - 2x^2 + 8x^3 + 3x^4 + x^5 - 5x^6 - 4x^7 - 4x^8 - 2x^9 + 5x^{10} - 6x^{11} - x^{12} + 2x^{13} + x^{14} + x^{15}) \\
& + q^{96} x^{28} (-1 - x + 4x^2 + x^3 + 8x^4 + 5x^6 - x^7 - 2x^8 + 2x^9 - 3x^{10} - x^{11} + 6x^{12} + 2x^{14} + x^{15}) \\
& - q^{58} x^{17} (-1 + 4x^2 + 2x^3 + x^4 - 2x^5 - 2x^6 - 5x^7 - 2x^8 + 3x^9 - x^{10} - 2x^{11} + 5x^{12} + 7x^{13} + 6x^{14} + x^{15}) \\
& - q^{45} x^{13} (1 + x^2 - 3x^3 - 4x^4 - 5x^5 + 2x^6 + 6x^7 + 6x^8 + 5x^{10} - x^{11} - 2x^{12} - 3x^{14} + 2x^{15}) \\
& - q^{103} x^{30} (-1 - 5x + 5x^2 + 5x^3 + 3x^4 + 3x^5 + 5x^6 - 3x^7 - 2x^8 + x^9 + 4x^{10} + 3x^{11} - 7x^{12} + 7x^{13} + 2x^{14} \\
& + 3x^{15}) \\
& - q^{54} x^{16} (1 - 2x - 6x^2 + x^4 + x^5 + x^7 - 4x^9 - x^{10} - 7x^{11} - 2x^{12} + 5x^{13} + 4x^{15}) \\
& - q^{69} x^{21} (2 + 5x - 4x^2 - x^3 + 2x^4 + 6x^5 + 3x^6 + 5x^7 + 3x^8 - 8x^9 - 6x^{11} - 3x^{12} + x^{13} - 3x^{14} + 4x^{15}) \\
& + q^{61} x^{18} (1 - 3x^2 - 3x^3 - 2x^4 + 4x^5 + 8x^6 + 9x^7 + x^8 - 2x^{10} - 4x^{11} - 2x^{12} + 2x^{13} - 3x^{14} + 4x^{15}) \\
& - q^{71} x^{21} (1 + 2x - 3x^4 + 3x^5 - x^6 + 2x^{11} + x^{12} - 5x^{13} - 2x^{14} + 4x^{15}) \\
& + q^{64} x^{19} (2 + x - x^3 + 4x^4 + 8x^5 - 2x^6 - 3x^7 - 4x^8 - 6x^9 - 2x^{10} - 4x^{12} - x^{13} - 2x^{14} + 4x^{15}) \\
& + q^{124} x^{34} (-1 + x^3 - x^4 - 4x^5 - 2x^6 + x^7 - x^8 + 5x^9 + 4x^{10} + x^{11} - 2x^{12} + 3x^{13} - x^{14} + 5x^{15}) \\
& + q^{90} x^{25} (3 - 3x^2 - 2x^3 + 2x^5 + 8x^6 + 3x^8 + 5x^9 - 6x^{10} + 2x^{11} + 8x^{12} + x^{14} + 5x^{15}) \\
& + q^{105} x^{29} (-1 + x + x^3 - 6x^4 - 5x^5 + 8x^6 + 8x^7 + x^9 + 5x^{10} - 13x^{11} - 6x^{12} + 4x^{13} - 4x^{14} - 2x^{15} - 2x^{16}) \\
& + q^{99} x^{29} (-1 + x + x^2 + 3x^3 + x^4 + 4x^7 - 2x^8 - x^9 - 2x^{10} - 5x^{11} + x^{12} + 3x^{13} - 3x^{15} - x^{16}) \\
& + q^{63} x^{18} (1 + x + 6x^5 + x^6 + 3x^7 + 4x^8 - 3x^9 - x^{10} + 5x^{12} - 3x^{13} + 3x^{14} + 4x^{15} - x^{16}) \\
& - q^{47} x^{12} (-1 + x^2 - x^4 - 4x^5 - x^6 + x^7 + 9x^9 + 6x^{10} + 7x^{11} + 6x^{13} - 3x^{14} + x^{16}) \\
& + q^{132} x^{37} (1 - x - 3x^3 - 2x^5 + x^6 + 4x^7 - 3x^9 - 6x^{10} - 2x^{11} + 5x^{12} - 3x^{13} - x^{14} + x^{16}) \\
& - q^{92} x^{26} (1 + 2x + 4x^2 - x^3 - x^4 - 3x^5 - x^6 + 5x^8 + 2x^9 - 5x^{10} + 5x^{12} + 6x^{13} + x^{14} - 3x^{15} + x^{16}) \\
& + q^{101} x^{28} (-2 - 2x^3 + 3x^4 - x^5 - 3x^6 + x^7 - 2x^8 + 7x^9 + 5x^{10} - 6x^{11} - 3x^{12} + 9x^{13} - 2x^{15} + x^{16}) \\
& - q^{67} x^{19} (-2 + 2x^2 - 2x^3 - 6x^4 - 5x^5 + x^6 + 4x^7 + x^8 + 4x^9 - x^{11} - 5x^{12} + 2x^{13} - 9x^{14} + 2x^{15} + x^{16}) \\
& - q^{127} x^{36} (-1 + 3x^4 + x^5 + x^6 - 3x^7 - 4x^8 - 2x^9 + x^{11} - 5x^{12} - 3x^{14} + 4x^{15} + x^{16}) \\
& + q^{59} x^{17} (-2 + x - x^2 - 7x^3 - 6x^4 - 3x^5 + 6x^6 + 4x^7 + 8x^8 - 7x^{10} - 6x^{11} + x^{12} - 7x^{13} + 2x^{16}) \\
& - q^{121} x^{33} (1 + x^2 - x^3 - 6x^4 - x^5 + 5x^6 + 4x^8 + 8x^9 - 8x^{10} - 2x^{11} + x^{12} + x^{13} - 2x^{14} - 3x^{15} + 2x^{16}) \\
& + q^{70} x^{20} (2 - 3x^2 + 2x^3 + 3x^4 - 8x^5 - 4x^6 + x^7 - x^8 + 9x^{10} + 3x^{11} - x^{12} + 9x^{14} - 3x^{15} + 2x^{16}) \\
& + q^{55} x^{15} (-1 + x + x^2 + x^3 - 4x^4 - 8x^5 - 3x^6 + x^7 + x^8 + 4x^9 + 8x^{10} + 2x^{11} + 5x^{13} - 2x^{14} - x^{15} + 2x^{16}) \\
& - q^{82} x^{22} (1 - x - 2x^2 + x^4 + 5x^6 - 4x^7 - 3x^8 - 5x^{10} + 3x^{11} + 5x^{12} - 5x^{14} + 2x^{15} + 2x^{16}) \\
& - q^{52} x^{14} (1 + 2x + x^2 - 2x^3 + 3x^5 + 2x^6 + x^8 + 6x^9 - 2x^{10} - 7x^{11} - x^{12} + x^{13} + x^{14} + 3x^{15} + 2x^{16}) \\
& + q^{87} x^{25} (2 - x^2 - 4x^3 + 3x^4 - 2x^5 - 7x^6 - x^7 + 5x^8 - 6x^9 - 4x^{10} + 15x^{11} + 2x^{13} + 2x^{14} + 3x^{15} + 2x^{16}) \\
& + q^{113} x^{32} (1 - 5x - 2x^2 + 2x^3 + 8x^4 + x^5 - 2x^6 + 2x^7 - x^8 - 4x^9 - 2x^{10} + 3x^{11} + 4x^{12} - 3x^{13} \\
& + 4x^{14} + 3x^{16}) \\
& + q^{112} x^{31} (1 - x - x^3 - 5x^4 + 4x^5 - x^6 - 4x^7 + 3x^8 + 5x^9 - 4x^{10} + 9x^{11} + 4x^{12} - 4x^{13} - 2x^{15} + 3x^{16}) \\
& + q^{107} x^{30} (1 + 3x^2 - 5x^3 - 2x^4 + x^5 + 3x^6 + 7x^7 + 2x^8 + 2x^9 - 3x^{10} + 3x^{11} + 2x^{12} + x^{13} - 2x^{14} \\
& - x^{15} + 3x^{16}) \\
& + q^{114} x^{31} (1 - 3x^3 + x^4 + x^5 + x^6 + 3x^7 - 2x^8 - x^9 - 6x^{10} + 3x^{11} + 2x^{12} - 2x^{13} - 3x^{15} + 4x^{16})
\end{aligned}$$

$$\begin{aligned}
& -q^{86}x^{23}(2-4x^2+2x^3+x^4+2x^5+2x^6-7x^7+2x^8-x^9-9x^{10}+4x^{11}+2x^{12}+4x^{14}-x^{15}+4x^{16}) \\
& +q^{98}x^{27}(-2-2x+x^2+4x^3+8x^4+x^5-3x^6+6x^7-8x^8-4x^9+x^{10}-5x^{12}-7x^{13}+6x^{14}-6x^{15} \\
& +x^{16}-4x^{17}) \\
& +q^{94}x^{26}(1-2x+x^3+3x^4-3x^6+7x^7-5x^8-x^9-7x^{10}+2x^{11}-2x^{13}+4x^{15}+2x^{16}-3x^{17}) \\
& +q^{95}x^{27}(-1-6x-x^2+6x^3+2x^4-3x^5+6x^6+x^8+11x^{10}+x^{11}-8x^{12}+2x^{13}+4x^{14} \\
& +5x^{15}-x^{17}) \\
& -q^{93}x^{25}(-2+3x^2+6x^3+x^4-x^5-6x^6+x^7-5x^8-3x^9-8x^{11}+6x^{12}+4x^{13}+2x^{14} \\
& -7x^{15}+x^{17}) \\
& -q^{77}x^{21}(1+x+x^2-3x^3-5x^4+5x^5-5x^6+x^7-x^9-5x^{10}+2x^{11}+10x^{12}+4x^{13}+4x^{14} \\
& +2x^{15}+x^{17}) \\
& +q^{68}x^{19}(1-3x^2+4x^3+4x^4-3x^6-4x^7-3x^8-6x^9+x^{10}+3x^{11}-3x^{12}-4x^{13}+5x^{14} \\
& +6x^{15}+x^{17}) \\
& -q^{80}x^{22}(2+2x+x^2-2x^3-x^4+5x^5-2x^6-2x^7-7x^8-3x^{10}+3x^{11}+10x^{12}+2x^{13}-x^{14} \\
& +7x^{15}+x^{17}) \\
& -q^{60}x^{16}(1-2x^2+x^3+5x^4-x^5-6x^6-2x^7+3x^9+6x^{10}+5x^{11}+2x^{12}-2x^{13}+x^{14}+7x^{15} \\
& -3x^{16}+x^{17}) \\
& -q^{102}x^{28}(1-2x^2-3x^3-2x^4+5x^5-x^6+x^7+7x^8+x^9-3x^{10}+5x^{11}+3x^{12}-7x^{13}-3x^{14} \\
& -x^{15}+x^{16}+x^{17}) \\
& +q^{111}x^{30}(1-3x^3+2x^5+x^6+2x^7+6x^8+7x^9-8x^{10}-4x^{11}-3x^{12}-2x^{14}-5x^{15}+2x^{16}+x^{17}) \\
& +q^{108}x^{30}(1+4x-6x^4+3x^5+6x^6-2x^7+x^8+4x^9-3x^{10}+4x^{11}+2x^{12}+6x^{13}-5x^{14}+2x^{15} \\
& -x^{16}+2x^{17}) \\
& +q^{91}x^{24}(1+2x-2x^3-4x^4-2x^5-x^6-6x^7-3x^8-5x^9-5x^{10}+5x^{11}+4x^{12}+9x^{13}-2x^{14}+2x^{15} \\
& -x^{16}+2x^{17}) \\
& +q^{85}x^{24}(1+6x+3x^2-2x^3+x^4-4x^5-x^6-x^8-2x^9-3x^{10}+6x^{11}+3x^{12}-5x^{14}-x^{15}-x^{16}+3x^{17}) \\
& +q^{57}x^{14}(1+3x^3+3x^4-x^5-6x^6-3x^7-4x^8+x^9+2x^{10}+2x^{11}+7x^{12}+6x^{13}+x^{14}-3x^{15}-6x^{16} \\
& +4x^{17}) \\
& +q^{75}x^{20}(2-x-2x^2+2x^3+x^4+5x^5-x^6-x^7+4x^8+3x^9+2x^{10}+2x^{11}+5x^{12}+3x^{13}+7x^{15}-7x^{16} \\
& -3x^{18}) \\
& +q^{72}x^{19}(1-2x^2+2x^3-4x^4+3x^5-2x^6-5x^7-8x^8+5x^9-x^{10}-6x^{11}+15x^{12}+3x^{13}+3x^{15}+3x^{16} \\
& +4x^{17}-2x^{18}) \\
& +q^{97}x^{26}(1-x^3+2x^4+4x^5-3x^6-8x^7+7x^8+4x^9+7x^{11}-6x^{13}+x^{14}+x^{15}-x^{16}-4x^{17}-x^{18}) \\
& +q^{76}x^{19}(1-x^3+2x^4+x^5-x^6-4x^7-4x^8+3x^9+2x^{10}+7x^{11}+4x^{12}+6x^{13}+2x^{14}-3x^{15}-2x^{16} \\
& +2x^{17}-x^{18}) \\
& -q^{74}x^{19}(-1+2x^3-x^4-6x^5+5x^6+4x^7+x^8-2x^9-5x^{10}-11x^{11}-x^{12}+4x^{13}+4x^{14}+x^{15}+x^{18}) \\
& +q^{65}x^{17}(-1+x-x^2-2x^3-3x^4-x^5+3x^6-2x^7+x^8+3x^{10}-5x^{11}-5x^{12}-4x^{13}+x^{14}+6x^{16}+x^{18})
\end{aligned}$$

$$\begin{aligned}
& + q^{79} x^{21} (-1 - x + 2x^3 + 6x^4 + x^5 - 3x^6 + 3x^7 + 7x^8 - 10x^9 - 7x^{10} + x^{11} - 5x^{12} + 2x^{13} - x^{14} - 4x^{15} \\
& - 7x^{16} - 3x^{17} + x^{18}) \\
& - q^{106} x^{28} (1 - x^3 + 2x^4 + 2x^5 + 5x^6 + 3x^7 + 6x^8 + x^9 - 7x^{10} - 2x^{11} + x^{12} - x^{13} - 8x^{14} + 2x^{15} + 5x^{16} \\
& - x^{17} + x^{18}) \\
& + q^{62} x^{16} (-1 + 3x^3 - 7x^5 + 7x^6 + 6x^7 + 4x^8 - 2x^9 + 3x^{10} - 3x^{11} - 8x^{12} - x^{13} - 3x^{14} - 2x^{15} + 2x^{16} + 2x^{18}) \\
& + q^{83} x^{22} (-2 - 2x + 3x^2 + 2x^3 + x^4 + x^5 + 3x^6 + 4x^7 - 4x^8 - 4x^9 - 2x^{10} - 4x^{11} - 3x^{12} - 4x^{13} - 3x^{14} \\
& - 3x^{15} - 2x^{16} + 4x^{17} + 2x^{18}) \\
& + q^{89} x^{24} (1 - x^3 + x^4 - x^5 + 3x^6 - 5x^7 - 8x^8 - 5x^9 + 9x^{10} + 3x^{11} + x^{12} + 3x^{13} - x^{14} + x^{15} + 5x^{16} \\
& + 4x^{17} + 2x^{18}) \\
& + q^{84} x^{22} (-1 + 2x^2 + x^3 - 2x^4 - 6x^5 + 6x^7 + 4x^9 - 6x^{11} - 4x^{12} + 5x^{13} + 5x^{15} - 3x^{16} - x^{17} + 3x^{18}) \\
& + q^{81} x^{20} (1 - x - x^3 + 2x^4 - 2x^5 + x^6 - 2x^7 - 2x^8 + x^9 - x^{10} - 2x^{11} - 6x^{12} - 4x^{13} - 6x^{14} + 3x^{15} + 3x^{16} \\
& - x^{17} - 5x^{18} + 2x^{19}) \\
& + q^{78} x^{19} (1 + x - 3x^3 - x^4 + x^5 - 5x^7 - 5x^8 + 7x^9 + x^{10} - 2x^{11} + 8x^{12} - 4x^{13} - 6x^{14} + 3x^{15} + 6x^{16} \\
& - 3x^{17} - 6x^{18} + 3x^{19} - 2x^{20}) \\
& + q^{88} x^{22} (-1 + x^2 + 5x^4 - 3x^5 - 5x^6 + x^7 - 5x^9 + 4x^{10} - 5x^{11} - 2x^{12} + x^{13} + 7x^{14} + x^{15} - 4x^{16} \\
& + 5x^{17} + x^{20}) \\
& - q^{73} x^{17} (1 + x^4 + x^5 - 2x^6 - 3x^7 + x^8 + x^9 - 5x^{10} - 2x^{11} - 2x^{13} - 7x^{14} + 3x^{16} + x^{18} + 6x^{19} + 2x^{20}) \\
& + q^{182} (x^{60} + 3x^{62}) - q^{185} (x^{60} + 2x^{64})]
\end{aligned}$$

$$\begin{aligned}
h_4 = & -q^{343} x^{18} [-1 + (1 + q + q^2 + q^3 + q^4 + q^5 + q^6) x \\
& - q (1 + q + 2q^2 + 2q^3 + 3q^4 + 3q^5 + 3q^6 + 2q^7 + 2q^8 + q^9 + q^{10}) x^2 \\
& + q^3 (1 + q + 2q^2 + 3q^3 + 4q^4 + 4q^5 + 5q^6 + 4q^7 + 4q^8 + 3q^9 + 2q^{10} + q^{11} + q^{12}) x^3 \\
& - q^6 (1 + q + 2q^2 + 3q^3 + 4q^4 + 4q^5 + 5q^6 + 4q^7 + 4q^8 + 3q^9 + 2q^{10} + q^{11} + q^{12}) x^4 \\
& + q^{10} (1 + q + 2q^2 + 2q^3 + 3q^4 + 3q^5 + 3q^6 + 2q^7 + 2q^8 + q^9 + q^{10}) x^5 \\
& - q^{15} (1 + q + q^2 + q^3 + q^4 + q^5 + q^6) x^6 + q^{21} x^7]^2 \times \\
& [-1 + qx^2 + q^2 x^3 + q^{11} x^3 - q^3 x^5 + q^4 x^5 + 2q^{191} x^{65} - 2q^{207} x^{68} - q^{217} x^{68} + q^{212} x^{70} \\
& + q^{210} (-1 + x) x^{70} + q^{205} x^{71} + q^{220} x^{71} + q^{221} x^{72} - q^{222} x^{73} - q^{225} x^{73} - q^{226} x^{74} \\
& + q^{229} x^{76} - q^6 x^4 (1 + x) + q^{204} x^{65} (1 + x) + q^{209} x^{69} (-1 + 2x) + q^{201} x^{63} (-1 + x^2) \\
& + q^{202} x^{65} (-1 + x^2)^2 (1 + x^2) + q^{197} x^{65} (-1 + x + x^2) \\
& + q^{219} x^{69} (-1 + 2x^2) - q^{208} x^{67} (-1 + x + 3x^2) + q^{211} x^{68} (-1 + 2x^3) \\
& + q^{195} x^{64} (1 + x + 2x^2 - x^3 - 2x^4) + q^{194} x^{62} (-1 + x + x^3 - 2x^4) \\
& + q^{213} x^{69} (-1 + x^2 + x^3 - x^4) + q^{215} x^{68} (-1 + x^4) + q^8 x^3 (1 - x + x^4) \\
& + q^{200} x^{66} (2 - x + x^4) + q^{206} x^{66} (2 - 2x^2 + x^4) \\
& - q^{199} x^{65} (-1 + x + x^2 - x^3 + x^4) - q^7 x^2 (-1 + x^3 + x^4) - q^{186} x^{62} (1 - x - x^2 + x^3 + x^4)
\end{aligned}$$

$$\begin{aligned}
& + q^{14}x^8(3+x^2-x^5) + q^{188}x^{61}(-2+x^3-x^5) + q^{17}x^7(2+2x+x^2+x^3-x^5) \\
& + q^{189}x^{62}(-1+x+x^2+x^3-x^4-x^5) + q^{13}x^6(-1+x+x^5) + q^9x^5(-1-x^2-x^3+x^5) \\
& + q^{159}x^{51}(1+2x-4x^3-2x^4+x^5) + q^{196}x^{63}(1+x^2+x^3-x^4+x^5) \\
& + q^{10}x^5(-1-x+x^4+x^5) - q^{185}x^{61}(1+x^4+2x^5) \\
& + q^{177}x^{58}(1+2x-x^2-x^3+x^4+x^5-x^6) + q^{198}x^{63}(-1+x-3x^3-2x^5+x^6) \\
& + q^{12}x^4(-1-2x+x^5+x^6) + q^{184}x^{59}(-1-x^2-2x^3+x^5+x^6) \\
& + q^{192}x^{63}(1-x^2+2x^3-x^4+x^5+x^6) - q^{193}x^{61}(1+x^2-x^3+x^4+2x^5+x^6) \\
& + q^{180}x^{57}(1-2x^4-2x^5+2x^6) + q^{160}x^{52}(1+x-2x^3-4x^4-3x^5+3x^6-2x^7) \\
& + q^5(x^2+x^3-x^7) + q^{203}x^{64}(-1+x^2-2x^4+x^5-x^7) \\
& + q^{18}x^8(1+x^3+x^4-2x^5-x^6-x^7) + q^{161}x^{54}(-1-2x+x^7) \\
& - q^{15}x^5(2+x^3-x^4+x^7) - q^{16}x^5(1+x-x^2+x^3-x^4-3x^5+x^7) \\
& + q^{175}x^{57}(1+2x-x^5+x^7) + q^{190}x^{61}(1-2x^2+x^3+2x^4-x^5+x^7) \\
& - q^{156}x^{52}(-1+x+3x^2+2x^3+x^5+x^7) + q^{173}x^{57}(1+3x^2-x^4+x^6+x^7) \\
& - q^{181}x^{59}(-1+x^2-2x^4-x^5+x^6+x^7) + q^{164}x^{54}(-3-x-2x^2-2x^3+x^4+x^5+x^6+x^7) \\
& + q^{136}x^{45}(2+x^2-3x^3-9x^4-x^5+2x^6+x^7-x^8) + q^{141}x^{48}(-4+x-3x^3+x^4+x^5-6x^6+x^8) \\
& + q^{172}x^{55}(-1+2x^2+3x^3-2x^4+x^5+x^6+x^8) + q^{182}x^{58}(1+x-2x^3-x^4+3x^5+3x^6+x^8) \\
& - q^{183}x^{57}(-1+x^2+x^4+2x^5-x^6-4x^7+x^8) - q^{176}x^{57}(1-x-2x^2+x^3+4x^4-x^6-2x^7+x^8) \\
& - q^{155}x^{51}(-1-3x+x^3-x^4+x^6-2x^7+x^8) - q^{19}x^6(2-x^5+x^6+x^7+x^8) \\
& - q^{187}x^{59}(-1+x^3-x^4-3x^5+2x^7+x^8) + q^{23}x^9(-1+x^2-x^3-2x^4+3x^8) \\
& + q^{140}x^{45}(1+2x-2x^2+x^3+x^4-5x^5-2x^6+5x^7+x^8-3x^9) \\
& + q^{133}x^{44}(-1+2x+3x^3+x^4-2x^5+x^7-2x^9) + q^{167}x^{52}(1-2x^2+x^3+3x^4+2x^6+6x^7-x^8-x^9) \\
& + q^{168}x^{54}(-1+x^2+x^3+x^4+4x^5-2x^7+x^8-x^9) \\
& + q^{171}x^{55}(-1-2x+x^3+2x^4+x^5-2x^6-x^7+x^8-x^9) \\
& + q^{148}x^{49}(-1-x+5x^2+x^3+x^4+3x^5+x^6+2x^7+3x^8-x^9) + q^{21}x^7(1+x+3x^2-2x^5-x^7+x^9) \\
& - q^{151}x^{49}(1-x^2+x^3-x^4-2x^6+2x^7+x^9) - q^{142}x^{46}(-3-x+x^2+3x^3+x^6+x^7-3x^8+x^9) \\
& + q^{125}x^{43}(-1+5x^2-x^3+x^4-3x^5-2x^6-5x^7-x^8+x^9) \\
& + q^{170}x^{54}(-2+x^2-x^3-x^4+2x^5-2x^6-4x^7-x^8+x^9) \\
& - q^{153}x^{49}(3+x^2-x^3+x^4-3x^5+3x^6-2x^7-x^8+x^9) \\
& + q^{163}x^{52}(1-x-4x^4+4x^5+4x^6+2x^7-x^8+x^9) - q^{150}x^{50}(-3+x-2x^2-5x^3+2x^4+3x^5+x^8+x^9) \\
& + q^{166}x^{53}(-1-x^2-x^3+4x^5-x^6-3x^7+x^8+x^9) + q^{157}x^{52}(-1+x^2-x^3-4x^4+x^5-x^7+x^8+x^9) \\
& + q^{149}x^{48}(-3-2x^2-2x^3+4x^4+x^7+x^8+x^9) + q^{174}x^{55}(-1-x+x^3-x^6-x^7+2x^8+x^9) \\
& - q^{20}x^5(1-3x^3-x^5-x^6+x^7+2x^8+x^9) + q^{24}x^9(3+2x+x^2-x^3-3x^4-x^5+2x^6-x^7+2x^9) \\
& + q^{144}x^{47}(1-x-x^2-2x^3+5x^6-2x^7+x^8+2x^9) \\
& + q^{128}x^{43}(-2-x-x^3+2x^5+2x^6-x^7+5x^8+3x^9) \\
& + q^{143}x^{47}(-1-2x-x^2-2x^3+x^4+6x^5+x^6-2x^7+4x^9)
\end{aligned}$$



$$\begin{aligned}
& + q^{98} x^{32} (1 - x^2 + 6x^3 - 2x^4 - 4x^5 + 5x^7 + x^8 + x^9 - 5x^{10}) \\
& + q^{113} x^{37} (-2 + x + x^2 + x^3 - 5x^5 - 5x^6 - 2x^7 + 4x^8 + 3x^9 - 5x^{10}) \\
& + q^{27} x^{10} (-4 - x - x^3 + 2x^4 + x^5 + 2x^6 + x^7 + 2x^8 + x^9 - 3x^{10}) \\
& + q^{146} x^{48} (-1 - x^2 + x^3 + x^4 - 2x^5 + x^6 + 3x^8 - x^{10}) \\
& - q^{131} x^{43} (2 + x - 3x^2 - 4x^3 - x^4 + x^5 + 3x^6 + 2x^7 + x^{10}) \\
& - q^{154} x^{49} (1 - 6x^2 + x^3 + 2x^4 - x^5 + x^6 + 5x^7 + x^{10}) \\
& + q^{147} x^{47} (1 - 3x^2 + x^3 + 2x^4 + x^5 + 2x^6 - x^7 - x^8 + x^{10}) \\
& - q^{179} x^{56} (-1 - x^3 + x^4 + 4x^5 + x^6 + x^8 + x^{10}) + q^{169} x^{52} (1 - x^3 - x^5 - x^7 + x^8 - 3x^9 + x^{10}) \\
& + q^{145} x^{47} (-1 + x - 3x^2 + x^3 - x^6 - 3x^8 - 2x^9 + x^{10}) \\
& - q^{152} x^{49} (-1 + x - x^2 - 2x^3 - 3x^4 + 2x^5 + x^6 - x^7 + x^9 + x^{10}) \\
& - q^{162} x^{51} (-2 - 3x^3 + x^6 + 2x^7 + x^9 + x^{10}) \\
& - q^{139} x^{45} (-1 - 2x^2 + x^3 + 4x^4 - x^5 - 2x^6 + x^7 + 2x^8 + x^9 + x^{10}) \\
& + q^{22} x^7 (1 + x - x^3 - 4x^4 - x^5 + x^7 - 4x^8 + x^9 + 2x^{10}) \\
& + q^{31} x^{11} (-3 - x^2 + 2x^3 + 6x^4 + 2x^5 - 4x^6 + x^7 - 4x^9 - 2x^{11}) \\
& + q^{134} x^{43} (-2 + 3x^2 + 3x^3 - 6x^4 + x^5 - 3x^7 + x^8 + 2x^9 + x^{10} - 2x^{11}) \\
& + q^{127} x^{42} (-3 + 3x^2 + 2x^3 - x^4 + 5x^5 + 4x^6 - 4x^7 + x^8 + 2x^9 - x^{11}) \\
& - q^{122} x^{39} (-2 + x^3 - x^4 + 3x^5 - 3x^6 + x^7 - 4x^8 - 2x^9 + x^{11}) \\
& + q^{137} x^{45} (2 + 2x - 3x^2 + 2x^3 - x^4 - 4x^5 - x^6 - 2x^8 - 2x^9 + x^{11}) \\
& + q^{32} x^{12} (-2 + x + x^2 + 3x^3 - 4x^4 + 3x^5 + 2x^6 - 2x^8 - 2x^9 + x^{11}) \\
& + q^{47} x^{16} (-1 - 2x - x^2 + 2x^3 + 5x^4 + 5x^5 - 4x^6 - x^7 - 4x^8 - x^9 - 7x^{10} + x^{11}) \\
& - q^{37} x^{14} (1 - 5x - 4x^2 + x^3 + 5x^6 + 2x^7 - 3x^8 - 2x^9 - 3x^{10} + x^{11}) \\
& + q^{117} x^{39} (2 + 2x + x^4 - 4x^5 + 4x^6 + 2x^7 + 2x^8 - 8x^9 - x^{10} + x^{11}) \\
& - q^{26} x^8 (-2 + x + x^2 + 6x^4 + 2x^5 + x^6 - 2x^7 - x^8 - x^9 - x^{10} + x^{11}) \\
& + q^{61} x^{21} (2 + 4x + x^2 - 4x^3 - 2x^4 + 6x^5 - x^6 + x^7 + 2x^8 - x^9 - x^{10} + x^{11}) \\
& - q^{158} x^{49} (1 + x - 3x^3 - 3x^4 - x^5 - 2x^7 + x^8 + 2x^9 - x^{10} + x^{11}) \\
& - q^{28} x^8 (-2 - x^4 + 3x^6 + x^7 - 2x^8 - 2x^9 + x^{10} + x^{11}) \\
& - q^{29} x^{10} (1 + x + 2x^2 - 3x^4 - 4x^6 - 6x^7 - x^8 + 2x^9 + x^{10} + x^{11}) \\
& + q^{138} x^{44} (1 - x + x^3 - 4x^4 + x^5 + 4x^7 + 4x^8 + 2x^9 + x^{10} + x^{11}) \\
& - q^{42} x^{16} (3 + 3x + 3x^2 + 2x^3 - x^5 - 4x^6 - 8x^7 + 3x^9 + x^{10} + x^{11}) \\
& + q^{121} x^{40} (3 - 6x^2 + 3x^4 - 3x^5 - x^6 + x^7 - 4x^9 + 2x^{10} + x^{11}) \\
& - q^{109} x^{35} (-1 + 2x^2 + 2x^3 - x^4 + x^5 + 9x^7 - 4x^8 - 3x^9 + 2x^{10} + x^{11}) \\
& - q^{130} x^{42} (1 + x + x^2 + x^3 + x^4 - 6x^5 - 2x^6 + 5x^7 + x^8 - 3x^9 + 2x^{11}) \\
& + q^{123} x^{40} (1 - 2x^2 - x^3 - x^4 + 3x^5 + 6x^6 - x^7 + 2x^8 + 3x^9 + 2x^{10} + 2x^{11}) \\
& + q^{135} x^{42} (-1 + 2x^3 + x^4 + 4x^5 - 4x^8 - 4x^9 - 3x^{12}) \\
& + q^{25} x^7 (1 + x + x^3 - 3x^4 - 2x^5 - 3x^6 - x^7 + x^8 + x^9 + 2x^{10} + x^{11} - x^{12})
\end{aligned}$$

$$\begin{aligned}
& + q^{165} x^{51} (1 - x^4 - 4x^5 - x^6 + x^7 + x^8 + x^9 + x^{12}) \\
& - q^{178} x^{54} (1 + x^3 - 2x^5 + x^6 + x^7 + x^8 - x^{10} + x^{12}) \\
& - q^{118} x^{39} (-1 - 4x + 7x^3 + 4x^4 - 2x^5 + 4x^6 - x^8 + 3x^9 + x^{10} + x^{12}) \\
& - q^{124} x^{40} (-1 + 4x^2 + 3x^3 - 3x^4 + 3x^5 + 2x^6 - 3x^7 + 2x^8 + 2x^9 + x^{10} - 3x^{11} + x^{12}) \\
& - q^{50} x^{16} (2 + 2x + x^2 + 4x^3 + 3x^4 - 7x^5 + 2x^6 + x^7 + 7x^9 + 5x^{10} - 3x^{11} + x^{12}) \\
& - q^{132} x^{42} (1 - 3x^2 + x^3 - 2x^4 + x^5 - 3x^7 + x^9 - 5x^{10} - x^{11} + x^{12}) \\
& + q^{112} x^{36} (-3 - 2x + x^2 + 3x^3 + 7x^4 - 2x^6 - 4x^7 - 2x^8 + 3x^9 - x^{10} - x^{11} + x^{12}) \\
& - q^{119} x^{39} (-2 + x^3 + 6x^4 - 3x^5 + 3x^6 + 2x^7 - 2x^8 - 5x^9 + x^{11} + x^{12}) \\
& - q^{114} x^{37} (-1 + 3x - 6x^2 - 5x^3 - 2x^5 - 3x^6 + 4x^7 + 3x^8 - 3x^9 + 2x^{10} + x^{11} + x^{12}) \\
& - q^{126} x^{40} (-1 + x^2 + 6x^3 + 3x^4 - 2x^5 - 4x^6 + x^7 - x^9 - 2x^{10} + 2x^{11} + x^{12}) \\
& + q^{115} x^{37} (-1 + x + 6x^3 + x^5 + 6x^6 - 2x^7 - 6x^8 + 2x^9 + 5x^{10} + 2x^{12}) \\
& + q^{116} x^{37} (-1 + 2x^2 + x^3 - x^4 - 4x^6 + x^7 - 3x^8 - 3x^9 - 3x^{10} - 3x^{11} + 2x^{12}) \\
& + q^{96} x^{32} (-3 + 2x + 5x^2 - x^3 - 8x^4 - x^5 + 3x^6 - x^7 - 5x^8 + 5x^9 - 4x^{10} - x^{11} + 2x^{12}) \\
& + q^{120} x^{38} (-1 + x^2 - 5x^4 - 3x^5 - 2x^6 + x^8 + x^{10} - 2x^{11} + 3x^{12}) \\
& + q^{107} x^{34} (3 + x - 2x^2 - 3x^3 + 7x^5 + 4x^6 + 7x^8 - 3x^9 + 7x^{11} + 4x^{12} - 2x^{13}) \\
& - q^{111} x^{35} (1 + 2x^2 + 2x^3 - 2x^4 + x^6 - x^7 + 2x^8 + 2x^9 - 5x^{10} - 2x^{11} + x^{13}) \\
& + q^{36} x^{12} (2 - x + 3x^2 + 3x^3 + x^4 - 5x^5 - 3x^6 + 3x^7 + x^8 + x^9 - x^{10} + 2x^{11} + x^{13}) \\
& + q^{30} x^9 (1 - x - 2x^2 - x^3 - x^4 + 2x^6 + 2x^8 + 3x^9 - 3x^{10} - 3x^{11} - x^{12} + x^{13}) \\
& + q^{108} x^{35} (-1 + x^2 + 3x^3 + 4x^4 - 2x^5 - x^6 - 2x^7 - 3x^9 - 2x^{11} + x^{12} + x^{13}) \\
& + q^{34} x^{11} (-1 - x + 2x^2 + x^3 + 3x^4 - 2x^5 - 3x^6 - 4x^7 - 5x^9 - x^{10} + 3x^{11} + x^{12} + x^{13}) \\
& + q^{78} x^{26} (-1 + 8x^2 - 5x^3 - 3x^4 - 9x^5 + x^6 - 2x^7 - 2x^8 + 3x^9 + 4x^{10} - 2x^{11} + 2x^{12} + x^{13}) \\
& + q^{91} x^{29} (1 + x - 2x^2 - x^3 + 4x^4 + 2x^5 - 5x^6 - 2x^7 + 6x^8 - 10x^9 - 7x^{10} + 6x^{11} + 4x^{12} + x^{13}) \\
& + q^{99} x^{31} (-1 + 3x^2 + 5x^3 - 5x^4 - 5x^5 - 4x^6 + 4x^7 + 2x^8 - 3x^9 + 6x^{11} + 2x^{13}) \\
& + q^{95} x^{31} (-1 + 2x + x^2 - 2x^3 + x^5 + 2x^6 + 4x^7 - 5x^8 - x^9 + x^{10} + 4x^{11} + x^{12} + 2x^{13}) \\
& + q^{38} x^{12} (-1 + x^2 + x^3 + 2x^4 - x^5 - 5x^6 - 3x^7 + x^8 + x^9 + 5x^{10} + 3x^{12} + 2x^{13}) \\
& + q^{104} x^{32} (1 - x + x^2 + 2x^3 - 3x^4 - x^5 + 3x^6 + 5x^7 - x^8 + 2x^9 + x^{10} - x^{11} - 7x^{12} + 3x^{13}) \\
& + q^{35} x^{10} (-2 - 3x^2 - 2x^3 + 2x^4 + x^6 - x^7 - x^8 - 2x^9 - 3x^{10} - 4x^{11} - x^{12} + 3x^{13}) \\
& - q^{67} x^{22} (-1 + 2x^2 + 5x^3 - 6x^4 + 6x^5 + 3x^6 - 2x^7 - 4x^8 + x^9 + 2x^{10} + 2x^{11} + x^{12} + 3x^{13}) \\
& + q^{46} x^{14} (1 + x - 3x^3 - 2x^4 + 5x^6 - 2x^7 - x^8 + x^9 + 4x^{10} - 2x^{12} - 3x^{13} - 4x^{14}) \\
& + q^{85} x^{27} (1 + x^3 - 2x^5 + 6x^6 - x^7 + x^8 + 2x^{10} - x^{11} + 3x^{12} - 5x^{13} - 2x^{14}) \\
& + q^{94} x^{29} (1 - x - 6x^2 + x^3 + 4x^4 + 3x^5 - 6x^6 + x^7 + 3x^8 + x^9 - 3x^{10} + 9x^{11} + 3x^{12} - 3x^{13} - 2x^{14}) \\
& + q^{88} x^{27} (1 - x^2 + x^3 - 5x^4 + 14x^6 + x^7 - 7x^8 - x^9 - 2x^{10} - 3x^{11} + x^{12} - 2x^{13} - 2x^{14}) \\
& + q^{77} x^{25} (-1 - 3x + 3x^2 + x^3 - 6x^5 + 5x^6 - 8x^9 + 7x^{10} - 7x^{11} + x^{12} + x^{13} - 2x^{14}) \\
& + q^{106} x^{33} (1 - x^2 - x^3 + x^4 - 2x^5 + 4x^6 + 4x^7 + x^8 - x^{12} + 2x^{13} - 2x^{14}) \\
& + q^{81} x^{26} (2 + 2x + 4x^2 + x^3 - 5x^4 + 4x^6 + x^7 - 3x^8 + 4x^{10} + 3x^{11} - 2x^{12} - x^{14})
\end{aligned}$$

$$\begin{aligned}
& + q^{33}x^9(1 - 2x^2 + 4x^5 + 2x^6 + 4x^7 + 3x^9 - 6x^{10} - 3x^{11} + 2x^{13} - x^{14}) \\
& + q^{101}x^{30}(-1 + 2x^4 + 3x^5 - 6x^6 - 6x^7 - 2x^8 + 3x^9 - 5x^{10} + 3x^{11} + x^{12} - 7x^{13} + x^{14}) \\
& + q^{129}x^{40}(1 - x^2 - 2x^3 + 2x^4 + 3x^5 + 5x^6 + 2x^8 - 3x^{10} + x^{13} + x^{14}) \\
& - q^{43}x^{14}(1 - 2x - x^2 + 2x^4 - 2x^5 + 2x^8 - x^{10} + x^{13} + x^{14}) \\
& - q^{84}x^{25}(1 - x + 3x^3 - x^4 + 2x^5 + x^6 + x^7 + 4x^8 - x^9 - 6x^{10} - x^{11} + 2x^{12} + x^{13} + x^{14}) \\
& + q^{93}x^{30}(-2 + x - x^2 + x^3 + 2x^4 - 3x^5 - 6x^6 - 8x^7 - x^8 - x^{10} - 6x^{12} + 2x^{14}) \\
& - q^{41}x^{13}(-1 - 2x + x^2 + x^3 + 2x^4 - 2x^5 - 2x^6 - 2x^7 + x^8 + 3x^9 + x^{10} - x^{13} + 2x^{14}) \\
& - q^{86}x^{28}(-3 + 3x + 2x^2 + 4x^3 - 9x^4 - 2x^5 + 2x^6 + 3x^7 - 9x^8 - 2x^{10} + x^{11} + x^{12} + x^{13} + 2x^{14}) \\
& + q^{39}x^{11}(-2 + x^3 + 2x^4 + x^6 - 4x^7 + x^8 - 2x^{10} + 2x^{11} + 5x^{12} + x^{13} + 2x^{14}) \\
& + q^{71}x^{22}(1 - x - x^2 - 4x^4 + 2x^5 + 2x^6 - x^7 + 4x^8 + 3x^9 + 3x^{10} + x^{11} - 3x^{12} + 3x^{13} + 2x^{14}) \\
& - q^{83}x^{27}(1 - x + 9x^3 + 4x^4 - 7x^5 - 9x^6 - 8x^7 - 2x^8 + 5x^9 + 7x^{10} + x^{11} - 3x^{12} - 2x^{13} + 3x^{14}) \\
& + q^{72}x^{24}(-2 - x + x^2 + 3x^3 + 2x^4 - 5x^5 - x^6 + x^7 - 6x^8 + 3x^9 + 5x^{10} - 9x^{11} - x^{12} + 2x^{13} + 3x^{14}) \\
& - q^{45}x^{13}(-1 - 2x + 2x^3 + 2x^4 + 7x^5 - 3x^6 - 2x^7 - 4x^{10} + 3x^{11} + 2x^{12} + x^{13} + 4x^{14}) \\
& + q^{110}x^{33}(1 - 2x^3 - 3x^4 + x^5 - x^6 + x^8 + 2x^9 - 3x^{10} + x^{11} + x^{12} - 2x^{14} - 2x^{15}) \\
& + q^{90}x^{27}(1 + x - x^3 + x^4 + x^5 - x^7 - 2x^9 - x^{10} + 4x^{12} + 3x^{13} - 2x^{14} - 2x^{15}) \\
& + q^{59}x^{19}(-1 + 5x^2 + x^3 - 8x^4 - x^5 + x^7 - 2x^8 + x^9 + x^{10} - 3x^{11} + 2x^{12} + 5x^{13} - 2x^{14} - x^{15}) \\
& + q^{40}x^{11}(-1 + 4x^2 + x^3 + 2x^4 - 5x^6 - x^7 - 2x^8 - 2x^9 + x^{10} + 5x^{11} + 5x^{12} + 2x^{14} - x^{15}) \\
& - q^{105}x^{31}(1 - 3x^2 + x^5 + 3x^6 - x^7 + x^8 + 2x^9 - x^{10} - 4x^{11} + 2x^{12} - 3x^{13} + x^{15}) \\
& + q^{97}x^{30}(-1 + 3x^3 + 2x^4 - 3x^5 + 3x^7 - 3x^8 - 7x^9 + 9x^{10} + 2x^{11} - x^{12} - 2x^{13} + x^{15}) \\
& + q^{63}x^{20}(1 + x + 4x^2 + x^3 - 3x^4 - 6x^5 - 3x^6 + 3x^7 + 10x^8 + 2x^9 + 9x^{10} - 7x^{11} - 4x^{12} - 4x^{14} + x^{15}) \\
& + q^{54}x^{16}(-1 - 2x^3 + 2x^4 + 2x^5 + x^6 - 5x^7 + 5x^8 + 6x^9 + 4x^{11} + 4x^{12} + x^{13} - 2x^{14} + x^{15}) \\
& - q^{102}x^{31}(2 - x^3 + x^4 + 3x^5 + 3x^6 - 2x^7 + 3x^8 - 4x^9 - 4x^{10} - 2x^{11} + 6x^{12} + x^{13} - x^{14} + x^{15}) \\
& + q^{74}x^{23}(-1 - 2x + 2x^3 + x^4 + 5x^5 + 2x^6 - 3x^7 - x^9 - 6x^{10} + 6x^{11} + 4x^{12} - x^{13} + 3x^{14} + x^{15}) \\
& + q^{92}x^{28}(2 - 3x^2 - x^3 + x^4 - x^5 + x^6 + x^7 + 5x^9 - 8x^{10} - 2x^{11} - 2x^{13} - 2x^{14} + 3x^{15}) \\
& + q^{80}x^{24}(-1 + x - x^2 + x^3 - x^4 - 3x^5 - x^6 - x^7 + 3x^8 - 3x^9 + 5x^{10} + 3x^{11} + 2x^{12} - 2x^{13} + 3x^{14} + 4x^{15}) \\
& + q^{103}x^{30}(-1 + x^3 - x^4 - 2x^5 - 2x^7 - x^8 - 5x^9 + 8x^{10} - 7x^{12} + 3x^{13} + 4x^{14} + 4x^{15}) \\
& + q^{58}x^{17}(-1 + x^2 + 2x^4 - x^5 + 5x^6 - 7x^7 + 2x^8 - 3x^9 + x^{10} - 9x^{11} + 3x^{12} + x^{13} + 4x^{14} - 2x^{16}) \\
& + q^{52}x^{15}(-1 - x^2 - x^3 - x^4 + 5x^5 - 2x^6 + 2x^8 + x^9 - 4x^{10} + x^{12} + 3x^{13} - x^{14} + x^{16}) \\
& + q^{57}x^{17}(-1 - x - 2x^2 + 2x^3 + x^4 - 5x^6 + x^8 + 3x^9 - 4x^{10} + 8x^{11} - 3x^{13} - x^{14} + x^{15} + x^{16}) \\
& + q^{75}x^{23}(1 - x + 5x^3 + 2x^4 - 3x^5 - 2x^6 - 5x^7 + 5x^8 + 10x^{11} - 4x^{12} - 3x^{13} + 5x^{14} + 2x^{15} + x^{16}) \\
& - q^{62}x^{19}(1 - 3x^2 - 2x^3 + 3x^4 + 2x^5 - 6x^6 + x^8 + x^9 + x^{10} + 7x^{11} + x^{12} - 6x^{13} - 2x^{14} + 4x^{15} + x^{16}) \\
& - q^{73}x^{21}(-1 + x^2 + 2x^3 + x^4 - 4x^5 - 4x^6 - 3x^7 - x^8 + 2x^9 + 3x^{10} + x^{11} + 3x^{12} - 2x^{13} + x^{14} + 6x^{15} + x^{16}) \\
& - q^{68}x^{20}(-1 - 2x + 2x^3 + x^4 + 3x^5 + 5x^6 - 6x^7 - 2x^8 + 5x^{10} + 5x^{11} + 6x^{13} - 2x^{14} + 2x^{16}) \\
& + q^{49}x^{14}(1 + x^2 + x^3 - 4x^4 - 2x^5 + 2x^6 + 4x^7 - x^8 - 5x^9 - 2x^{10} - 4x^{11} + 2x^{12} + 2x^{14} + 2x^{16}) \\
& - q^{60}x^{17}(1 + x + x^2 - x^3 - 3x^4 + 3x^6 + x^7 - 2x^8 - 3x^9 - 3x^{10} + x^{11} - x^{12} + 4x^{13} + 3x^{14} - 2x^{15} + 2x^{16})
\end{aligned}$$

$$\begin{aligned}
& -q^{82}x^{25}(-1-x^2-2x^4+x^5+x^6+x^7-2x^9+x^{10}-5x^{11}-3x^{12}-4x^{13}+2x^{15}+2x^{16}) \\
& +q^{70}x^{21}(-1-2x^2-3x^3-x^4+5x^5+4x^6+x^7+x^8-2x^9-7x^{10}+8x^{12}+x^{13}-3x^{14}+2x^{15}+2x^{16}) \\
& +q^{76}x^{23}(1-3x^2+x^3+5x^4+3x^5-x^6-x^7-6x^8-4x^9-5x^{10}+3x^{11}+4x^{12}+3x^{13}-x^{14}+5x^{15}+2x^{16}) \\
& +q^{56}x^{16}(-2+x+4x^5+4x^6-2x^7+3x^8+5x^9-3x^{10}-8x^{11}+3x^{12}+4x^{14}+3x^{15}-x^{16}-x^{17}) \\
& +q^{89}x^{26}(-1+2x^2-3x^4+2x^5+2x^6+4x^7+4x^8+x^9+2x^{10}-5x^{11}-7x^{12}-6x^{15}+x^{17}) \\
& +q^{48}x^{13}(1+4x^3+2x^4-2x^5-5x^6+3x^7+2x^9-x^{10}-2x^{11}+3x^{12}+3x^{13}-5x^{14}-4x^{15}+x^{17}) \\
& -q^{87}x^{25}(1-x^2+x^5+3x^6+x^7-x^8+x^9-6x^{10}-2x^{11}+7x^{12}+5x^{13}-3x^{15}+x^{16}+x^{17}) \\
& +q^{53}x^{14}(1-x^2+x^3-x^5+5x^7+2x^8-3x^9-2x^{10}+4x^{11}-5x^{12}+4x^{13}+x^{14}+4x^{16}+x^{17}) \\
& -q^{79}x^{23}(1+x^2+x^5+x^6+3x^7+3x^8+3x^9-5x^{10}+4x^{11}-3x^{12}+x^{13}-4x^{15}-2x^{16}+2x^{17}) \\
& +q^{66}x^{19}(1+2x^3+2x^4-4x^5-x^6+7x^8-2x^9-2x^{10}-5x^{11}+9x^{12}-5x^{13}+x^{14}-x^{15}-2x^{16}+2x^{17}) \\
& -q^{44}x^{11}(1+x-2x^3-2x^4-4x^5+2x^6+3x^7-7x^9-x^{10}-4x^{11}+2x^{12}-3x^{13}+5x^{14}+5x^{15} \\
& +x^{16}+2x^{17}) \\
& +q^{100}x^{28}(1+x^5+x^6-x^7+2x^9-2x^{10}+5x^{11}+4x^{12}+4x^{13}-3x^{14}-x^{15}+2x^{16}+2x^{17}) \\
& +q^{69}x^{19}(1-x^4-x^5-2x^6+4x^8-x^9-x^{10}+8x^{11}+2x^{12}-5x^{13}+3x^{14}-4x^{15}-5x^{16}-3x^{17}+x^{18}) \\
& -q^{65}x^{18}(-1-x^3-2x^4+4x^5+x^6+4x^7+3x^9-3x^{10}-2x^{11}-x^{12}+3x^{13}-2x^{14}-2x^{15}+x^{16} \\
& +3x^{17}+x^{18}) \\
& +q^{55}x^{14}(1-x^3-x^4-x^5+x^6+x^7+x^8-3x^9-4x^{10}-2x^{11}+3x^{12}+5x^{13}+6x^{14}+2x^{15}+x^{16} \\
& +5x^{17}+x^{18}) \\
& +q^{51}x^{13}(1-3x^5-x^7+3x^8-7x^9-x^{10}+x^{11}-2x^{12}+2x^{13}-x^{14}-4x^{15}+x^{16}+4x^{17}+2x^{18}) \\
& -q^{64}x^{16}(1+x^3+x^4-2x^5-x^6-2x^7+7x^8-4x^9-7x^{10}+2x^{11}+11x^{12}-2x^{13}-2x^{14}+9x^{15}+2x^{16} \\
& -4x^{17}+x^{18}+x^{19})+q^{214}(x^{66}+x^{71})-q^{216}(x^{69}+x^{73})+q^{218}(x^{70}-x^{74}) \\
& +q^{224}(x^{71}-x^{74})]
\end{aligned}$$

$$\begin{aligned}
h_5 = & -q^{411}x^{36}[1-(1+q+q^3+q^4+q^5+q^6)x+(q+q^3+q^4+2q^5+2q^6+2q^7+q^8+2q^9+q^{10}+q^{11})x^2 \\
& -q^6(1+q+q^2+2q^3+2q^4+2q^5+2q^6+q^7+q^8+q^9)x^3 \\
& +q^5(-1-q^2-q^3-q^4-q^6+q^7+q^9+q^{10}+q^{11}+q^{13})x^4 \\
& +q^8(1+q+q^2+2q^3+2q^4+2q^5+2q^6+q^7+q^8+q^9)x^5 \\
& -q^{12}(1+q+2q^2+q^3+2q^4+2q^5+2q^6+q^7+q^8+q^{10})x^6 \\
& +q^{17}(1+q+q^2+q^3+q^5+q^6)x^7-q^{23}x^8]^2 \times \\
& [1-qx^2+2q^{168}(1-2x)x^{55}-q^{171}x^{57}-2q^{172}x^{58}+q^{174}x^{59}+3q^{166}x^{54}(-1+2x) \\
& +q^{170}x^{56}(-1+3x)+q^{165}x^{52}(3+5x^2-x^3)-2q^2(x+x^3)+q^3x^2(-1+2x+x^3) \\
& +q^{167}x^{53}(-2-3x^2+x^3)-q^{164}x^{52}(1-4x+6x^2+x^4) \\
& +q^5x^3(1-3x+3x^2-2x^3+x^4)+q^4x^2(3+5x^2-x^3+x^4) \\
& +q^{162}x^{51}(1-5x+6x^2+2x^4)-q^7x^4(1-4x+4x^2-4x^3+4x^4)
\end{aligned}$$

$$\begin{aligned}
& + q^{160}x^{50}(-1+5x-6x^2+x^3-3x^4+x^5) + q^6x^3(-4-7x^2+2x^3-3x^4+x^5) \\
& + q^{159}x^{49}(-5-7x^2+x^3-2x^4+2x^5-3x^6) - q^{163}x^{51}(4+6x^2-x^3+x^6) \\
& + q^{161}x^{50}(5+6x^2-x^3+x^4+2x^6) - q^8x^3(1-5x-9x^3+4x^4-5x^5+3x^6) \\
& + q^{157}x^{48}(5+8x^2-x^3+3x^4-3x^5+4x^6) \\
& + q^{150}x^{45}(1-5x+7x^2-10x^3+9x^4-12x^5+8x^6-13x^7) \\
& + q^{154}x^{47}(1-5x+7x^2-7x^3+7x^4-8x^5+3x^6-6x^7) \\
& + q^{158}x^{49}(1-5x+6x^2-3x^3+4x^4-3x^5+x^6-2x^7) \\
& - q^{10}x^4(-3+5x-2x^2+11x^3-5x^4+7x^5-5x^6+x^7) \\
& + q^{155}x^{47}(-5-9x^2+x^3-5x^4+5x^5-6x^6+2x^7) \\
& + q^{156}x^{48}(-1+5x-6x^2+5x^3-6x^4+5x^5-x^6+4x^7) \\
& + q^{152}x^{46}(-1+5x-7x^2+9x^3-8x^4+10x^5-5x^6+8x^7) \\
& + q^{153}x^{46}(5+10x^2-2x^3+6x^4-9x^5+7x^6-4x^7+3x^8) \\
& - q^{151}x^{45}(5+11x^2-3x^3+5x^4-13x^5+7x^6-6x^7+4x^8) \\
& + q^{12}x^4(1-5x+5x^2-6x^3+12x^4-7x^5+9x^6-6x^7+4x^8) \\
& + q^{11}x^3(2+3x^2-3x^3+5x^4-7x^5+6x^6-9x^7+5x^8) \\
& + q^{15}x^5(5+9x^2-7x^3+12x^4-12x^5+10x^6-12x^7+9x^8-3x^9) \\
& + q^{13}x^4(-3-6x^2+5x^3-9x^4+9x^5-7x^6+11x^7-7x^8+2x^9) \\
& + q^{19}x^6(-3+8x-6x^2+17x^3-15x^4+20x^5-19x^6+16x^7-17x^8+11x^9-5x^{10}) \\
& + q^{149}x^{44}(5+11x^2-3x^3+4x^4-17x^5+7x^6-11x^7+5x^8+x^{10}) \\
& - q^{148}x^{44}(1-5x+7x^2-11x^3+9x^4-15x^5+11x^6-14x^7+x^8-2x^9+x^{10}) \\
& + q^{146}x^{43}(1-5x+7x^2-11x^3+10x^4-16x^5+14x^6-15x^7+x^8-5x^9+2x^{10}) \\
& - q^9(x^2-2x^5+5x^6-5x^7+5x^8-6x^9+3x^{10}) \\
& + q^{17}x^5(2-7x+x^2-13x^3+10x^4-16x^5+15x^6-12x^7+15x^8-11x^9+4x^{10}) \\
& - q^{144}x^{42}(1-5x+7x^2-10x^3+10x^4-17x^5+15x^6-18x^7+4x^8-9x^9+5x^{10}) \\
& - q^{14}x^3(1+2x^2-7x^3+8x^4-9x^5+14x^6-9x^7+11x^8-7x^9+5x^{10}) \\
& + q^{21}x^7(4-9x+10x^2-21x^3+21x^4-25x^5+23x^6-21x^7+19x^8-13x^9+6x^{10}) \\
& + q^{136}x^{39}(3-6x+7x^2-7x^3+18x^4-16x^5+21x^6-22x^7+29x^8-21x^9+4x^{10}-6x^{11}) \\
& + q^{23}x^7(1-6x+10x^2-13x^3+24x^4-26x^5+31x^6-26x^7+26x^8-21x^9+13x^{10}-6x^{11}) \\
& + q^{141}x^{40}(2+7x^2-x^3+5x^4-22x^5+10x^6-22x^7+12x^8-13x^9+13x^{10}-5x^{11}) \\
& + q^{140}x^{41}(5-6x+9x^2-9x^3+19x^4-19x^5+19x^6-12x^7+21x^8-14x^9+x^{10}-2x^{11}) \\
& + q^{145}x^{42}(4+9x^2-3x^3+3x^4-22x^5+9x^6-16x^7+8x^8-5x^9+4x^{10}-2x^{11}) \\
& + q^{16}x^4(2+5x^2-9x^3+11x^4-13x^5+19x^6-11x^7+14x^8-7x^9+6x^{10}-x^{11}) \\
& + q^{18}x^5(-3-10x^2+11x^3-16x^4+17x^5-23x^6+16x^7-16x^8+8x^9-7x^{10}+x^{11}) \\
& - q^{20}x^6(-4+x-14x^2+12x^3-22x^4+20x^5-29x^6+21x^7-17x^8+11x^9-7x^{10}+x^{11}) \\
& + q^{147}x^{43}(-5-10x^2+3x^3-3x^4+20x^5-8x^6+14x^7-6x^8+x^9-2x^{10}+x^{11})
\end{aligned}$$

$$\begin{aligned}
& + q^{125}x^{37}(-7 + 6x - 16x^2 + 15x^3 - 20x^4 + 45x^5 - 21x^6 + 32x^7 - 26x^8 + 23x^9 - 11x^{10} + 3x^{11}) \\
& + q^{143}x^{41}(-3 - 8x^2 + 2x^3 - 4x^4 + 22x^5 - 10x^6 + 19x^7 - 10x^8 + 9x^9 - 9x^{10} + 4x^{11}) \\
& + q^{138}x^{40}(-4 + 6x - 8x^2 + 8x^3 - 19x^4 + 17x^5 - 21x^6 + 18x^7 - 25x^8 + 18x^9 - 2x^{10} + 4x^{11}) \\
& + q^{110}x^{32}(-4 + 4x - 10x^2 + 19x^3 - 21x^4 + 32x^5 - 34x^6 + 49x^7 - 35x^8 + 31x^9 - 32x^{10} + 11x^{11} - 8x^{12}) \\
& + q^{119}x^{35}(-4 + 10x - 10x^2 + 14x^3 - 32x^4 + 17x^5 - 37x^6 + 38x^7 - 35x^8 + 24x^9 - 11x^{10} + 9x^{11} - 6x^{12}) \\
& + q^{111}x^{33}(-2 + 4x - 19x^2 + 10x^3 - 32x^4 + 36x^5 - 45x^6 + 38x^7 - 25x^8 + 36x^9 - 22x^{10} + 4x^{11} - 5x^{12}) \\
& + q^{114}x^{34}(-9 + 4x - 17x^2 + 22x^3 - 24x^4 + 37x^5 - 39x^6 + 46x^7 - 28x^8 + 22x^9 - 22x^{10} + 5x^{11} - 3x^{12}) \\
& + q^{135}x^{39}(-5 + x - 4x^2 + 18x^3 - 8x^4 + 29x^5 - 22x^6 + 20x^7 - 30x^8 + 10x^9 - 7x^{10} + 3x^{11} - 2x^{12}) \\
& + q^{22}x^6(1 - 5x + x^2 - 18x^3 + 17x^4 - 28x^5 + 25x^6 - 33x^7 + 26x^8 - 19x^9 + 12x^{10} - 7x^{11} + x^{12}) \\
& - q^{24}x^7(2 - 6x + 4x^2 - 21x^3 + 19x^4 - 34x^5 + 31x^6 - 37x^7 + 31x^8 - 20x^9 + 13x^{10} - 7x^{11} + x^{12}) \\
& - q^{122}x^{36}(3 - 9x + 19x^2 - 14x^3 + 32x^4 - 34x^5 + 29x^6 - 33x^7 + 31x^8 - 27x^9 + 12x^{10} - 3x^{11} + x^{12}) \\
& + q^{137}x^{40}(6 - x + 6x^2 - 19x^3 + 9x^4 - 27x^5 + 18x^6 - 22x^7 + 25x^8 - 9x^9 + 4x^{10} - 2x^{11} + x^{12}) \\
& + q^{142}x^{41}(1 - 5x + 6x^2 - 10x^3 + 9x^4 - 18x^5 + 18x^6 - 19x^7 + 8x^8 - 14x^9 + 9x^{10} - x^{11} + x^{12}) \\
& - q^{139}x^{39}(1 + 6x^2 - x^3 + 6x^4 - 21x^5 + 10x^6 - 24x^7 + 15x^8 - 20x^9 + 19x^{10} - 7x^{11} + 2x^{12}) \\
& + q^{112}x^{33}(6 - 4x + 14x^2 - 20x^3 + 24x^4 - 35x^5 + 36x^6 - 49x^7 + 32x^8 - 27x^9 + 27x^{10} - 8x^{11} + 4x^{12}) \\
& + q^{120}x^{35}(2 - 7x + 17x^2 - 11x^3 + 29x^4 - 33x^5 + 28x^6 - 35x^7 + 35x^8 - 32x^9 + 15x^{10} - 5x^{11} + 4x^{12}) \\
& + q^{117}x^{34}(3 - 6x + 8x^2 - 11x^3 + 28x^4 - 16x^5 + 34x^6 - 38x^7 + 40x^8 - 29x^9 + 14x^{10} - 14x^{11} + 10x^{12}) \\
& + q^{126}x^{35}(2 + x^2 - 8x^3 + 11x^4 - 22x^5 + 20x^6 - 36x^7 + 34x^8 - 32x^9 + 25x^{10} - 19x^{11} + 17x^{12} - 6x^{13}) \\
& + q^{103}x^{30}(1 - 12x + 6x^2 - 21x^3 + 31x^4 - 38x^5 + 34x^6 - 30x^7 + 41x^8 - 37x^9 + 23x^{10} - 16x^{11} + 9x^{12} - 5x^{13}) \\
& + q^{40}x^{12}(2 - 4x + 11x^2 - 17x^3 + 32x^4 - 35x^5 + 68x^6 - 55x^7 + 71x^8 - 67x^9 + 55x^{10} - 28x^{11} + 15x^{12} - 3x^{13}) \\
& + q^{30}x^8(1 - 5x + 8x^2 - 14x^3 + 15x^4 - 37x^5 + 34x^6 - 50x^7 + 42x^8 - 53x^9 + 36x^{10} - 25x^{11} + 15x^{12} - 3x^{13}) \\
& + q^{46}x^{14}(1 - 4x + 6x^2 - 14x^3 + 22x^4 - 39x^5 + 40x^6 - 76x^7 + 60x^8 - 72x^9 + 58x^{10} - 42x^{11} + 19x^{12} - 3x^{13}) \\
& + q^{123}x^{36}(4 - 6x + 13x^2 - 14x^3 + 20x^4 - 42x^5 + 22x^6 - 33x^7 + 31x^8 - 30x^9 + 16x^{10} - 4x^{11} + x^{12} - 2x^{13}) \\
& + q^{106}x^{31}(5 - 3x + 17x^2 - 14x^3 + 30x^4 - 31x^5 + 47x^6 - 38x^7 + 29x^8 - 44x^9 + 19x^{10} - 14x^{11} + 2x^{12} - 2x^{13}) \\
& + q^{107}x^{32}(2 - 16x + 8x^2 - 26x^3 + 32x^4 - 43x^5 + 39x^6 - 28x^7 + 40x^8 - 30x^9 + 13x^{10} - 9x^{11} + 2x^{12} - 2x^{13}) \\
& + q^{130}x^{37}(4 - 2x + 3x^2 - 11x^3 + 11x^4 - 23x^5 + 25x^6 - 37x^7 + 29x^8 - 22x^9 + 17x^{10} - 7x^{11} + 7x^{12} - 2x^{13}) \\
& + q^{127}x^{36}(1 + 10x^2 - 6x^3 + 19x^4 - 18x^5 + 18x^6 - 45x^7 + 20x^8 - 29x^9 + 20x^{10} - 17x^{11} + 8x^{12} - 2x^{13}) \\
& + q^{34}x^{10}(2 - 8x + 11x^2 - 23x^3 + 25x^4 - 51x^5 + 44x^6 - 62x^7 + 56x^8 - 58x^9 + 32x^{10} - 26x^{11} + 9x^{12} - 2x^{13}) \\
& + q^{109}x^{33}(-3 + 18x - 9x^2 + 29x^3 - 33x^4 + 46x^5 - 42x^6 + 26x^7 - 39x^8 + 26x^9 - 9x^{10} + 7x^{11} + x^{13}) \\
& + q^{115}x^{33}(-2 + 4x - 5x^2 + 8x^3 - 25x^4 + 13x^5 - 35x^6 + 37x^7 - 42x^8 + 34x^9 - 19x^{10} + 21x^{11} - 15x^{12} + x^{13}) \\
& + q^{26}x^7(-1 + 3x - 8x^2 + 8x^3 - 25x^4 + 23x^5 - 37x^6 + 35x^7 - 45x^8 + 34x^9 - 23x^{10} + 14x^{11} - 5x^{12} + x^{13}) \\
& - q^{133}x^{38}(-3 + x - 3x^2 + 17x^3 - 8x^4 + 27x^5 - 22x^6 + 18x^7 - 37x^8 + 11x^9 - 12x^{10} + 7x^{11} - 3x^{12} + x^{13}) \\
& + q^{134}x^{38}(-2 + 6x - 5x^2 + 6x^3 - 15x^4 + 15x^5 - 21x^6 + 23x^7 - 33x^8 + 26x^9 - 9x^{10} + 11x^{11} - x^{12} + x^{13}) \\
& + q^{32}x^9(-1 + 7x - 9x^2 + 20x^3 - 22x^4 + 42x^5 - 39x^6 + 56x^7 - 49x^8 + 56x^9 - 34x^{10} + 26x^{11} - 13x^{12} + 2x^{13}) \\
& + q^{131}x^{37}(-2 + x - 2x^2 + 16x^3 - 7x^4 + 25x^5 - 21x^6 + 16x^7 - 43x^8 + 14x^9 - 17x^{10} + 10x^{11} - 6x^{12} + 2x^{13})
\end{aligned}$$

$$\begin{aligned}
& + q^{116} x^{34} (-3 + 14x - 5x^2 + 20x^3 - 24x^4 + 26x^5 - 37x^6 + 38x^7 - 40x^8 + 26x^9 - 16x^{10} + 14x^{11} - 3x^{12} + 2x^{13}) \\
& + q^{105} x^{31} (-1 + 13x - 8x^2 + 24x^3 - 30x^4 + 43x^5 - 36x^6 + 29x^7 - 41x^8 + 34x^9 - 18x^{10} + 13x^{11} - 6x^{12} + 3x^{13}) \\
& + q^{128} x^{36} (-3 + x - 2x^2 + 9x^3 - 11x^4 + 24x^5 - 22x^6 + 38x^7 - 32x^8 + 26x^9 - 22x^{10} + 14x^{11} - 11x^{12} + 4x^{13}) \\
& + q^{121} x^{35} (-1 + 6x - 12x^2 + 12x^3 - 19x^4 + 36x^5 - 20x^6 + 36x^7 - 34x^8 + 33x^9 - 20x^{10} + 7x^{11} - 3x^{12} + 4x^{13}) \\
& + q^{38} x^{11} (-1 + 3x - 11x^2 + 14x^3 - 30x^4 + 34x^5 - 61x^6 + 53x^7 - 68x^8 + 64x^9 - 60x^{10} + 28x^{11} - 21x^{12} + 5x^{13}) \\
& - q^{129} x^{36} (-1 + x + 14x^3 - 6x^4 + 22x^5 - 21x^6 + 16x^7 - 46x^8 + 17x^9 - 24x^{10} + 15x^{11} - 12x^{12} + 5x^{13}) \\
& + q^{101} x^{29} (-1 + 12x - 9x^2 + 17x^3 - 27x^4 + 37x^5 - 33x^6 + 31x^7 - 40x^8 + 35x^9 - 29x^{10} + 18x^{11} - 12x^{12} \\
& + 6x^{13}) \\
& + q^{43} x^{12} (-3 + 3x - 5x^2 + 15x^3 - 7x^4 + 31x^5 - 33x^6 + 49x^7 - 61x^8 + 69x^9 - 68x^{10} + 62x^{11} - 39x^{12} \\
& + 18x^{13} - 10x^{14}) \\
& + q^{37} x^{10} (-3 + 2x - 8x^2 + 8x^3 - 22x^4 + 26x^5 - 45x^6 + 48x^7 - 60x^8 + 69x^9 - 57x^{10} + 47x^{11} - 29x^{12} \\
& + 21x^{13} - 6x^{14}) \\
& + q^{104} x^{30} (-5 + x - 18x^2 + 11x^3 - 29x^4 + 29x^5 - 43x^6 + 41x^7 - 30x^8 + 48x^9 - 21x^{10} + 21x^{11} - 5x^{12} \\
& + 3x^{13} - x^{14}) \\
& - q^{124} x^{34} (1 - 5x^3 + 11x^4 - 20x^5 + 17x^6 - 35x^7 + 35x^8 - 33x^9 + 30x^{10} - 24x^{11} + 23x^{12} - 10x^{13} \\
& + x^{14}) \\
& - q^{44} x^{13} (1 - 3x + 6x^2 - 14x^3 + 20x^4 - 37x^5 + 39x^6 - 73x^7 + 61x^8 - 71x^9 + 64x^{10} - 46x^{11} + 23x^{12} \\
& - 6x^{13} + x^{14}) \\
& + q^{132} x^{37} (1 - 6x + 3x^2 - 4x^3 + 13x^4 - 13x^5 + 22x^6 - 25x^7 + 34x^8 - 28x^9 + 15x^{10} - 13x^{11} + 4x^{12} \\
& - 4x^{13} + x^{14}) \\
& - q^{28} x^7 (1 - 3x + 4x^2 - 10x^3 + 11x^4 - 32x^5 + 28x^6 - 42x^7 + 39x^8 - 49x^9 + 35x^{10} - 24x^{11} + 14x^{12} \\
& - 4x^{13} + x^{14}) \\
& - q^{118} x^{34} (1 - 5x + 15x^2 - 8x^3 + 25x^4 - 28x^5 + 27x^6 - 36x^7 + 36x^8 - 36x^9 + 23x^{10} - 10x^{11} + 9x^{12} \\
& - 2x^{13} + x^{14}) \\
& + q^{108} x^{31} (2 - 5x + 5x^2 - 17x^3 + 18x^4 - 30x^5 + 33x^6 - 48x^7 + 37x^8 - 30x^9 + 40x^{10} - 16x^{11} + 11x^{12} \\
& - 2x^{13} + x^{14}) \\
& + q^{48} x^{14} (-2 - x + 5x^2 - 6x^3 + 16x^4 - 25x^5 + 40x^6 - 42x^7 + 76x^8 - 60x^9 + 69x^{10} - 49x^{11} + 38x^{12} \\
& - 13x^{13} + 2x^{14}) \\
& - q^{31} x^8 (4 + 8x^2 - 10x^3 + 15x^4 - 30x^5 + 32x^6 - 44x^7 + 51x^8 - 46x^9 + 41x^{10} - 36x^{11} + 25x^{12} \\
& - 12x^{13} + 2x^{14}) \\
& + q^{36} x^{10} (1 - 2x + 9x^2 - 14x^3 + 25x^4 - 31x^5 + 56x^6 - 48x^7 + 66x^8 - 60x^9 + 61x^{10} - 30x^{11} + 24x^{12} \\
& - 7x^{13} + 2x^{14}) \\
& + q^{102} x^{29} (5 + 18x^2 - 10x^3 + 26x^4 - 29x^5 + 39x^6 - 40x^7 + 33x^8 - 51x^9 + 25x^{10} - 23x^{11} + 7x^{12} \\
& - 6x^{13} + 2x^{14}) \\
& + q^{29} x^7 (3 + 5x^2 - 7x^3 + 12x^4 - 24x^5 + 28x^6 - 38x^7 + 42x^8 - 44x^9 + 39x^{10} - 34x^{11} + 26x^{12} - 13x^{13}
\end{aligned}$$

$$\begin{aligned}
& +3x^{14}) \\
& +q^{42}x^{12}(1-3x+4x^2-12x^3+19x^4-34x^5+38x^6-70x^7+60x^8-71x^9+65x^{10}-51x^{11}+28x^{12} \\
& -10x^{13}+3x^{14}) \\
& -q^{100}x^{28}(5+17x^2-9x^3+24x^4-27x^5+38x^6-38x^7+34x^8-52x^9+27x^{10}-24x^{11}+9x^{12} \\
& -9x^{13}+3x^{14}) \\
& +q^{113}x^{32}(1-2x+3x^2-4x^3+23x^4-11x^5+33x^6-38x^7+43x^8-37x^9+24x^{10}-31x^{11}+19x^{12} \\
& -2x^{13}+3x^{14}) \\
& -q^{27}x^6(2+2x^2-4x^3+10x^4-20x^5+22x^6-31x^7+37x^8-41x^9+34x^{10}-32x^{11}+25x^{12} \\
& -13x^{13}+4x^{14}) \\
& +q^{98}x^{27}(5+18x^2-7x^3+18x^4-27x^5+35x^6-40x^7+34x^8-50x^9+25x^{10}-26x^{11}+14x^{12} \\
& -9x^{13}+4x^{14}) \\
& +q^{25}x^5(1-3x^3+8x^4-13x^5+17x^6-27x^7+32x^8-37x^9+29x^{10}-29x^{11}+23x^{12}-13x^{13} \\
& +6x^{14}) \\
& +q^{45}x^{13}(4-2x+7x^2-13x^3+11x^4-32x^5+33x^6-54x^7+59x^8-72x^9+65x^{10}-61x^{11}+35x^{12} \\
& -15x^{13}+7x^{14}) \\
& +q^{35}x^9(2-3x+4x^2-10x^3+17x^4-23x^5+42x^6-42x^7+55x^8-64x^9+55x^{10}-45x^{11}+32x^{12} \\
& -23x^{13}+8x^{14}) \\
& +q^{53}x^{15}(-1+x+2x^2+4x^3+6x^4-10x^5+23x^6-32x^7+37x^8-60x^9+53x^{10}-56x^{11}+55x^{12} \\
& -27x^{13}+13x^{14}-4x^{15}) \\
& +q^{58}x^{16}(-1+5x-2x^2+12x^3+10x^5+4x^6-21x^7+25x^8-53x^9+45x^{10}-62x^{11}+44x^{12}-40x^{13} \\
& +17x^{14}-4x^{15}) \\
& +q^{50}x^{14}(-1+3x+x^2-2x^3+6x^4-19x^5+27x^6-42x^7+43x^8-73x^9+60x^{10}-66x^{11}+42x^{12} \\
& -30x^{13}+9x^{14}-2x^{15}) \\
& +q^{41}x^{11}(2-4x+2x^2-14x^3+7x^4-27x^5+32x^6-48x^7+58x^8-66x^9+69x^{10}-62x^{11}+43x^{12} \\
& -21x^{13}+14x^{14}-2x^{15}) \\
& -q^{99}x^{28}(-1+11x-8x^2+16x^3-23x^4+37x^5-30x^6+31x^7-44x^8+34x^9-31x^{10}+21x^{11}-18x^{12} \\
& +9x^{13}+x^{15}) \\
& +q^{54}x^{15}(2+7x^2+x^3+4x^4+2x^5-20x^6+28x^7-47x^8+47x^9-68x^{10}+53x^{11}-53x^{12}+30x^{13} \\
& -14x^{14}+x^{15}) \\
& +q^{33}x^8(-1+4x-x^2+10x^3-13x^4+20x^5-37x^6+36x^7-50x^8+58x^9-49x^{10}+43x^{11}-34x^{12} \\
& +24x^{13}-12x^{14}+x^{15}) \\
& -q^{70}x^{20}(6-9x+17x^2-24x^3+22x^4-22x^5+18x^6-9x^7-4x^8+26x^9-35x^{10}+29x^{11}-26x^{12} \\
& +24x^{13}-8x^{14}+x^{15}) \\
& -q^{56}x^{16}(3-x+11x^2+x^3+6x^4+3x^5-20x^6+26x^7-51x^8+47x^9-65x^{10}+49x^{11}-46x^{12} \\
& +27x^{13}-8x^{14}+x^{15})
\end{aligned}$$



$$\begin{aligned}
& + q^{89} x^{24} (6 - 6x + 14x^2 - 15x^3 + 20x^4 - 32x^5 + 12x^6 - 33x^7 + 27x^8 - 27x^9 + 29x^{10} - 15x^{11} + 29x^{12} \\
& - x^{13} + 4x^{14} + x^{15}) \\
& - q^{96} x^{26} (5 + 15x^2 - 9x^3 + 15x^4 - 24x^5 + 37x^6 - 39x^7 + 34x^8 - 45x^9 + 22x^{10} - 26x^{11} + 17x^{12} \\
& - 12x^{13} + 5x^{14} + x^{15}) \\
& - q^{92} x^{24} (3 + 11x^2 - 7x^3 + 16x^4 - 19x^5 + 32x^6 - 33x^7 + 22x^8 - 37x^9 + 22x^{10} - 31x^{11} + 21x^{12} \\
& - 17x^{13} + 7x^{14} + x^{15}) \\
& + q^{97} x^{27} (-1 + 10x - 8x^2 + 16x^3 - 19x^4 + 37x^5 - 30x^6 + 28x^7 - 43x^8 + 33x^9 - 33x^{10} + 22x^{11} \\
& - 17x^{12} + 12x^{13} - x^{14} + 2x^{15}) \\
& + q^{39} x^{10} (-1 + 4x - x^2 + 11x^3 - 7x^4 + 25x^5 - 28x^6 + 48x^7 - 53x^8 + 63x^9 - 69x^{10} + 59x^{11} - 47x^{12} \\
& + 25x^{13} - 18x^{14} + 4x^{15}) \\
& + q^{68} x^{19} (5 - 7x + 12x^2 - 19x^3 + 17x^4 - 23x^5 + 12x^6 - 9x^7 - 4x^8 + 25x^9 - 31x^{10} + 33x^{11} - 32x^{12} \\
& + 29x^{13} - 10x^{14} + 4x^{15}) \\
& - q^{52} x^{14} (1 + 4x^2 - 2x^3 + x^4 + 5x^5 - 20x^6 + 28x^7 - 44x^8 + 45x^9 - 73x^{10} + 56x^{11} - 62x^{12} + 35x^{13} \\
& - 21x^{14} + 5x^{15}) \\
& + q^{51} x^{14} (1 - x^2 - 3x^3 - 10x^4 + 10x^5 - 21x^6 + 33x^7 - 34x^8 + 61x^9 - 56x^{10} + 62x^{11} - 58x^{12} \\
& + 35x^{13} - 19x^{14} + 6x^{15}) \\
& + q^{82} x^{21} (3 - 2x + 10x^2 - 9x^3 + 6x^4 - 23x^5 + 15x^6 - 19x^7 + 27x^8 - 33x^9 + 21x^{10} - 28x^{11} + 4x^{12} \\
& + 10x^{13} - 10x^{14} + 7x^{15} - 8x^{16}) \\
& + q^{67} x^{18} (2 - 6x + 6x^2 - 22x^3 + 10x^4 - 24x^5 + 3x^6 - 20x^7 - 8x^8 + 10x^9 - 13x^{10} + 32x^{11} - 32x^{12} \\
& + 35x^{13} - 26x^{14} + 9x^{15} - 6x^{16}) \\
& + q^{72} x^{19} (1 + 6x^2 - 10x^3 + 18x^4 - 26x^5 + 26x^6 - 24x^7 + 23x^8 - 5x^9 - 3x^{10} + 23x^{11} - 32x^{12} \\
& + 26x^{13} - 18x^{14} + 20x^{15} - 5x^{16}) \\
& + q^{47} x^{12} (1 - 5x^2 + x^3 - 9x^4 + 13x^5 - 14x^6 + 33x^7 - 33x^8 + 55x^9 - 60x^{10} + 68x^{11} - 62x^{12} + 55x^{13} \\
& - 30x^{14} + 12x^{15} - 4x^{16}) \\
& + q^{64} x^{17} (2 - 3x + 6x^2 - 11x^3 + 9x^4 - 20x^5 + 4x^6 - 14x^7 - 6x^8 + 19x^9 - 29x^{10} + 42x^{11} - 40x^{12} \\
& + 47x^{13} - 22x^{14} + 16x^{15} - 4x^{16}) \\
& + q^{86} x^{23} (6 - 4x + 17x^2 - 14x^3 + 14x^4 - 28x^5 + 15x^6 - 31x^7 + 26x^8 - 38x^9 + 19x^{10} - 22x^{11} + 6x^{12} \\
& + 4x^{13} - 7x^{14} + 2x^{15} - 3x^{16}) \\
& + q^{91} x^{24} (1 - 7x + 6x^2 - 17x^3 + 13x^4 - 25x^5 + 35x^6 - 17x^7 + 38x^8 - 27x^9 + 27x^{10} - 27x^{11} + 14x^{12} \\
& - 26x^{13} + x^{14} - 3x^{15} - x^{16}) \\
& + q^{49} x^{13} (-1 + 3x^2 + x^3 + 11x^4 - 12x^5 + 16x^6 - 34x^7 + 32x^8 - 59x^9 + 59x^{10} - 65x^{11} + 60x^{12} \\
& - 44x^{13} + 25x^{14} - 8x^{15} + x^{16}) \\
& + q^{87} x^{23} (-4 + 6x - 12x^2 + 14x^3 - 15x^4 + 28x^5 - 11x^6 + 28x^7 - 29x^8 + 24x^9 - 29x^{10} + 18x^{11} - 27x^{12} \\
& - 2x^{13} - 2x^{14} - 2x^{15} + x^{16}) \\
& + q^{94} x^{25} (4 + 13x^2 - 8x^3 + 17x^4 - 21x^5 + 36x^6 - 36x^7 + 29x^8 - 42x^9 + 22x^{10} - 28x^{11} + 18x^{12}
\end{aligned}$$

$$\begin{aligned}
& -16x^{13} + 9x^{14} + x^{15} + x^{16}) \\
& -q^{95}x^{26}(-1 + 9x - 8x^2 + 16x^3 - 17x^4 + 34x^5 - 30x^6 + 25x^7 - 42x^8 + 31x^9 - 33x^{10} + 25x^{11} - 15x^{12} \\
& + 15x^{13} - 2x^{14} + 3x^{15} + x^{16}) \\
& + q^{93}x^{25}(-1 + 8x - 9x^2 + 16x^3 - 12x^4 + 30x^5 - 33x^6 + 23x^7 - 40x^8 + 29x^9 - 29x^{10} + 29x^{11} - 15x^{12} \\
& + 19x^{13} - x^{14} + 4x^{15} + x^{16}) \\
& - q^{71}x^{20}(-4 + 6x - 13x^2 + 24x^3 - 15x^4 + 31x^5 - 12x^6 + 20x^7 + 8x^8 - 10x^9 + 11x^{10} - 24x^{11} + 23x^{12} \\
& - 27x^{13} + 15x^{14} + 2x^{16}) \\
& + q^{60}x^{16}(-1 + 2x - 6x^2 + 4x^3 - 17x^4 + 2x^5 - 10x^6 - 4x^7 + 20x^8 - 25x^9 + 50x^{10} - 47x^{11} + 57x^{12} \\
& - 36x^{13} + 31x^{14} - 12x^{15} + 2x^{16}) \\
& + q^{66}x^{18}(-3 + 5x - 10x^2 + 15x^3 - 12x^4 + 20x^5 - 9x^6 + 11x^7 + 4x^8 - 25x^9 + 31x^{10} - 36x^{11} + 35x^{12} \\
& - 39x^{13} + 19x^{14} - 9x^{15} + 2x^{16}) \\
& + q^{55}x^{15}(-1 + 2x - 2x^2 - 2x^3 - 7x^4 - 7x^5 + 9x^6 - 21x^7 + 31x^8 - 39x^9 + 62x^{10} - 51x^{11} + 51x^{12} \\
& - 47x^{13} + 19x^{14} - 8x^{15} + 2x^{16}) \\
& + q^{63}x^{17}(-4 + x - 13x^2 + 3x^3 - 17x^4 + x^5 - 16x^6 - 7x^7 + 12x^8 - 15x^9 + 27x^{10} - 42x^{11} + 40x^{12} \\
& - 42x^{13} + 21x^{14} - 14x^{15} + 4x^{16}) \\
& + q^{84}x^{22}(-5 + 3x - 12x^2 + 11x^3 - 10x^4 + 25x^5 - 15x^6 + 26x^7 - 26x^8 + 36x^9 - 17x^{10} + 24x^{11} - 5x^{12} \\
& - 6x^{13} + 7x^{14} - 4x^{15} + 4x^{16}) \\
& + q^{69}x^{19}(-3 + 6x - 10x^2 + 23x^3 - 13x^4 + 29x^5 - 7x^6 + 20x^7 + 9x^8 - 9x^9 + 12x^{10} - 29x^{11} + 26x^{12} \\
& - 32x^{13} + 20x^{14} - 4x^{15} + 4x^{16}) \\
& + q^{62}x^{16}(-1 + 2x - 3x^2 + 9x^3 - 6x^4 + 19x^5 - x^6 + 14x^7 + 5x^8 - 21x^9 + 27x^{10} - 48x^{11} + 44x^{12} \\
& - 52x^{13} + 27x^{14} - 24x^{15} + 8x^{16}) \\
& + q^{83}x^{21}(-2 + 6x - 5x^2 + 14x^3 - 7x^4 + 19x^5 - 11x^6 + 20x^7 - 30x^8 + 23x^9 - 32x^{10} + 20x^{11} - 25x^{12} \\
& + 5x^{14} - 3x^{15} + x^{16} - 5x^{17}) \\
& + q^{61}x^{16}(3 + 9x^2 - 2x^3 + 13x^4 + x^5 + 14x^6 + 6x^7 - 12x^8 + 18x^9 - 28x^{10} + 44x^{11} - 45x^{12} + 48x^{13} \\
& - 31x^{14} + 23x^{15} - 6x^{16} + x^{17}) \\
& - q^{59}x^{15}(2 + 5x^2 - x^3 + 9x^4 + x^5 + 11x^6 + 5x^7 - 14x^8 + 17x^9 - 27x^{10} + 44x^{11} - 52x^{12} + 49x^{13} \\
& - 37x^{14} + 30x^{15} - 10x^{16} + 2x^{17}) \\
& - q^{65}x^{17}(1 - 6x + 3x^2 - 16x^3 + 6x^4 - 22x^5 + x^6 - 17x^7 - 6x^8 + 12x^9 - 13x^{10} + 29x^{11} - 38x^{12} \\
& + 36x^{13} - 34x^{14} + 14x^{15} - 9x^{16} + 2x^{17}) \\
& + q^{74}x^{19}(1 - 2x - 8x^3 + 11x^4 - 16x^5 + 26x^6 - 30x^7 + 26x^8 - 26x^9 + 6x^{10} + 7x^{11} - 19x^{12} + 27x^{13} \\
& - 25x^{14} + 11x^{15} - 13x^{16} + 3x^{17}) \\
& + q^{85}x^{22}(3 - 6x + 9x^2 - 14x^3 + 11x^4 - 25x^5 + 11x^6 - 25x^7 + 28x^8 - 23x^9 + 32x^{10} - 21x^{11} + 25x^{12} \\
& + 5x^{13} - x^{14} + 2x^{15} - x^{16} + 3x^{17}) \\
& + q^{57}x^{14}(1 + 2x^2 - x^3 + 5x^4 - x^5 + 7x^6 + 7x^7 - 10x^8 + 20x^9 - 27x^{10} + 42x^{11} - 60x^{12} + 49x^{13} \\
& - 44x^{14} + 37x^{15} - 15x^{16} + 5x^{17})
\end{aligned}$$

$$\begin{aligned}
& + q^{78} x^{19} (1 - x + 3x^2 - 7x^3 + 2x^4 - 14x^5 + 13x^6 - 17x^7 + 28x^8 - 33x^9 + 25x^{10} - 29x^{11} + 6x^{12} + 9x^{13} \\
& - 16x^{14} + 15x^{15} - 15x^{16} + 2x^{17} - 5x^{18}) \\
& + q^{90} x^{23} (2 + 8x^2 - 6x^3 + 16x^4 - 16x^5 + 27x^6 - 32x^7 + 21x^8 - 35x^9 + 21x^{10} - 36x^{11} + 23x^{12} - 19x^{13} \\
& + 4x^{14} - 2x^{16} + x^{17} - x^{18}) \\
& - q^{76} x^{19} (-1 + 2x - 3x^2 + x^3 - 11x^4 + 12x^5 - 15x^6 + 28x^7 - 33x^8 + 25x^9 - 26x^{10} + 4x^{11} + 9x^{12} - 15x^{13} \\
& + 19x^{14} - 22x^{15} + 6x^{16} - 8x^{17} + x^{18}) \\
& + q^{88} x^{22} (-1 - 6x^2 + 5x^3 - 18x^4 + 14x^5 - 21x^6 + 31x^7 - 16x^8 + 33x^9 - 23x^{10} + 38x^{11} - 23x^{12} + 21x^{13} \\
& - 4x^{14} - 3x^{15} + 4x^{16} + 2x^{18}) \\
& - q^{79} x^{20} (-4 + x - 7x^2 + 3x^3 - 12x^4 + 9x^5 - 17x^6 + 29x^7 - 20x^8 + 34x^9 - 19x^{10} + 21x^{11} + 3x^{12} - 7x^{13} \\
& + 6x^{14} - 7x^{15} + 9x^{16} - 2x^{17} + 2x^{18}) \\
& + q^{80} x^{20} (-2 + x - 6x^2 + 8x^3 - 4x^4 + 19x^5 - 14x^6 + 16x^7 - 27x^8 + 34x^9 - 23x^{10} + 30x^{11} - 5x^{12} - 11x^{13} \\
& + 13x^{14} - 10x^{15} + 11x^{16} - 2x^{17} + 2x^{18}) \\
& + q^{77} x^{19} (-3 - 5x^2 + 2x^3 - 9x^4 + 9x^5 - 17x^6 + 26x^7 - 19x^8 + 36x^9 - 21x^{10} + 18x^{11} + 3x^{12} - 8x^{13} \\
& + 10x^{14} - 9x^{15} + 13x^{16} - 7x^{17} + 3x^{18}) \\
& - q^{75} x^{18} (-2 - 2x^2 + x^3 - 7x^4 + 6x^5 - 18x^6 + 27x^7 - 20x^8 + 35x^9 - 16x^{10} + 20x^{11} + 3x^{12} - 7x^{13} \\
& + 15x^{14} - 13x^{15} + 17x^{16} - 12x^{17} + 7x^{18}) \\
& + q^{73} x^{17} (-1 - 6x^4 + 6x^5 - 15x^6 + 27x^7 - 18x^8 + 33x^9 - 13x^{10} + 20x^{11} + 6x^{12} - 8x^{13} + 14x^{14} \\
& - 19x^{15} + 19x^{16} - 17x^{17} + 10x^{18}) \\
& + q^{81} x^{20} (1 - 6x + 2x^2 - 9x^3 + 6x^4 - 15x^5 + 10x^6 - 18x^7 + 31x^8 - 23x^9 + 32x^{10} - 19x^{11} + 22x^{12} + x^{13} \\
& - 7x^{14} + 4x^{15} - 5x^{16} + 7x^{17} + x^{19}) \\
& + q^{169} (x^{54} + 2x^{56} - x^{57})]
\end{aligned}$$

$$\begin{aligned}
h_6 = & q^{448} x^{39} [-1 + (1 + q + q^2 + q^3 + q^4 + q^5 + q^6) x \\
& - q (1 + q + 2q^2 + 2q^3 + 3q^4 + 3q^5 + 3q^6 + 2q^7 + 2q^8 + q^9 + q^{10}) x^2 \\
& + q^3 (1 + q + 2q^2 + 3q^3 + 4q^4 + 4q^5 + 5q^6 + 4q^7 + 4q^8 + 3q^9 + 2q^{10} + q^{11} + q^{12}) x^3 \\
& - q^6 (1 + q + 2q^2 + 3q^3 + 4q^4 + 4q^5 + 5q^6 + 4q^7 + 4q^8 + 3q^9 + 2q^{10} + q^{11} + q^{12}) x^4 \\
& + q^{10} (1 + q + 2q^2 + 2q^3 + 3q^4 + 3q^5 + 3q^6 + 2q^7 + 2q^8 + q^9 + q^{10}) x^5 \\
& - q^{15} (1 + q + q^2 + q^3 + q^4 + q^5 + q^6) x^6 + q^{21} x^7]^2 \times \\
& [-1 + qx^2 + q^2 x^3 + q^{11} x^3 - q^3 x^5 + q^4 x^5 + q^{128} x^{52} + q^{134} x^{52} + q^{129} x^{53} + q^{137} x^{54} \\
& - q^{138} x^{55} - q^{141} x^{55} - q^{142} x^{56} + q^{145} x^{58} - q^6 x^4 (1 + x) + q^{125} x^{48} (-1 + x^2)^2 \\
& - q^{132} x^{51} (-1 + x^2)^2 - q^{135} x^{51} (-1 + x^2)^2 + q^{117} x^{46} (1 + x + x^2 - x^3) \\
& + q^{127} x^{50} (-1 - 2x + x^3) + q^{133} x^{50} (-1 + x^4) - q^{124} x^{49} (2 + x^4) \\
& + q^8 x^3 (1 - x + x^4) + q^{122} x^{48} (3 - 2x^2 + x^4) + q^{126} x^{49} (1 - x - x^2 + x^4)
\end{aligned}$$

$$\begin{aligned}
& + q^{131}x^{50}(-1-x+x^2+x^4) - q^{113}x^{42}(1+x+x^2+x^4) \\
& + q^{121}x^{46}(-1+x+x^2-2x^3+x^4) - q^7x^2(-1+x^3+x^4) - q^{112}x^{45}(1-3x^2+x^3+x^4) \\
& + q^{14}x^8(3+x^2-x^5) + q^{17}x^7(2+2x+x^2+x^3-x^5) + q^{13}x^6(-1+x+x^5) \\
& + q^{130}x^{48}(1-x^2+x^5) + q^9x^5(-1-x^2-x^3+x^5) + q^{120}x^{45}(-1+x+x^2-x^3+x^5) \\
& + q^{119}x^{46}(1+x-2x^2-3x^4+x^5) + q^{10}x^5(-1-x+x^4+x^5) \\
& + q^{123}x^{47}(1+x^2-x^3-x^4+x^6) + q^{12}x^4(-1-2x+x^5+x^6) + q^5(x^2+x^3-x^7) \\
& + q^{105}x^{41}(1+x-x^3+3x^4+x^5-x^7) + q^{18}x^8(1+x^3+x^4-2x^5-x^6-x^7) \\
& - q^{15}x^5(2+x^3-x^4+x^7) + q^{114}x^{43}(-1-x-x^2+2x^3-x^4+x^7) \\
& - q^{16}x^5(1+x-x^2+x^3-x^4-3x^5+x^7) + q^{115}x^{44}(-1+x+x^2+2x^3-x^4-x^5+x^7) \\
& - q^{116}x^{41}(1-x^4+x^8) - q^{110}x^{41}(-1+x^2+2x^3-2x^5+x^6+x^8) \\
& - q^{108}x^{39}(-1+x^2-x^3+x^4+2x^5-x^7+x^8) - q^{19}x^6(1-x^5+x^6+x^7+x^8) \\
& + q^{23}x^9(-1-x^3-2x^4+3x^8) + q^{85}x^{32}(-1+4x+3x^2+x^3+x^4+x^6+2x^7-3x^8-2x^9) \\
& + q^{107}x^{39}(1+x^3-4x^4-x^5+x^6+x^7-x^9) - q^{84}x^{31}(1+x+x^2-x^3-5x^4-2x^5+2x^6+x^9) \\
& + q^{21}x^7(1+x+2x^2-2x^5-x^7+x^9) + q^{47}x^{18}(-1+2x+5x^2+4x^3-4x^4-2x^5-4x^6-x^7-6x^8+x^9) \\
& + q^{89}x^{33}(3+3x+2x^2-x^3-x^4-6x^5-2x^6+4x^7-6x^8+x^9) \\
& - q^{80}x^{31}(3+x^2-4x^3+x^6-3x^7-3x^8+x^9) + q^{95}x^{35}(1-x^2+3x^3-4x^4+x^6-x^8+x^9) \\
& - q^{103}x^{38}(-2-x-x^2+x^4+x^5-2x^6-2x^7+x^8+x^9) - q^{20}x^5(1-2x^3-x^5-x^6+x^7+2x^8+x^9) \\
& + q^{24}x^9(2+2x+x^2-x^3-2x^4-x^5+2x^6-x^7+2x^9) \\
& + q^{98}x^{36}(-3-x+x^2+3x^3+x^4+x^5-4x^6+x^7+2x^9) \\
& - q^{111}x^{39}(-1+x^2+x^3+x^5-2x^6-5x^7+3x^9) + q^{92}x^{34}(2+x-x^2+x^3-5x^4-x^6-2x^7-2x^8+4x^9) \\
& + q^{27}x^{10}(-3-x-x^3+2x^4+x^5+2x^6+x^7+2x^8+x^9-3x^{10}) \\
& + q^{79}x^{30}(-3-x-2x^2+x^3-5x^4+6x^5-3x^6+2x^7+5x^8+2x^9-2x^{10}) \\
& + q^{37}x^{15}(4+2x-2x^2+x^3-5x^5-x^6+3x^7+2x^8+3x^9-x^{10}) \\
& + q^{102}x^{36}(-1-x+x^3+x^4+4x^5-2x^6-3x^7-2x^8+x^{10}) \\
& + q^{88}x^{33}(5+2x-4x^2-x^3+2x^4-x^5+2x^6-2x^7-2x^8+x^{10}) \\
& + q^{101}x^{36}(-2-x+x^2-x^3+x^4+3x^5-5x^7+x^8+x^{10}) \\
& - q^{97}x^{34}(-1+x^2+4x^4+2x^5-3x^6-2x^7-3x^8+x^9+x^{10}) \\
& - q^{109}x^{38}(-1-x+2x^4+x^5+2x^6-x^8+x^9+x^{10}) \\
& - q^{29}x^{11}(1+2x-3x^3-3x^5-6x^6-x^7+2x^8+x^9+x^{10}) \\
& - q^{90}x^{32}(1-x+x^2+x^3+2x^4+3x^5+x^6-x^7+2x^9+x^{10}) \\
& + q^{100}x^{36}(-1-x-x^2+x^3+3x^4+4x^5+x^6-2x^7+x^8+2x^9+x^{10}) \\
& + q^{22}x^7(1+x-x^3-3x^4-x^5+x^7-4x^8+x^9+2x^{10}) \\
& - q^{82}x^{31}(1+2x+5x^2-4x^5-5x^7+2x^9+2x^{10}) \\
& + q^{106}x^{36}(-1+x^2+2x^4+x^5+x^6-2x^7-2x^8+2x^9+2x^{10}) \\
& - q^{45}x^{17}(1+3x-4x^2-x^3-4x^6+3x^7+2x^8+x^9+4x^{10})
\end{aligned}$$

$$\begin{aligned}
& + q^{73}x^{25}(-2 + 3x^2 + 3x^3 - 3x^5 - 2x^6 + x^7 - 5x^8 + 3x^9 - 5x^{11}) \\
& + q^{31}x^{11}(-1 - 2x^2 + 2x^3 + 5x^4 + x^5 - 4x^6 + x^7 - 4x^9 - 2x^{11}) \\
& + q^{41}x^{16}(-1 - 3x + x^2 + 3x^3 + 2x^4 - 3x^6 - x^7 + x^{10} - 2x^{11}) \\
& + q^{104}x^{37}(-1 + x^2 + x^3 + 2x^4 + x^5 - 3x^6 - 3x^7 + 2x^8 + x^9 - x^{11}) \\
& + q^{32}x^{12}(-1 + x + x^2 + 3x^3 - 3x^4 + 2x^5 + 2x^6 - 2x^8 - 2x^9 + x^{11}) \\
& + q^{93}x^{33}(2 + 2x - 3x^2 - 4x^4 - 2x^5 - 2x^6 + 3x^7 - x^9 + x^{11}) \\
& - q^{91}x^{31}(1 - 3x^3 + 2x^5 + x^6 + 5x^7 + 3x^8 - 2x^9 - 4x^{10} + x^{11}) \\
& - q^{50}x^{17}(1 + x^2 + 3x^3 - 3x^4 + x^5 + x^7 + 7x^8 + 4x^9 - 3x^{10} + x^{11}) \\
& + q^{96}x^{33}(1 + x - 2x^2 - 4x^3 - x^7 + 5x^8 - x^9 - 2x^{10} + x^{11}) \\
& - q^{26}x^8(-1 + x + x^2 + 5x^4 + 2x^5 + x^6 - 2x^7 - x^8 - x^9 - x^{10} + x^{11}) \\
& + q^{99}x^{34}(1 - x - x^3 + 2x^8 + x^{10} + x^{11}) - q^{28}x^8(-1 - x^4 + 2x^6 + x^7 - x^8 - 2x^9 + x^{10} + x^{11}) \\
& - q^{86}x^{31}(3 - 4x - 2x^2 - x^4 - 6x^5 - x^6 + 2x^7 + 2x^8 + x^9 + x^{10} + x^{11}) \\
& - q^{87}x^{31}(1 + x - x^2 - x^3 - 4x^4 - 3x^5 + 4x^6 + x^7 + 2x^9 + x^{10} + x^{11}) \\
& - q^{42}x^{16}(1 + 4x + 3x^2 - x^4 - 4x^6 - 7x^7 + 3x^9 + x^{10} + x^{11}) \\
& + q^{78}x^{28}(5 - 3x^2 - 5x^3 + x^4 - 2x^5 + 2x^7 + x^8 - x^9 + 3x^{10} + x^{11}) \\
& + q^{39}x^{14}(1 + x - x^2 - 5x^4 + 2x^5 - 2x^7 + 2x^8 + 5x^9 + x^{10} + 2x^{11}) \\
& + q^{38}x^{14}(1 + x + x^2 - x^3 - 3x^4 - 2x^5 + x^6 + x^7 + 5x^8 + 3x^{10} + 2x^{11}) \\
& - q^{83}x^{30}(5 + 3x - 3x^2 - 6x^3 - 4x^4 - 3x^5 + x^6 + x^7 + x^8 - 5x^9 - x^{10} + 3x^{11}) \\
& + q^{68}x^{24}(-2 - 5x - 3x^2 + 5x^3 + 3x^4 - 4x^6 + x^8 - 3x^9 - 2x^{12}) \\
& + q^{60}x^{21}(1 + x^2 - 3x^3 + x^4 + 3x^5 + 4x^6 - 5x^9 - 3x^{10} + x^{11} - 2x^{12}) \\
& + q^{25}x^7(1 + x + x^3 - 2x^4 - 2x^5 - 3x^6 - x^7 + x^8 + x^9 + 2x^{10} + x^{11} - x^{12}) \\
& + q^{33}x^{11}(-1 + 2x^3 + x^4 + 4x^5 + 2x^7 - 5x^8 - 3x^9 + 2x^{11} - x^{12}) \\
& + q^{52}x^{19}(-1 + 4x - x^2 - 3x^3 + x^5 - x^6 + x^7 + x^8 + 3x^9 + x^{12}) \\
& + q^{54}x^{19}(-1 + x^2 + x^3 - 5x^4 + 5x^5 + 6x^6 + 2x^7 + 6x^8 + 3x^9 - 2x^{11} + x^{12}) \\
& - q^{77}x^{27}(-1 - 4x^4 + x^5 + 2x^6 + x^7 - 2x^8 + 4x^9 - x^{10} - 2x^{11} + x^{12}) \\
& + q^{30}x^{10}(-1 - x - x^2 + x^4 + 2x^5 + 2x^7 + 3x^8 - 3x^9 - 3x^{10} - x^{11} + x^{12}) \\
& + q^{70}x^{25}(-1 + x + 3x^2 + 4x^3 - x^5 - 4x^6 - x^7 + 7x^8 + 3x^9 - 5x^{10} + x^{11} + x^{12}) \\
& + q^{94}x^{33}(1 - x^3 - x^4 - x^5 - x^6 + 5x^7 + 3x^8 - 3x^9 - 2x^{10} + x^{11} + x^{12}) \\
& + q^{34}x^{12}(-1 + x + 2x^2 + 3x^3 - 2x^4 - 3x^5 - 4x^6 - 5x^8 - x^9 + 3x^{10} + x^{11} + x^{12}) \\
& + q^{53}x^{19}(-1 - x + 4x^2 + x^3 - 3x^4 + 5x^6 - x^7 + 4x^8 + 4x^{11} + x^{12}) \\
& + q^{55}x^{20}(1 + x + 2x^2 - x^3 - 4x^4 - 2x^5 + x^6 + 4x^7 + 5x^8 + x^{10} + 4x^{11} + x^{12}) \\
& + q^{49}x^{18}(-1 + x^2 + x^3 - 2x^4 - 6x^5 - 3x^6 - 3x^7 + 2x^8 + 2x^{10} + 2x^{12}) \\
& - q^{46}x^{16}(-1 + x + x^2 - 5x^4 + x^5 + x^6 - 3x^8 + x^{10} + 3x^{11} + 4x^{12}) \\
& + q^{44}x^{15}(1 + 2x - 2x^2 + x^4 + 6x^5 + 2x^6 + 3x^7 - 3x^8 + 2x^9 - 5x^{10} - 5x^{11} - x^{12} - 2x^{13}) \\
& + q^{81}x^{27}(1 - 4x^3 - 3x^4 + x^6 - x^7 + x^8 + x^9 - x^{11} - x^{13})
\end{aligned}$$

$$\begin{aligned}
& + q^{40} x^{13} (1 + x + x^2 - x^3 - 4x^4 - x^6 - x^7 + x^8 + 5x^9 + 5x^{10} + 2x^{12} - x^{13}) \\
& + q^{61} x^{19} (-1 - x + x^2 + 4x^3 - x^6 + 4x^7 - 4x^8 - x^{11} + x^{13}) \\
& + q^{36} x^{12} (1 - x + x^2 + 2x^3 - 5x^5 - 2x^6 + 2x^7 + x^8 + x^9 - x^{10} + 2x^{11} + x^{13}) \\
& + q^{63} x^{22} (3 + 3x - 2x^2 - 6x^3 - x^4 + 2x^5 + 4x^6 + 9x^8 - 4x^9 - 3x^{10} - 3x^{12} + x^{13}) \\
& + q^{75} x^{26} (1 - 4x^4 + 2x^5 - 3x^6 + 2x^7 + x^8 - 4x^9 - 5x^{10} + 4x^{11} + 3x^{12} + x^{13}) \\
& - q^{67} x^{22} (-1 + 2x^2 + x^3 - 2x^4 + 4x^5 + 3x^6 - 4x^8 - 3x^9 + x^{10} - x^{11} + 2x^{13}) \\
& + q^{35} x^{10} (-1 - x^2 - x^3 + 2x^4 - x^6 - x^7 - 2x^9 - 3x^{10} - 4x^{11} - x^{12} + 3x^{13}) \\
& + q^{65} x^{22} (1 - x + x^2 - 4x^3 - 2x^5 + x^6 - 4x^9 + 4x^{10} + 2x^{11} - 3x^{13} - x^{14}) \\
& + q^{48} x^{16} (1 + x - x^2 - 3x^3 + 2x^4 - 2x^5 + x^6 - 2x^7 - 3x^8 + 3x^9 + 3x^{10} - 4x^{11} - 4x^{12} + x^{14}) \\
& + q^{69} x^{23} (1 - 3x^2 + x^3 + x^4 - 2x^5 + 8x^7 + 2x^8 - 2x^9 + 3x^{10} - 2x^{11} - 5x^{12} - 3x^{13} + x^{14}) \\
& - q^{43} x^{14} (1 - x + x^2 + x^4 - 2x^5 - x^6 - x^7 + x^8 + x^{13} + x^{14}) \\
& + q^{71} x^{22} (1 - x^2 - 4x^4 + 3x^5 + 2x^6 + 4x^8 + 4x^9 + x^{11} - 3x^{12} + x^{13} + x^{14}) \\
& + q^{74} x^{24} (-1 - x + x^3 + 3x^4 + 2x^6 + x^7 - 2x^8 - 6x^9 + 3x^{10} + 3x^{11} - 2x^{12} + x^{13} + x^{14}) \\
& + q^{57} x^{19} (-1 + x^3 - 4x^4 + 2x^6 + 3x^7 - 3x^8 + 5x^9 - 3x^{11} - x^{12} + x^{13} + x^{14}) \\
& - q^{62} x^{21} (-1 - x + x^2 + x^3 - 5x^4 - x^5 + x^6 + 4x^7 + 5x^9 + x^{10} - 6x^{11} - 3x^{12} + 3x^{13} + x^{14}) \\
& + q^{76} x^{25} (-1 + 3x^2 + 4x^3 - 2x^5 - 4x^6 - 4x^7 - 5x^8 + 3x^{11} - x^{12} + 4x^{13} + x^{14}) \\
& - q^{58} x^{19} (1 + 2x - x^2 - 4x^4 + 4x^5 - 2x^6 + x^7 + 9x^9 - 4x^{12} + 2x^{14}) \\
& + q^{66} x^{22} (2 + 2x - 3x^2 - 2x^3 + 4x^5 - 4x^6 + 8x^9 - 3x^{10} - 2x^{13} + 2x^{14}) \\
& + q^{51} x^{17} (1 - 2x + x^2 + x^4 - 6x^5 - x^6 - x^8 + 3x^9 - 3x^{11} + 4x^{13} + 2x^{14}) \\
& + q^{72} x^{24} (-1 + x^2 + x^3 + 3x^6 + x^7 - 3x^8 + x^9 + 4x^{10} - 7x^{11} - 3x^{12} + 2x^{13} + 3x^{14}) \\
& - q^{64} x^{20} (1 - x + 3x^4 - x^5 - 2x^6 + x^7 + 8x^8 - 2x^{10} + 6x^{11} + 2x^{12} - 5x^{13} + x^{14} + x^{15}) \\
& - q^{59} x^{19} (1 - x^2 - x^3 + 2x^4 + x^5 + x^6 - 2x^7 + 2x^8 + 2x^9 + 3x^{11} - 5x^{13} + 2x^{14} + x^{15}) \\
& - q^{56} x^{17} (-1 + x^3 - 2x^5 + x^6 - x^7 - 5x^8 + 8x^{10} - x^{11} - 3x^{13} - 3x^{14} + x^{15} + x^{16}) \\
& + q^{118} (x^{44} - x^{51}) + q^{136} (x^{53} - x^{56}) + q^{140} (x^{53} - x^{56})]
\end{aligned}$$

$$\begin{aligned}
b_0 = & q^{40} x^3 [-1 + (1 + q + q^2 + q^3 + q^4) x - q (1 + q + 2q^2 + 2q^3 + 2q^4 + q^5 + q^6) x^2 \\
& + q^3 (1 + q + 2q^2 + 2q^3 + 2q^4 + q^5 + q^6) x^3 - q^6 (1 + q + q^2 + q^3 + q^4) x^4 + q^{10} x^5]^2 \times \\
& [1 - q^2 x - q^3 x^2 - q^5 x^2 - 2q^7 x^2 + q^9 x^3 + q^{10} (-1 + x) x^3 + q^8 x^4 + q^{14} x^4 + q^{11} x^5 + q^{17} x^5 \\
& - q^{15} (-1 + x) x^5 + q^{16} x^6 - 2q^{18} x^7 - q^{20} x^7 - q^{22} x^7 - q^{23} x^8 + q^{25} x^9 - q^6 x^2 (1 + x) \\
& - q^{19} x^6 (1 + x) + q^{12} x^4 (2 + x) + q^{13} x^4 (1 + 2x)]
\end{aligned}$$

$$\begin{aligned}
b_1 = & q^{38} [-1 + (1 + q + q^2 + q^3 + q^4) x - q (1 + q + 2q^2 + 2q^3 + 2q^4 + q^5 + q^6) x^2 \\
& + q^3 (1 + q + 2q^2 + 2q^3 + 2q^4 + q^5 + q^6) x^3 - q^6 (1 + q + q^2 + q^3 + q^4) x^4 + q^{10} x^5]^2 \times
\end{aligned}$$

$$\begin{aligned}
& [1 - qx^2 + q^3x^3 + q^4(-1+x)x^3 - q^{25}(-1+x)x^{11} + q^{26}x^{12} - q^{28}x^{13} + q^{29}x^{15} + q^8x^4(2+x^2) \\
& - q^2(x+x^3) - q^{24}x^{10}(-3+x^2+x^3) - q^{11}x^5(-3+x^2+2x^3) + q^{18}x^7(-2-x+3x^3) \\
& + q^5x^2(-1-x+3x^3) + q^{20}x^8(2+x+2x^2-x^3+x^4) + q^9x^3(1-x+2x^2+x^3+2x^4) \\
& - q^6x^2(1+x-2x^2-2x^3-x^4+x^5) + q^{16}x^6(2-2x-3x^2-4x^3+x^4+x^5) \\
& - q^{23}x^8(1-x-2x^2-2x^3+x^4+x^5) + q^{13}x^4(1+x-4x^2-3x^3-2x^4+2x^5) \\
& + q^{12}x^4(2+2x+x^2-5x^3+x^5+x^6) - q^7x^2(2-x^2-2x^3+x^4+x^5+x^6) \\
& - q^{10}x^3(1+x+x^2-2x^3+x^4+x^5+x^6) - q^{19}x^6(1+x+x^2-2x^3+x^4+x^5+x^6) \\
& - q^{22}x^7(1+x+x^2-2x^3-x^4+2x^6) + q^{17}x^5(1+x-5x^3+x^4+2x^5+2x^6) \\
& + q^{14}(x^4-x^6-3x^7+x^8+x^{10}) + q^{15}(x^5+x^7-3x^8-x^9+x^{11}) \\
& + q^{21}(x^9+2x^{11}) - q^{27}(x^{12}+x^{14})]
\end{aligned}$$

$$\begin{aligned}
b_2 = & -q^{37}(1+q)[-1+(1+q+q^2+q^3+q^4)x - q(1+q+2q^2+2q^3+2q^4+q^5+q^6)x^2 \\
& + q^3(1+q+2q^2+2q^3+2q^4+q^5+q^6)x^3 - q^6(1+q+q^2+q^3+q^4)x^4 + q^{10}x^5]^2 \times \\
& [1 - 2qx^2 - 2q^{29}x^{13} + q^{30}x^{15} - q^{28}x^{11}(-1+x+x^3) + q^3x^2(-1+2x+x^3) \\
& - q^4x^2(-1+x-2x^2+x^3) + q^2x(-1-x^2+x^3) + q^{26}x^{10}(-1+2x-x^2+x^3) \\
& + q^{23}x^9(1+3x-2x^4) + q^{24}x^8(-1+x+x^3-2x^4) + q^6x^3(-2+x+x^3-x^4) \\
& - q^{25}x^9(1-2x+2x^2+x^4) + q^7x^2(-2+3x^3+x^4) - q^{11}x^4(2-2x+2x^2+x^5) \\
& - q^{10}x^3(1-x+3x^2+x^5) + q^{12}x^4(2+3x^2-2x^3+x^5) + 2q^9(x^3+x^5) \\
& - q^{22}x^7(1+x-3x^4+x^5) - q^{20}x^7(1+3x^3-x^4+x^5) - q^8x^3(1-3x+x^4+x^5) \\
& + q^{13}x^5(3-2x+x^4+x^5) - q^{19}x^6(1+2x^3-2x^4+2x^5) + q^{17}x^5(1+x-2x^4+3x^5) \\
& + q^{16}x^5(-1-2x^2-4x^3+x^6) - q^{14}x^4(-1+4x^3+2x^4+x^6) - q^5(x^2+2x^4-2x^5+x^6) \\
& + 2q^{15}(x^5+x^{10}) + q^{18}(x^6-2x^8+3x^9+2x^{11}) + 2q^{21}(x^{10}+x^{12}) \\
& + q^{27}(x^{10}+2x^{12}-x^{13})]
\end{aligned}$$

$$\begin{aligned}
b_3 = & q^{37}[-1+(1+q+q^2+q^3+q^4)x - q(1+q+2q^2+2q^3+2q^4+q^5+q^6)x^2 \\
& + q^3(1+q+2q^2+2q^3+2q^4+q^5+q^6)x^3 - q^6(1+q+q^2+q^3+q^4)x^4 + q^{10}x^5]^2 \times \\
& [1 - 2qx^2 + 2q^4x^4 + 2q^{11}(1-2x)x^5 - q^5(-1+x)x^5 + 2q^{20}(-2+x)x^9 + q^{26}(-1+x)x^9 + 2q^{27}x^{11} \\
& - 2q^{30}x^{13} + q^{31}x^{15} + q^{28}x^{10}(1+x+x^2-x^3) + q^{23}x^9(2+2x+2x^2-x^3) \\
& + q^2x(-1-x-x^2+x^3) + q^3x^2(-1+x+x^2+x^3) - q^{29}x^{11}(-1+x+x^2+x^3) \\
& + q^8x^3(-1+2x+2x^2+2x^3) - q^6x^3(1+x+x^4) + q^{19}x^7(2-2x+x^2+x^4) \\
& + q^{15}x^5(3+x-3x^2-5x^3+x^4) + q^{13}x^5(2+x^2-x^3+x^4) - q^{25}x^8(1+x^3+x^4) \\
& + q^7x^2(-1-x-x^2+x^3+x^4) - q^{24}x^9(-1-x+x^2+x^3+x^4) - q^{14}x^5(-2-2x+3x^2+x^3+x^4)
\end{aligned}$$

$$\begin{aligned}
& + q^{18}x^6(1-x+x^2+2x^4) + q^{17}x^6(-1-x-3x^2+2x^3+2x^4) + q^{16}x^6(1-5x-3x^2+x^3+3x^4) \\
& - q^{21}x^7(1+2x+x^2+x^3-2x^4+x^5) + q^{22}x^7(-1-x+3x^3+x^4+x^5) \\
& - q^{10}x^3(1-2x+x^2+x^3+2x^4+x^5) + q^9(x^3+x^4+3x^5-x^7-x^8) + q^{12}(x^4+x^6-2x^7+2x^8)
\end{aligned}$$

$$\begin{aligned}
b_4 = & q^{47}x^3[-1 + (1+q+q^2+q^3+q^4)x - q(1+q+2q^2+2q^3+2q^4+q^5+q^6)x^2 \\
& + q^3(1+q+2q^2+2q^3+2q^4+q^5+q^6)x^3 - q^6(1+q+q^2+q^3+q^4)x^4 + q^{10}x^5]^2 \times \\
& [1 - 2qx^2 + 2q^4x^4 + 2q^7x^5 - 2q^{10}x^7 + q^{11}x^9 + q^2x(-1-x-x^2+x^3) + q^3x^2(-1+x+x^2+x^3) \\
& - q^9x^5(-1+x+x^2+x^3) - q^6x^3(1-x+x^4) - q^5(x^2-x^5+x^6) + q^8(x^4+x^5+x^6-x^7)]
\end{aligned}$$

## References

- [1] Chae J., A Connect Sum Formula for the BPS Invariant of Knot Complements, arXiv September 2021
